# Supplementary material for: Geometric realizations of the Lie superalgebra D(2,1;a)
Source: arXiv:2507.03418 ancillary file (2025-07-04)
Supplement: Supplementary file 1 [file D21alpha_p123i.pdf]

In this worksheet we compute  $G/P_{\{123\}}^I$  realization of LSA  $D(2,1;a)$

- > *interface*(warnlevel = 0) : with(Physics) :
- > Setup(anticommutativeprefix = {seq(y||i, i = 1..4)}, anticommutativecolor = maroon)  
[anticommutativecolor = maroon, anticommutativeprefix = {y1, y2, y3, y4}]

(1)

Realization of the GNLSA (one parameter unremovable but perhaps inessential)

- >  $U1 := f \rightarrow \text{diff}(f, x1) + y1 \text{diff}(f, y2) + k y1 y3 \text{diff}(f, x3) + y1 x2 \text{diff}(f, y4) :$   
 $U2 := f \rightarrow \text{diff}(f, x2) + y1 \text{diff}(f, y3) + y1 y2 \text{diff}(f, x3) + y1 x1 \text{diff}(f, y4) :$   
 $U3 := f \rightarrow (1 + k) \text{diff}(f, x3) :$
- >  $V1 := f \rightarrow -\text{diff}(f, y1) :$   
 $V2 := f \rightarrow \text{diff}(f, y2) + k y3 \text{diff}(f, x3) + x2 \text{diff}(f, y4) :$   
 $V3 := f \rightarrow \text{diff}(f, y3) + y2 \text{diff}(f, x3) + x1 \text{diff}(f, y4) :$   
 $V4 := f \rightarrow \text{diff}(f, y4) + (1 + k) y1 \text{diff}(f, x3) :$
- > var := [x1, x2, x3, y1, y2, y3, y4] :
- > {seq(U1(U2(var[j])) - U2(U1(var[j])), j = 1..7), seq(U1(U3(var[j])) - U3(U1(var[j])), j = 1..7), seq(U2(U3(var[j])) - U3(U2(var[j])), j = 1..7)}

(2)

- > simplify({seq(U1(V1(var[j])) - V1(U1(var[j])) - V2(var[j]), j = 1..7), seq(U2(V1(var[j])) - V1(U2(var[j])) - V3(var[j]), j = 1..7), seq(U3(V1(var[j])) - V1(U3(var[j])), j = 1..7), seq(U1(V2(var[j])) - V2(U1(var[j])), j = 1..7), seq(U2(V2(var[j])) - V2(U2(var[j])) - V4(var[j]), j = 1..7), seq(U3(V2(var[j])) - V2(U3(var[j])), j = 1..7), seq(U1(V3(var[j])) - V3(U1(var[j])) - V4(var[j]), j = 1..7), seq(U2(V3(var[j])) - V3(U2(var[j])), j = 1..7), seq(U3(V3(var[j])) - V3(U3(var[j])), j = 1..7), seq(U1(V4(var[j])) - V4(U1(var[j])), j = 1..7), seq(U2(V4(var[j])) - V4(U2(var[j])), j = 1..7), seq(U3(V4(var[j])) - V4(U3(var[j])), j = 1..7)})

(3)

- > simplify({seq(V1(V1(var[j])), j = 1..7), seq(V1(V2(var[j])) + V2(V1(var[j])), j = 1..7), seq(V1(V3(var[j])) + V3(V1(var[j])), j = 1..7), seq(V1(V4(var[j])) + V4(V1(var[j])) + U3(var[j]), j = 1..7), seq(V2(V2(var[j])), j = 1..7), seq(V2(V3(var[j])) + V3(V2(var[j])) - U3(var[j]), j = 1..7), seq(V2(V4(var[j])) + V4(V2(var[j])), j = 1..7), seq(V3(V3(var[j])), j = 1..7), seq(V3(V4(var[j])) + V4(V3(var[j])), j = 1..7), seq(V4(V4(var[j])), j = 1..7)})

(4)

- > #` [U1, V1] = V2, [U2, V1] = V3, [U2, V2] = V4, [U1, V3] = V4, [V1, V4] = -U3, [V2, V3] = U3

Computing g[0] of dimension (3|0) uniquely

- >  $U01 := f \rightarrow x1 \text{diff}(f, x1) + y2 \text{diff}(f, y2) + y4 \text{diff}(f, y4) + x3 \text{diff}(f, x3) :$   
 $U02 := f \rightarrow x2 \text{diff}(f, x2) + y3 \text{diff}(f, y3) + y4 \text{diff}(f, y4) + x3 \text{diff}(f, x3) :$   
 $U03 := f \rightarrow y1 \text{diff}(f, y1) + y2 \text{diff}(f, y2) + y3 \text{diff}(f, y3) + y4 \text{diff}(f, y4) + 2 x3 \text{diff}(f, x3) :$   
 $Z := f \rightarrow U01(f) + U02(f) + U03(f) :$
- > simplify({seq(U01(U1(var[j])) - U1(U01(var[j])) + U1(var[j]), j = 1..7), seq(U01(U2(var[j])) - U2(U01(var[j])), j = 1..7), seq(U01(V1(var[j])) - V1(U01(var[j])), j = 1..7),

$$\begin{aligned}
& seq(U02(U1(var[j])) - U1(U02(var[j])), j = 1..7), seq(U02(U2(var[j])) \\
& \quad - U2(U02(var[j])) + U2(var[j]), j = 1..7), seq(U02(V1(var[j])) \\
& \quad - V1(U02(var[j])), j = 1..7), \\
& seq(U03(U1(var[j])) - U1(U03(var[j])), j = 1..7), seq(U03(U2(var[j])) \\
& \quad - U2(U03(var[j])), j = 1..7), seq(U03(V1(var[j])) - V1(U03(var[j])) \\
& \quad + V1(var[j]), j = 1..7) \} \\
& \{0\} \tag{5}
\end{aligned}$$

$$\begin{aligned}
> simplify(\{seq(Z(U1(var[j])) - U1(Z(var[j])) + U1(var[j]), j = 1..7), \\
seq(Z(U2(var[j])) - U2(Z(var[j])) + U2(var[j]), j = 1..7), seq(Z(U3(var[j])) \\
- U3(Z(var[j])) + 4 U3(var[j]), j = 1..7), seq(Z(V1(var[j])) - V1(Z(var[j])) \\
+ V1(var[j]), j = 1..7), seq(Z(V2(var[j])) - V2(Z(var[j])) + 2 V2(var[j]), j = 1 \\
..7), seq(Z(V3(var[j])) - V3(Z(var[j])) + 2 V3(var[j]), j = 1..7), seq(Z(V4(var[j])) \\
- V4(Z(var[j])) + 3 V4(var[j]), j = 1..7) \} \\
\{0\} \tag{6}
\end{aligned}$$

Computing pr\_1(g[0]) of dim=(2|2) with one dimensional freedom in odd part for reduction to g[1] of dim=(2|1)

$$\begin{aligned}
> Um := f \rightarrow (c1 x1^2 + c2 x1 x2 + c3 x2^2) diff(f, x1) + (c4 x1^2 + c5 x1 x2 + c6 x2^2) diff(f, x2) \\
+ (c7 x1 y1 + c8 x2 y1 + c9 y2 + c10 y3) diff(f, y1) + (c11 x1^2 y1 + c12 x1 x2 y1 \\
+ c13 x2^2 y1 + c14 x1 y2 + c15 x2 y2 + c16 x1 y3 + c17 x2 y3 + c18 y4) diff(f, y2) \\
+ (c19 x1^2 y1 + c20 x1 x2 y1 + c21 x2^2 y1 + c22 x1 y2 + c23 x2 y2 + c24 x1 y3 \\
+ c25 x2 y3 + c26 y4) diff(f, y3) + (c27 x1^3 y1 + c28 x1^2 x2 y1 + c29 x1 x2^2 y1 \\
+ c30 x2^3 y1 + c31 x1^2 y2 + c32 x1 x2 y2 + c33 x2^2 y2 + c34 x1^2 y3 + c35 x1 x2 y3 \\
+ c36 x2^2 y3 + c37 x1 y4 + c38 x2 y4) diff(f, y4) + (c39 x1^5 + c40 x1^4 x2 + c41 x1^3 x2^2 \\
+ c42 x1^2 x2^3 + c43 x1 x2^4 + c44 x2^5 + c45 x1^2 y1 y2 + c46 x1 x2 y1 y2 + c47 x2^2 y1 y2 \\
+ c48 x1^2 y1 y3 + c49 x1 x2 y1 y3 + c50 x2^2 y1 y3 + c51 x1 y1 y4 + c52 x2 y1 y4 \\
+ c53 x1 y2 y3 + c54 x2 y2 y3 + c55 y2 y4 + c56 y3 y4 + c57 x1 x3 + c58 x2 x3) diff(f, \\
x3) :
\end{aligned}$$

$$\begin{aligned}
> Vm := f \rightarrow (c1 x1 y1 + c2 x2 y1 + c3 y2 + c4 y3) diff(f, x1) + (c5 x1 y1 + c6 x2 y1 + c7 y2 \\
+ c8 y3) diff(f, x2) + (c9 x1^2 + c10 x1 x2 + c11 x2^2) diff(f, y1) + (c12 x1^3 + c13 x1^2 x2 \\
+ c14 x1 x2^2 + c15 x2^3 + c16 y1 y2 + c17 y1 y3) diff(f, y2) + (c18 x1^3 + c19 x1^2 x2 \\
+ c20 x1 x2^2 + c21 x2^3 + c22 y1 y2 + c23 y1 y3) diff(f, y3) + (c24 x1^4 + c25 x1^3 x2 \\
+ c26 x1^2 x2^2 + c27 x1 x2^3 + c28 x2^4 + c29 x1 y1 y2 + c30 x2 y1 y2 + c31 x1 y1 y3 \\
+ c32 x2 y1 y3 + c33 y2 y3 + c34 y1 y4 + c35 x3) diff(f, y4) + (c36 x1^4 y1 \\
+ c37 x1^3 x2 y1 + c38 x1^2 x2^2 y1 + c39 x1 x2^3 y1 + c40 x2^4 y1 + c41 x1^3 y2 + c42 x1^2 x2 y2 \\
+ c43 x1 x2^2 y2 + c44 x2^3 y2 + c45 x1^3 y3 + c46 x1^2 x2 y3 + c47 x1 x2^2 y3 + c48 x2^3 y3 \\
+ c49 x1^2 y4 + c50 x1 x2 y4 + c51 x2^2 y4 + c52 y1 y2 y3 + c53 x3 y1) diff(f, x3) :
\end{aligned}$$

$$\begin{aligned}
> simplify(\{seq(Z(Um(var[j])) - Um(Z(var[j])) - Um(var[j]), j = 1..7), \\
seq(Z(Vm(var[j])) - Vm(Z(var[j])) - Vm(var[j]), j = 1..7) \} \\
\{0\} \tag{7}
\end{aligned}$$

$$\begin{aligned}
> simplify(\{seq(V1(Um(var[j])) - Um(V1(var[j])), j = 1..7) \} \\
\{0, (c47 y2 + c50 y3) x2^2 + ((c46 y2 + c49 y3) x1 + c52 y4) x2 + x1 ((c45 y2 + c48 y3) x1 \\
+ c51 y4), c7 x1 + c8 x2, c11 x1^2 + c12 x1 x2 + c13 x2^2, c19 x1^2 + c20 x1 x2 + c21 x2^2, \\
c27 x1^3 + c28 x1^2 x2 + c29 x1 x2^2 + c30 x2^3\} \\
\tag{8}
\end{aligned}$$

$$\begin{aligned}
& \text{simplify}(\{seq(VI(Vm(var[j]))) + Vm(VI(var[j])) - r1 U01(var[j]) - r2 U02(var[j]) \\
& \quad - r3 U03(var[j]), j=1..7)\}) \\
& \{ -r3 y1, (c1 - r1) x1 + c2 x2, (c6 - r2) x2 + c5 x1, (-r1 - r3 + c16) y2 + c17 y3, (-r2 \\
& \quad - r3 + c23) y3 + c22 y2, (-r1 + c34 - r2 - r3) y4 + (c29 y2 + c31 y3) x1 + x2 (c30 y2 \\
& \quad + c32 y3), c52 y2 y3 + c36 x1^4 + c37 x1^3 x2 + c38 x1^2 x2^2 + c39 x1 x2^3 + c40 x2^4 - x3 (r1 \\
& \quad - c53 + r2 + 2 r3) \}
\end{aligned} \tag{9}$$

$$\begin{aligned}
& \text{Um} := f \rightarrow c1 x1^2 \text{diff}(f, x1) + c6 x2^2 \text{diff}(f, x2) - (c1 y2 + c6 y3) \text{diff}(f, y1) - c6 (x2 y2 \\
& \quad + x1 y3 - y4) \text{diff}(f, y2) - c1 (x2 y2 + x1 y3 - y4) \text{diff}(f, y3) + (-c1 x1 x2 y2 \\
& \quad - c6 x1 x2 y3 + c1 x1 y4 + c6 x2 y4) \text{diff}(f, y4) + (-k c1 x1 y2 y3 + c6 x2 y2 y3 \\
& \quad + k c1 y2 y4 + c6 y3 y4) \text{diff}(f, x3) : \\
& \text{simplify}(\{seq(VI(Um(var[j]))) - Um(VI(var[j])), j=1..7), seq(U1(Um(var[j]))) \\
& \quad - Um(U1(var[j])) - 2 c1 U01(var[j]) + c1 U03(var[j]), j=1..7), \\
& \quad seq(U2(Um(var[j]))) - Um(U2(var[j])) - 2 c6 U02(var[j]) + c6 U03(var[j]), j=1 \\
& \quad ..7)\}) \\
& \{0\}
\end{aligned} \tag{10}$$

$$\begin{aligned}
& \text{Um1} := f \rightarrow x1^2 \text{diff}(f, x1) - y2 \text{diff}(f, y1) - (x2 y2 + x1 y3 - y4) \text{diff}(f, y3) - x1 (x2 y2 \\
& \quad - y4) \text{diff}(f, y4) - k y2 (x1 y3 - y4) \text{diff}(f, x3) : \text{simplify}(\{seq(VI(Um1(var[j]))) \\
& \quad - Um1(VI(var[j])), j=1..7), seq(U1(Um1(var[j]))) - Um1(U1(var[j])) \\
& \quad - 2 U01(var[j]) + U03(var[j]), j=1..7), seq(U2(Um1(var[j]))) \\
& \quad - Um1(U2(var[j])), j=1..7)\}) \\
& \{0\}
\end{aligned} \tag{11}$$

$$\begin{aligned}
& \text{Um2} := f \rightarrow x2^2 \text{diff}(f, x2) - y3 \text{diff}(f, y1) - (x2 y2 + x1 y3 - y4) \text{diff}(f, y2) - x2 (x1 y3 \\
& \quad - y4) \text{diff}(f, y4) - y3 (x2 y2 - y4) \text{diff}(f, x3) : \text{simplify}(\{seq(VI(Um2(var[j]))) \\
& \quad - Um2(VI(var[j])), j=1..7), seq(U1(Um2(var[j]))) - Um2(U1(var[j])), j=1..7), \\
& \quad seq(U2(Um2(var[j]))) - Um2(U2(var[j])) - 2 U02(var[j]) + U03(var[j]), j=1 \\
& \quad ..7)\}) \\
& \{0\}
\end{aligned} \tag{12}$$

$$\begin{aligned}
& \text{Vm} := f \rightarrow (c1 x1 y1 - c1 y2) \text{diff}(f, x1) + (c6 x2 y1 - c6 y3) \text{diff}(f, x2) + c1 y1 y2 \text{diff}(f, y2) \\
& \quad + c6 y1 y3 \text{diff}(f, y3) + (c33 y2 y3 + c34 y1 y4 + c35 x3) \text{diff}(f, y4) + c53 x3 y1 \text{diff}(f, \\
& \quad x3) : \\
& \text{simplify}(\{seq(VI(Vm(var[j]))) + Vm(VI(var[j])) - c1 U01(var[j]) - c6 U02(var[j]), j \\
& \quad = 1..7), seq(U1(Vm(var[j]))) - Vm(U1(var[j])), j=1..7), seq(U2(Vm(var[j]))) \\
& \quad - Vm(U2(var[j])), j=1..7)\}) \\
& \{0, (c35 k + c33 - c6) y1 y3, -x3 (c1 - c53 + c6), -y4 (c1 - c34 + c6), -y1 y2 (c1 + c33 \\
& \quad - c35)\}
\end{aligned} \tag{13}$$

$$\begin{aligned}
& \text{solve}(\{(c35 k + c33 - c6), (c1 - c53 + c6), (c1 - c34 + c6), (c1 + c33 - c35)\}) \\
& \{c1 = c35 k + c35 - c6, c33 = -c35 k + c6, c34 = c35 k + c35, c35 = c35, c53 = c35 k + c35, c6 \\
& \quad = c6, k = k\}
\end{aligned} \tag{14}$$

$$\begin{aligned}
& \text{Vm1a} := f \rightarrow (x1 y1 - y2) \text{diff}(f, x1) + (y3 - x2 y1) \text{diff}(f, x2) + y1 y2 \text{diff}(f, y2) \\
& \quad - y1 y3 \text{diff}(f, y3) - y2 y3 \text{diff}(f, y4) : \text{simplify}(\{seq(VI(Vm1a(var[j]))) \\
& \quad + Vm1a(VI(var[j])) - U01(var[j]) + U02(var[j]), j=1..7), seq(U1(Vm1a(var[j]))) \\
& \quad - Vm1a(U1(var[j])), j=1..7), seq(U2(Vm1a(var[j]))) - Vm1a(U2(var[j])), j=1 \\
& \quad ..7)\})
\end{aligned}$$

$$\{0\} \quad (15)$$

$$\begin{aligned} &> Vm1b := f \rightarrow (x1 \ y1 - y2) \text{ diff}(f, x1) + k (x2 \ y1 - y3) \text{ diff}(f, x2) + y1 \ y2 \text{ diff}(f, y2) \\ &\quad + k \ y1 \ y3 \text{ diff}(f, y3) + (x3 + (1 + k) \ y1 \ y4) \text{ diff}(f, y4) + (1 + k) \ x3 \ y1 \text{ diff}(f, x3) : \\ &\quad \text{simplify}(\{seq(V1(Vm1b(var[j]))) + Vm1b(V1(var[j])) - U01(var[j]) \\ &\quad - k \ U02(var[j]), j = 1 \dots 7), seq(U1(Vm1b(var[j])) - Vm1b(U1(var[j])), j = 1 \dots 7), \\ &\quad seq(U2(Vm1b(var[j])) - Vm1b(U2(var[j])), j = 1 \dots 7)\}) \\ &\quad \{0\} \end{aligned} \quad (16)$$

General choice of Vm1

$$\begin{aligned} &> Vm1 := f \rightarrow \text{simplify}(Vm1a(f) + a \ Vm1b(f)) : seq(Vm1(Vm1(var[j])), j = 1 \dots 7) \\ &\quad 0, 0, 0, 0, 0, 0, 0 \end{aligned} \quad (17)$$

$$\begin{aligned} &> seq(\text{simplify}(Um1(Vm1(var[j]))) - Vm1(Um1(var[j])), j = 1 \dots 7); \\ &\quad seq(\text{simplify}(Um2(Vm1(var[j]))) - Vm1(Um2(var[j])), j = 1 \dots 7) \\ &- x1 \ (y1 \ x1 - y2) \ (a + 1), (y3 \ x1 - y4) \ (a \ k - 1), k \ x1 \ (a + 1) \ y1 \ y2 \ y3 - k \ (a + 1) \ y1 \ y2 \ y4 \\ &\quad - a \ x3 \ y2, (a + 1) \ y1 \ y2, 0, x2 \ (a + 1) \ y1 \ y2 + x1 \ (a + 1) \ y1 \ y3 + (-a - 1) \ y1 \ y4 \\ &\quad - a \ (x3 + y2 \ y3), -x1 \ (-x2 \ (a + 1) \ y1 \ y2 + (a + 1) \ y1 \ y4 + x3 \ a - y2 \ y3) \\ &(y2 \ x2 - y4) \ (a + 1), -x2 \ (y1 \ x2 - y3) \ (a \ k - 1), x2 \ (-a \ k + 1) \ y1 \ y2 \ y3 + (-a \ k \\ &\quad + 1) \ y1 \ y3 \ y4 - k \ a \ x3 \ y3, (a \ k - 1) \ y1 \ y3, x2 \ (a \ k - 1) \ y1 \ y2 + x1 \ (a \ k - 1) \ y1 \ y3 + ( \\ &\quad -a \ k + 1) \ y1 \ y4 + a \ (y2 \ y3 \ k - x3), 0, x2 \ (x1 \ (a \ k - 1) \ y1 \ y3 + (-a \ k + 1) \ y1 \ y4 - x3 \ a \\ &\quad + y2 \ y3) \end{aligned} \quad (18)$$

$$\begin{aligned} &> Vm2 := f \rightarrow -(a + 1) \ x1 \ (x1 \ y1 - y2) \text{ diff}(f, x1) + (a \ k - 1) \ (x1 \ y3 - y4) \text{ diff}(f, x2) + (a \\ &\quad + 1) \ y1 \ y2 \text{ diff}(f, y1) + ((a + 1) \ y1 \cdot (x2 \ y2 + x1 \ y3 - y4) - a \ (x3 + y2 \ y3)) \text{ diff}(f, y3) \\ &\quad + x1 \ ((a + 1) \ y1 \ (x2 \ y2 - y4) + y2 \ y3 - x3 \ a) \text{ diff}(f, y4) + (k \ (a + 1) \ y1 \ (x1 \ y2 \ y3 \\ &\quad - y2 \ y4) - a \ x3 \ y2) \text{ diff}(f, x3) : \\ &Vm3 := f \rightarrow (a + 1) \ (x2 \ y2 - y4) \text{ diff}(f, x1) - (a \ k - 1) \ x2 \ (x2 \ y1 - y3) \text{ diff}(f, x2) + (a \ k \\ &\quad - 1) \ y1 \ y3 \text{ diff}(f, y1) + ((a \ k - 1) \ y1 \ (x2 \ y2 + x1 \ y3 - y4) + a \ (k \ y2 \ y3 - x3)) \text{ diff}(f, \\ &\quad y2) + x2 \ ((a \ k - 1) \ y1 \ (x1 \ y3 - y4) + (y2 \ y3 - a \ x3)) \text{ diff}(f, y4) - ((a \ k \\ &\quad - 1) \ y3 \ (x2 \ y1 \ y2 - y1 \ y4) + a \ k \ x3 \ y3) \text{ diff}(f, x3) : \end{aligned}$$

$$\begin{aligned} &> seq(\text{simplify}(Um1(Vm1(var[j]))) - Vm1(Um1(var[j])) - Vm2(var[j])), j = 1 \dots 7), \\ &\quad seq(\text{simplify}(Um2(Vm1(var[j]))) - Vm1(Um2(var[j])) - Vm3(var[j])), j = 1 \dots 7) \\ &\quad 0, 0, 0, 0, 0, 0, 0, 0, 0, 0, 0, 0, 0, 0, 0 \end{aligned} \quad (19)$$

$$\begin{aligned} &> seq(\text{simplify}(Vm1(Vm2(var[j]))) + Vm2(Vm1(var[j])), j = 1 \dots 7), \\ &\quad seq(\text{simplify}(Vm1(Vm3(var[j]))) + Vm3(Vm1(var[j])), j = 1 \dots 7); \\ &\quad 0, 0, 0, 0, 0, 0, 0, 0, 0, 0, 0, 0, 0, 0, 0 \end{aligned} \quad (20)$$

$$\begin{aligned} &> seq(\text{simplify}(Um1(Vm2(var[j]))) - Vm2(Um1(var[j])), j = 1 \dots 7); \\ &\quad seq(\text{simplify}(Um1(Vm3(var[j]))) - Vm3(Um1(var[j])), j = 1 \dots 7); \\ &\quad seq(\text{simplify}(Um2(Vm2(var[j]))) - Vm2(Um2(var[j])), j = 1 \dots 7); \\ &\quad seq(\text{simplify}(Um2(Vm3(var[j]))) - Vm3(Um2(var[j])), j = 1 \dots 7); \\ &\quad 0, 0, 0, 0, 0, 0, 0, 0 \\ &- (y2 \ x2 - y4) \ (a + 1) \ x1, -x2 \ (y3 \ x1 - y4) \ (k \ a - 1), -(k + 1) \ y2 \ y3 \ y4, y2 \ y3 - x3 \ a, \\ &\quad - (k \ a - 1) \ (x1 \ y2 \ y3 - y2 \ y4), (x2 \ y2 \ y3 + y3 \ y4) \ (a + 1), 0 \\ &- (y2 \ x2 - y4) \ (a + 1) \ x1, -x2 \ (y3 \ x1 - y4) \ (k \ a - 1), -(k + 1) \ y2 \ y3 \ y4, y2 \ y3 - x3 \ a, \\ &\quad - (k \ a - 1) \ (x1 \ y2 \ y3 - y2 \ y4), (x2 \ y2 \ y3 + y3 \ y4) \ (a + 1), 0 \end{aligned}$$

$$0, 0, 0, 0, 0, 0, 0 \quad (21)$$

$$\begin{aligned} &> Vm4 := f \rightarrow -(a+1) x1 (x2 y2 - y4) \text{diff}(f, x1) - (a k - 1) x2 (x1 y3 - y4) \text{diff}(f, x2) \\ &\quad + (y2 y3 - a x3) \text{diff}(f, y1) - (a k - 1) y2 (x1 y3 - y4) \text{diff}(f, y2) - (a+1) y3 (x2 y2 \\ &\quad - y4) \text{diff}(f, y3) - (k+1) y2 y3 y4 \text{diff}(f, x3) : \end{aligned}$$

$$\begin{aligned} &> \text{seq}(\text{simplify}(Um1(Vm3(\text{var}[j]))) - Vm3(Um1(\text{var}[j]))) - Vm4(\text{var}[j])), j = 1..7, \\ &\quad \text{seq}(\text{simplify}(Um2(Vm2(\text{var}[j]))) - Vm2(Um2(\text{var}[j]))) - Vm4(\text{var}[j])), j = 1..7); \\ &\quad 0, 0, 0, 0, 0, 0, 0, 0, 0, 0, 0, 0, 0, 0, 0 \end{aligned} \quad (22)$$

$$\begin{aligned} &> \text{seq}(\text{simplify}(Vm2(Vm2(\text{var}[j]))), j = 1..7), \text{seq}(\text{simplify}(Vm3(Vm3(\text{var}[j]))), j = 1..7); \\ &\quad \text{seq}(\text{simplify}(Um1(Vm4(\text{var}[j]))) - Vm4(Um1(\text{var}[j]))), j = 1..7), \\ &\quad \text{seq}(\text{simplify}(Um2(Vm4(\text{var}[j]))) - Vm4(Um2(\text{var}[j]))), j = 1..7) \\ &\quad 0, 0, 0, 0, 0, 0, 0, 0, 0, 0, 0, 0, 0, 0, 0 \\ &\quad 0, 0, 0, 0, 0, 0, 0, 0, 0, 0, 0, 0, 0, 0, 0 \end{aligned} \quad (23)$$

$$\begin{aligned} &> \text{seq}(\text{simplify}(Vm2(Vm3(\text{var}[j]))) + Vm3(Vm2(\text{var}[j]))), j = 1..7) \\ a (k+1) (x1 x2 y1 y2 - y1 y4 x1 + y2 y4) (a+1), a (k+1) (y1 y3 x1 x2 - y1 y4 x2 \\ &\quad + y3 y4) (k a - 1), (k+1) ((k+1) y1 y2 y3 y4 + x3^2 a) a, a (k+1) (a x3 y1 \\ &\quad - y1 y2 y3), -(x1 (-k a + 1) y1 y2 y3 + (k a - 1) y1 y2 y4 - x3 y2 a) (k+1) a, -(k \\ &\quad + 1) ((a+1) x2 y1 y2 y3 + (a+1) y1 y3 y4 - x3 y3 a) a, a (k+1) (a x3 y4 - y2 y3 y4) \end{aligned} \quad (24)$$

$$\begin{aligned} &> \text{seq}(\text{simplify}(Vm1(Vm4(\text{var}[j]))) + Vm4(Vm1(\text{var}[j]))) + Vm2(Vm3(\text{var}[j])) \\ &\quad + Vm3(Vm2(\text{var}[j])), j = 1..7) \\ &\quad 0, 0, 0, 0, 0, 0, 0, 0 \end{aligned} \quad (25)$$

$$\begin{aligned} &> Um3 := f \rightarrow a (a+1) (k+1) (x1 x2 y1 y2 - x1 y1 y4 + y2 y4) \text{diff}(f, x1) + a (a k - 1) (k \\ &\quad + 1) (x1 x2 y1 y3 - x2 y1 y4 + y3 y4) \text{diff}(f, x2) + a (k+1) y1 (a x3 - y2 y3) \text{diff}(f, \\ &\quad y1) + a (k+1) ((a k - 1) y1 y2 (x1 y3 - y4) + a x3 y2) \text{diff}(f, y2) - a (k+1) ((a \\ &\quad + 1) y1 (x2 y2 y3 + y3 y4) - a x3 y3) \text{diff}(f, y3) + a (k+1) y4 (a x3 - y2 y3) \text{diff}(f, \\ &\quad y4) + a (k+1) ((k+1) y1 y2 y3 y4 + a x3^2) \text{diff}(f, x3) : \end{aligned}$$

$$\begin{aligned} &> \text{seq}(\text{simplify}(Vm2(Vm3(\text{var}[j]))) + Vm3(Vm2(\text{var}[j]))) - Um3(\text{var}[j])), j = 1..7, \\ &\quad \text{seq}(\text{simplify}(Vm1(Vm4(\text{var}[j]))) + Vm4(Vm1(\text{var}[j]))) + Um3(\text{var}[j])), j = 1..7) \\ &\quad 0, 0, 0, 0, 0, 0, 0, 0, 0, 0, 0, 0, 0, 0, 0 \end{aligned} \quad (26)$$

$$\begin{aligned} &> \text{seq}(\text{simplify}(Um1(Um3(\text{var}[j]))) - Um3(Um1(\text{var}[j]))), j = 1..7), \\ &\quad \text{seq}(\text{simplify}(Um2(Um3(\text{var}[j]))) - Um3(Um2(\text{var}[j]))), j = 1..7) \\ &\quad 0, 0, 0, 0, 0, 0, 0, 0, 0, 0, 0, 0, 0, 0, 0 \end{aligned} \quad (27)$$

$$\begin{aligned} &> \text{seq}(\text{simplify}(Vm1(Um3(\text{var}[j]))) - Um3(Vm1(\text{var}[j]))), j = 1..7), \\ &\quad \text{seq}(\text{simplify}(Vm2(Um3(\text{var}[j]))) - Um3(Vm2(\text{var}[j]))), j = 1..7), \\ &\quad \text{seq}(\text{simplify}(Vm3(Um3(\text{var}[j]))) - Um3(Vm3(\text{var}[j]))), j = 1..7), \\ &\quad \text{seq}(\text{simplify}(Vm4(Um3(\text{var}[j]))) - Um3(Vm4(\text{var}[j]))), j = 1..7) \\ &\quad 0, 0, 0, 0, 0, 0, 0, 0, 0, 0, 0, 0, 0, 0, 0, 0, 0, 0, 0, 0, 0, 0, 0, 0, 0, 0, 0, 0, 0, 0 \end{aligned} \quad (28)$$

$$\begin{aligned} &> \text{seq}(\text{simplify}(Vm2(Vm4(\text{var}[j]))) + Vm4(Vm2(\text{var}[j]))), j = 1..7), \\ &\quad \text{seq}(\text{simplify}(Vm3(Vm4(\text{var}[j]))) + Vm4(Vm3(\text{var}[j]))), j = 1..7), \\ &\quad \text{seq}(\text{simplify}(Vm4(Vm4(\text{var}[j]))), j = 1..7) \\ &\quad 0, 0, 0, 0, 0, 0, 0, 0, 0, 0, 0, 0, 0, 0, 0, 0, 0, 0, 0, 0, 0, 0, 0, 0, 0, 0, 0, 0, 0 \end{aligned} \quad (29)$$

$$\begin{aligned} \# \text{ ` } [Um1, Vm1] &= Vm2, [Um2, Vm1] = Vm3, [Um2, Vm2] = Vm4, [Um1, Vm3] = Vm4, [Vm1, \\ Vm4] &= -Um3, [Vm2, Vm3] = Um3 \end{aligned}$$

$$\begin{aligned}
&> \text{simplify}(\{ \text{seq}(U01(Um1(\text{var}[j])) - Um1(U01(\text{var}[j])) - Um1(\text{var}[j]), j=1..7), \\
&\quad \text{seq}(U01(Um2(\text{var}[j])) - Um2(U01(\text{var}[j])), j=1..7), \text{seq}(U01(Vm1(\text{var}[j])) \\
&\quad - Vm1(U01(\text{var}[j])), j=1..7), \\
&\quad \text{seq}(U02(Um1(\text{var}[j])) - Um1(U02(\text{var}[j])), j=1..7), \text{seq}(U02(Um2(\text{var}[j])) \\
&\quad - Um2(U02(\text{var}[j])) - Um2(\text{var}[j]), j=1..7), \text{seq}(U02(Vm1(\text{var}[j])) \\
&\quad - Vm1(U02(\text{var}[j])), j=1..7), \\
&\quad \text{seq}(U03(Um1(\text{var}[j])) - Um1(U03(\text{var}[j])), j=1..7), \text{seq}(U03(Um2(\text{var}[j])) \\
&\quad - Um2(U03(\text{var}[j])), j=1..7), \text{seq}(U03(Vm1(\text{var}[j])) - Vm1(U03(\text{var}[j])) \\
&\quad - Vm1(\text{var}[j]), j=1..7) \} \} \\
&\qquad\qquad\qquad \{0\} \tag{30}
\end{aligned}$$

$$\begin{aligned}
&> \text{simplify}(\{ \text{seq}(Z(Um1(\text{var}[j])) - Um1(Z(\text{var}[j])) - Um1(\text{var}[j]), j=1..7), \\
&\quad \text{seq}(Z(Um2(\text{var}[j])) - Um2(Z(\text{var}[j])) - Um2(\text{var}[j]), j=1..7), \\
&\quad \text{seq}(Z(Um3(\text{var}[j])) - Um3(Z(\text{var}[j])) - 4 Um3(\text{var}[j]), j=1..7), \\
&\quad \text{seq}(Z(Vm1(\text{var}[j])) - Vm1(Z(\text{var}[j])) - Vm1(\text{var}[j]), j=1..7), \\
&\quad \text{seq}(Z(Vm2(\text{var}[j])) - Vm2(Z(\text{var}[j])) - 2 Vm2(\text{var}[j]), j=1..7), \\
&\quad \text{seq}(Z(Vm3(\text{var}[j])) - Vm3(Z(\text{var}[j])) - 2 Vm3(\text{var}[j]), j=1..7), \\
&\quad \text{seq}(Z(Vm4(\text{var}[j])) - Vm4(Z(\text{var}[j])) - 3 Vm4(\text{var}[j]), j=1..7) \} \} \\
&\qquad\qquad\qquad \{0\} \tag{31}
\end{aligned}$$

Now we compute the parameter in D(2,1;a) via pairing between g[-] and g[+]

$$\begin{aligned}
&> \text{seq}(\text{simplify}(U1(Um1(\text{var}[j])) - Um1(U1(\text{var}[j])) - 2 U01(\text{var}[j]) + U03(\text{var}[j])), j \\
&\quad = 1..7); \\
&\text{seq}(\text{simplify}(U2(Um2(\text{var}[j])) - Um2(U2(\text{var}[j])) - 2 U02(\text{var}[j]) + U03(\text{var}[j])), j \\
&\quad = 1..7); \\
&\text{seq}(\text{simplify}(U3(Um3(\text{var}[j])) - Um3(U3(\text{var}[j])) - a^2 (k+1)^2 U03(\text{var}[j])), j=1..7) \\
&\qquad\qquad\qquad 0, 0, 0, 0, 0, 0, 0 \\
&\qquad\qquad\qquad 0, 0, 0, 0, 0, 0, 0 \\
&\qquad\qquad\qquad 0, 0, 0, 0, 0, 0, 0 \tag{32}
\end{aligned}$$

$$\begin{aligned}
&> H1 := f \rightarrow U03(f) : H2 := f \rightarrow 2 U01(f) - U03(f) : H3 := f \rightarrow 2 U02(f) - U03(f) : \\
&> \text{simplify}(\{ \text{seq}(H1(Um3(\text{var}[j])) - Um3(H1(\text{var}[j])) - 2 Um3(\text{var}[j]), j=1..7), \\
&\quad \text{seq}(H2(Um1(\text{var}[j])) - Um1(H2(\text{var}[j])) - 2 Um1(\text{var}[j]), j=1..7), \\
&\quad \text{seq}(H3(Um2(\text{var}[j])) - Um2(H3(\text{var}[j])) - 2 Um2(\text{var}[j]), j=1..7) \} \} \\
&\qquad\qquad\qquad \{0\} \tag{33}
\end{aligned}$$

$$\begin{aligned}
&> \text{seq}(\text{simplify}(V1(Vm1(\text{var}[j])) + Vm1(V1(\text{var}[j])) + (a+1) U01(\text{var}[j]) + (a k \\
&\quad - 1) U02(\text{var}[j])), j=1..7) \\
&\qquad\qquad\qquad 0, 0, 0, 0, 0, 0, 0 \tag{34}
\end{aligned}$$

$$\begin{aligned}
&> \text{seq}(\text{simplify}(V4(Vm4(\text{var}[j])) + Vm4(V4(\text{var}[j])) - (a+1) U01(\text{var}[j]) - (a k \\
&\quad - 1) U02(\text{var}[j]) + a (k+1) U03(\text{var}[j])), j=1..7) \\
&\qquad\qquad\qquad 0, 0, 0, 0, 0, 0, 0 \tag{35}
\end{aligned}$$

$$\begin{aligned}
&> \text{seq}\left(\text{simplify}\left(V1(Vm1(\text{var}[j])) + Vm1(V1(\text{var}[j])) + \frac{a(k+1)}{2} H1(\text{var}[j]) \right. \right. \\
&\quad \left. \left. + \frac{a+1}{2} H2(\text{var}[j]) + \frac{k a - 1}{2} H3(\text{var}[j]) \right), j=1..7\right) \\
&\qquad\qquad\qquad 0, 0, 0, 0, 0, 0, 0 \tag{36}
\end{aligned}$$

$$\begin{aligned} & \text{seq}\left(\text{simplify}\left(V4(Vm4(\text{var}[j])) + Vm4(V4(\text{var}[j])) + \frac{a(k+1)}{2} H1(\text{var}[j])\right.\right. \\ & \quad \left.\left. - \frac{a+1}{2} H2(\text{var}[j]) - \frac{ka-1}{2} H3(\text{var}[j])\right), j=1..7\right) \\ & \quad \quad \quad 0, 0, 0, 0, 0, 0, 0 \end{aligned} \tag{37}$$

$$\begin{aligned} & \text{seq}(\text{simplify}(V2(Vm2(\text{var}[j])) + Vm2(V2(\text{var}[j])) - (a+1) U01(\text{var}[j]) + (ak \\ & \quad - 1) U02(\text{var}[j]) + (a+1) U03(\text{var}[j])), j=1..7); \\ & \text{seq}(\text{simplify}(V2(Vm3(\text{var}[j])) + Vm3(V2(\text{var}[j]))), j=1..7); \\ & \text{seq}(\text{simplify}(V3(Vm2(\text{var}[j])) + Vm2(V3(\text{var}[j]))), j=1..7); \\ & \text{seq}(\text{simplify}(V3(Vm3(\text{var}[j])) + Vm3(V3(\text{var}[j])) + (a+1) U01(\text{var}[j]) - (ak \\ & \quad - 1) U02(\text{var}[j]) + (ak-1) U03(\text{var}[j])), j=1..7) \\ & \quad \quad \quad 0, 0, 0, 0, 0, 0, 0 \\ & \quad \quad \quad 0, 0, 0, 0, 0, 0, 0 \\ & \quad \quad \quad 0, 0, 0, 0, 0, 0, 0 \\ & \quad \quad \quad 0, 0, 0, 0, 0, 0, 0 \end{aligned} \tag{38}$$

$$\begin{aligned} & \text{solve}\left(\left\{1 + \alpha = \rho \frac{a(k+1)}{2}, 1 = \rho \frac{a+1}{2}, \alpha = \rho \frac{ka-1}{2}\right\}, \{\alpha, \rho\}\right) \\ & \quad \quad \quad \left\{\alpha = \frac{ka-1}{a+1}, \rho = \frac{2}{a+1}\right\} \end{aligned} \tag{39}$$

$$\begin{aligned} & \text{simplify}\left(-1 - \frac{ka-1}{a+1}\right), \text{simplify}\left(-1 + \frac{a+1}{a(k+1)}\right), \text{simplify}\left(-1 - \frac{a(k+1)}{-ka+1}\right) \\ & \quad \quad \quad - \frac{a(k+1)}{a+1}, \frac{-ka+1}{a(k+1)}, \frac{a+1}{ka-1} \end{aligned} \tag{40}$$

>
