# Supplementary material for: Geometric realizations of the Lie superalgebra D(2,1;a)
Source: arXiv:2507.03418 ancillary file (2025-07-04)
Supplement: Supplementary file 2 [file H1forD21alpha.pdf]

```

> with(LinearAlgebra) : with(DifferentialGeometry) : with(LieAlgebras) :
  Preferences("ShowFramePrompt",false) : interface(warnlevel=0) : with(Groebner) :
> # with(Physics) : KroneckerDelta[1,2]

```

## osp(4|2,α)

```

> δ[1,1] := 1 : δ[1,2] := 0 : δ[1,3] := 0 : δ[2,1] := 0 : δ[2,2] := 1 : δ[2,3] := 0 : δ[3,
  1] := 0 : δ[3,2] := 0 : δ[3,3] := 1 :
for i to 3 do ε[0,0,i] := 0 : ε[0,1,i] := 2 Y[i] : ε[0,2,i] := -H[i] : ε[1,0,i] := -2 Y[i] :
  ε[1,1,i] := 0 : ε[1,2,i] := 2 X[i] : ε[2,0,i] := H[i] : ε[2,1,i] := -2 X[i] : ε[2,2,
  i] := 0 : od:
δ2[0,0] := 0 : δ2[0,1] := 1 : δ2[1,0] := -1 : δ2[1,1] := 1 : δ2[2,0] := 1 : δ2[2,1] :=
  0 : x0 := 1 : x1 :=  $\frac{1}{2}$  : x2 := -1 :
ε[0,0] := 0 : ε[0,1] := 1 : ε[1,0] := -1 : ε[1,1] := 0 : YHX[0] := Y : YHX[1] := H :
  YHX[2] := X :
> for i1 from 0 to 2 do for i2 from 0 to 2 do for j1 to 3 do for j2 to 3 do Br[YHX[i1][j1],
  YHX[i2][j2]] := δ[j1,j2]·ε[i1,i2,j1] : od:od:od:od:
> for i1 from 0 to 2 do for i2 from 0 to 1 do for j2 from 0 to 1 do for k2 from 0 to 1
  do Br[YHX[i1][1], W[i2,j2,k2]] := δ2[i1,i2]·W[i1+i2-1,j2,k2] : Br[W[i2,j2,k2],
  YHX[i1][1]] := -δ2[i1,i2]·W[i1+i2-1,j2,k2] : Br[YHX[i1][2], W[i2,j2,k2]] :=
  δ2[i1,j2]·W[i2,i1+j2-1,k2] : Br[W[i2,j2,k2], YHX[i1][2]] := -δ2[i1,j2]·W[i2,i1
  +j2-1,k2] : Br[YHX[i1][3], W[i2,j2,k2]] := δ2[i1,k2]·W[i2,j2,i1+k2-1] :
  Br[W[i2,j2,k2], YHX[i1][3]] := -δ2[i1,k2]·W[i2,j2,i1+k2-1] : od:od:od:od:
> for i1 from 0 to 1 do for j1 from 0 to 1 do for k1 from 0 to 1 do for i2 from 0 to 1 do for j2
  from 0 to 1 do for k2 from 0 to 1 do Br[W[i1,j1,k1], W[i2,j2,k2]] := s1·x[i1+i2]
  ·YHX[i1+i2][1]·ε[j1,j2]·ε[k1,k2] + s2·x[j1+j2]·YHX[j1+j2][2]·ε[i1,i2]·ε[k1,
  k2] + s3·x[k1+k2]·YHX[k1+k2][3]·ε[i1,i2]·ε[j1,j2] : od:od:od:od:od:od:
> for i1 from 0 to 1 do for j1 from 0 to 1 do for k1 from 0 to 1 do for i2 from 0 to 1 do for j2
  from 0 to 1 do for k2 from 0 to 1 do sBr[W[i1,j1,k1], W[i2,j2,k2]] := s1·x[i1+i2]
  ·YHX[i1+i2][1]·ε[j1,j2]·ε[k1,k2] + s2·x[j1+j2]·YHX[j1+j2][2]·ε[i1,i2]·ε[k1,
  k2] + s3·x[k1+k2]·YHX[k1+k2][3]·ε[i1,i2]·ε[j1,j2] : od:od:od:od:od:od:
> -2 Br[W[1,0,1], W[0,1,0]]
  s1 H1 - s2 H2 + s3 H3 (1.1)
> Ev := [Y[1], H[1], X[1], Y[2], H[2], X[2], Y[3], H[3], X[3]] : Ov := [W[0,0,0], W[1,0,
  0], W[0,1,0], W[1,1,0], W[0,0,1], W[1,0,1], W[0,1,1], W[1,1,1]] : n0 :=
  nops(Ev) : n1 := nops(Ov) : N := n0 + n1 : eV := A→[seq(diff(A, Ev[i]), i = 1..n0)] :
  oV := A→[seq(diff(A, Ov[i]), i = 1..n1)] :
> for i to 9 do for j to 9 do for k to 9 do c[i,j,k] := eV(Br[Ev[i], Ev[j]])(k) : od:od:od:
> Me := i→Matrix((k,j)→c[i,j,k], 9) : L1 := LieAlgebraData([seq(Me(i), i = 1..9)], alg1)
L1 := [[e1, e2] = 2 e1, [e1, e3] = -e2, [e2, e3] = 2 e3, [e4, e5] = 2 e4, [e4, e6] = -e5, [e5,
  e6] = 2 e6, [e7, e8] = 2 e7, [e7, e9] = -e8, [e8, e9] = 2 e9] (1.2)
> RpE1 := [seq(Transpose(Matrix([seq(oV(Br[Ev[i], Ov[j]]), j = 1..n1)])), i = 1..n0)] :
  unassign(VI) :

```

>  $DGsetup(L1) : DGsetup([seq(x||i, i = 1..n0)], V1) : \rho1 := Representation(alg1, V1, RpE1);$   
 $Query(\rho1, "Representation");$

$$\rho1 := \left[ \begin{array}{c} e1, \\ \begin{bmatrix} 0 & 1 & 0 & 0 & 0 & 0 & 0 & 0 \\ 0 & 0 & 0 & 0 & 0 & 0 & 0 & 0 \\ 0 & 0 & 0 & 1 & 0 & 0 & 0 & 0 \\ 0 & 0 & 0 & 0 & 0 & 0 & 0 & 0 \\ 0 & 0 & 0 & 0 & 0 & 1 & 0 & 0 \\ 0 & 0 & 0 & 0 & 0 & 0 & 0 & 0 \\ 0 & 0 & 0 & 0 & 0 & 0 & 0 & 1 \\ 0 & 0 & 0 & 0 & 0 & 0 & 0 & 0 \end{bmatrix} \end{array} \right], e2, \left[ \begin{array}{c} e3, \\ \begin{bmatrix} -1 & 0 & 0 & 0 & 0 & 0 & 0 & 0 \\ 0 & 1 & 0 & 0 & 0 & 0 & 0 & 0 \\ 0 & 0 & -1 & 0 & 0 & 0 & 0 & 0 \\ 0 & 0 & 0 & 1 & 0 & 0 & 0 & 0 \\ 0 & 0 & 0 & 0 & -1 & 0 & 0 & 0 \\ 0 & 0 & 0 & 0 & 0 & 1 & 0 & 0 \\ 0 & 0 & 0 & 0 & 0 & 0 & -1 & 0 \\ 0 & 0 & 0 & 0 & 0 & 0 & 0 & 1 \end{bmatrix} \end{array} \right],$$

$$\left[ \begin{array}{c} e4, \\ \begin{bmatrix} 0 & 0 & 0 & 0 & 0 & 0 & 0 & 0 \\ 1 & 0 & 0 & 0 & 0 & 0 & 0 & 0 \\ 0 & 0 & 0 & 0 & 0 & 0 & 0 & 0 \\ 0 & 0 & 1 & 0 & 0 & 0 & 0 & 0 \\ 0 & 0 & 0 & 0 & 0 & 0 & 0 & 0 \\ 0 & 0 & 0 & 0 & 0 & 0 & 0 & 0 \\ 0 & 0 & 0 & 0 & 1 & 0 & 0 & 0 \\ 0 & 0 & 0 & 0 & 0 & 0 & 0 & 0 \\ 0 & 0 & 0 & 0 & 0 & 0 & 1 & 0 \end{bmatrix} \end{array} \right], e5, \left[ \begin{array}{c} e6, \\ \begin{bmatrix} 0 & 0 & 1 & 0 & 0 & 0 & 0 & 0 \\ 0 & 0 & 0 & 1 & 0 & 0 & 0 & 0 \\ 0 & 0 & 0 & 0 & 0 & 0 & 0 & 0 \\ 0 & 0 & 0 & 0 & 0 & 0 & 0 & 0 \\ 0 & 0 & 0 & 0 & 0 & 0 & 1 & 0 \\ 0 & 0 & 0 & 0 & 0 & 0 & 0 & 1 \\ 0 & 0 & 0 & 0 & 0 & 0 & 0 & 0 \\ 0 & 0 & 0 & 0 & 0 & 0 & 0 & 0 \end{bmatrix} \end{array} \right],$$

$$\left[ \begin{array}{c} e7, \\ \begin{bmatrix} -1 & 0 & 0 & 0 & 0 & 0 & 0 & 0 \\ 0 & -1 & 0 & 0 & 0 & 0 & 0 & 0 \\ 0 & 0 & 1 & 0 & 0 & 0 & 0 & 0 \\ 0 & 0 & 0 & 1 & 0 & 0 & 0 & 0 \\ 0 & 0 & 0 & 0 & -1 & 0 & 0 & 0 \\ 0 & 0 & 0 & 0 & 0 & -1 & 0 & 0 \\ 0 & 0 & 0 & 0 & 0 & 0 & 1 & 0 \\ 0 & 0 & 0 & 0 & 0 & 0 & 0 & 1 \end{bmatrix} \end{array} \right], e7, \left[ \begin{array}{c} e7, \\ \begin{bmatrix} 0 & 0 & 0 & 0 & 0 & 0 & 0 & 0 \\ 0 & 0 & 0 & 0 & 0 & 0 & 0 & 0 \\ 1 & 0 & 0 & 0 & 0 & 0 & 0 & 0 \\ 0 & 1 & 0 & 0 & 0 & 0 & 0 & 0 \\ 0 & 0 & 0 & 0 & 0 & 0 & 0 & 0 \\ 0 & 0 & 0 & 0 & 0 & 0 & 0 & 0 \\ 0 & 0 & 0 & 0 & 1 & 0 & 0 & 0 \\ 0 & 0 & 0 & 0 & 0 & 1 & 0 & 0 \end{bmatrix} \end{array} \right]$$

$$\begin{aligned}
& \left[ \begin{array}{cccccccc} 0 & 0 & 0 & 0 & 1 & 0 & 0 & 0 \\ 0 & 0 & 0 & 0 & 0 & 1 & 0 & 0 \\ 0 & 0 & 0 & 0 & 0 & 0 & 1 & 0 \\ 0 & 0 & 0 & 0 & 0 & 0 & 0 & 1 \\ 0 & 0 & 0 & 0 & 0 & 0 & 0 & 0 \\ 0 & 0 & 0 & 0 & 0 & 0 & 0 & 0 \\ 0 & 0 & 0 & 0 & 0 & 0 & 0 & 0 \\ 0 & 0 & 0 & 0 & 0 & 0 & 0 & 0 \end{array} \right] \Bigg] , e8, \left[ \begin{array}{cccccccc} -1 & 0 & 0 & 0 & 0 & 0 & 0 & 0 \\ 0 & -1 & 0 & 0 & 0 & 0 & 0 & 0 \\ 0 & 0 & -1 & 0 & 0 & 0 & 0 & 0 \\ 0 & 0 & 0 & -1 & 0 & 0 & 0 & 0 \\ 0 & 0 & 0 & 0 & 1 & 0 & 0 & 0 \\ 0 & 0 & 0 & 0 & 0 & 1 & 0 & 0 \\ 0 & 0 & 0 & 0 & 0 & 0 & 1 & 0 \\ 0 & 0 & 0 & 0 & 0 & 0 & 0 & 1 \end{array} \right] \Bigg] , e9, \\
& \left[ \begin{array}{cccccccc} 0 & 0 & 0 & 0 & 0 & 0 & 0 & 0 \\ 0 & 0 & 0 & 0 & 0 & 0 & 0 & 0 \\ 0 & 0 & 0 & 0 & 0 & 0 & 0 & 0 \\ 0 & 0 & 0 & 0 & 0 & 0 & 0 & 0 \\ 1 & 0 & 0 & 0 & 0 & 0 & 0 & 0 \\ 0 & 1 & 0 & 0 & 0 & 0 & 0 & 0 \\ 0 & 0 & 1 & 0 & 0 & 0 & 0 & 0 \\ 0 & 0 & 0 & 1 & 0 & 0 & 0 & 0 \end{array} \right] \Bigg]
\end{aligned}$$

*true*

**(1.3)**

> [seq([f||i, Transpose(Matrix([seq(eV(sBr[Ov[i], Ov[j]]), j=1..nl)]))], i=1..nl)]

$$\begin{aligned}
& \left[ \left[ \begin{array}{cccccccc} 0 & 0 & 0 & 0 & 0 & 0 & s1 & 0 \\ 0 & 0 & 0 & 0 & 0 & 0 & 0 & \frac{s1}{2} \\ 0 & 0 & 0 & 0 & 0 & 0 & 0 & 0 \\ 0 & 0 & 0 & 0 & 0 & s2 & 0 & 0 \\ 0 & 0 & 0 & 0 & 0 & 0 & 0 & \frac{s2}{2} \\ 0 & 0 & 0 & 0 & 0 & 0 & 0 & 0 \\ 0 & 0 & 0 & s3 & 0 & 0 & 0 & 0 \\ 0 & 0 & 0 & 0 & 0 & 0 & 0 & \frac{s3}{2} \\ 0 & 0 & 0 & 0 & 0 & 0 & 0 & 0 \end{array} \right] , \left[ \begin{array}{cccccccc} 0 & 0 & 0 & 0 & 0 & 0 & 0 & 0 \\ 0 & 0 & 0 & 0 & 0 & 0 & \frac{s1}{2} & 0 \\ 0 & 0 & 0 & 0 & 0 & 0 & 0 & -s1 \\ 0 & 0 & 0 & 0 & -s2 & 0 & 0 & 0 \\ 0 & 0 & 0 & 0 & 0 & 0 & -\frac{s2}{2} & 0 \\ 0 & 0 & 0 & 0 & 0 & 0 & 0 & 0 \\ 0 & 0 & -s3 & 0 & 0 & 0 & 0 & 0 \\ 0 & 0 & 0 & 0 & 0 & 0 & -\frac{s3}{2} & 0 \\ 0 & 0 & 0 & 0 & 0 & 0 & 0 & 0 \end{array} \right] \right] ,
\end{aligned}$$

**(1.4)**

$$\left[ \begin{array}{c} f3, \\ \left[ \begin{array}{cccccccc} 0 & 0 & 0 & 0 & -s1 & 0 & 0 & 0 \\ 0 & 0 & 0 & 0 & 0 & -\frac{s1}{2} & 0 & 0 \\ 0 & 0 & 0 & 0 & 0 & 0 & 0 & 0 \\ 0 & 0 & 0 & 0 & 0 & 0 & 0 & 0 \\ 0 & 0 & 0 & 0 & 0 & \frac{s2}{2} & 0 & 0 \\ 0 & 0 & 0 & 0 & 0 & 0 & 0 & -s2 \\ 0 & -s3 & 0 & 0 & 0 & 0 & 0 & 0 \\ 0 & 0 & 0 & 0 & 0 & -\frac{s3}{2} & 0 & 0 \\ 0 & 0 & 0 & 0 & 0 & 0 & 0 & 0 \end{array} \right] \end{array} \right], f4, \\ \left[ \begin{array}{c} \left[ \begin{array}{cccccccc} 0 & 0 & 0 & 0 & 0 & 0 & 0 & 0 \\ 0 & 0 & 0 & 0 & -\frac{s1}{2} & 0 & 0 & 0 \\ 0 & 0 & 0 & 0 & 0 & s1 & 0 & 0 \\ 0 & 0 & 0 & 0 & 0 & 0 & 0 & 0 \\ 0 & 0 & 0 & 0 & -\frac{s2}{2} & 0 & 0 & 0 \\ 0 & 0 & 0 & 0 & 0 & 0 & s2 & 0 \\ s3 & 0 & 0 & 0 & 0 & 0 & 0 & 0 \\ 0 & 0 & 0 & 0 & \frac{s3}{2} & 0 & 0 & 0 \\ 0 & 0 & 0 & 0 & 0 & 0 & 0 & 0 \end{array} \right] \end{array} \right], f5, \\ \left[ \begin{array}{c} \left[ \begin{array}{cccccccc} 0 & 0 & -s1 & 0 & 0 & 0 & 0 & 0 \\ 0 & 0 & 0 & -\frac{s1}{2} & 0 & 0 & 0 & 0 \\ 0 & 0 & 0 & 0 & 0 & 0 & 0 & 0 \\ 0 & -s2 & 0 & 0 & 0 & 0 & 0 & 0 \\ 0 & 0 & 0 & -\frac{s2}{2} & 0 & 0 & 0 & 0 \\ 0 & 0 & 0 & 0 & 0 & 0 & 0 & 0 \\ 0 & 0 & 0 & 0 & 0 & 0 & 0 & 0 \\ 0 & 0 & 0 & \frac{s3}{2} & 0 & 0 & 0 & 0 \\ 0 & 0 & 0 & 0 & 0 & 0 & 0 & -s3 \end{array} \right] \end{array} \right],
\end{array}$$

$$\begin{aligned}
& \left[ \begin{array}{c} f6, \\ \left[ \begin{array}{cccccccc} 0 & 0 & 0 & 0 & 0 & 0 & 0 & 0 \\ 0 & 0 & -\frac{s1}{2} & 0 & 0 & 0 & 0 & 0 \\ 0 & 0 & 0 & s1 & 0 & 0 & 0 & 0 \\ s2 & 0 & 0 & 0 & 0 & 0 & 0 & 0 \\ 0 & 0 & \frac{s2}{2} & 0 & 0 & 0 & 0 & 0 \\ 0 & 0 & 0 & 0 & 0 & 0 & 0 & 0 \\ 0 & 0 & 0 & 0 & 0 & 0 & 0 & 0 \\ 0 & 0 & -\frac{s3}{2} & 0 & 0 & 0 & 0 & 0 \\ 0 & 0 & 0 & 0 & 0 & 0 & s3 & 0 \end{array} \right] \end{array} \right], \left[ \begin{array}{c} f7, \\ \left[ \begin{array}{cccccccc} s1 & 0 & 0 & 0 & 0 & 0 & 0 & 0 \\ 0 & \frac{s1}{2} & 0 & 0 & 0 & 0 & 0 & 0 \\ 0 & 0 & 0 & 0 & 0 & 0 & 0 & 0 \\ 0 & 0 & 0 & 0 & 0 & 0 & 0 & 0 \\ 0 & -\frac{s2}{2} & 0 & 0 & 0 & 0 & 0 & 0 \\ 0 & 0 & 0 & s2 & 0 & 0 & 0 & 0 \\ 0 & 0 & 0 & 0 & 0 & 0 & 0 & 0 \\ 0 & -\frac{s3}{2} & 0 & 0 & 0 & 0 & 0 & 0 \\ 0 & 0 & 0 & 0 & 0 & s3 & 0 & 0 \end{array} \right] \end{array} \right], f8, \\
& \left[ \begin{array}{c} \left[ \begin{array}{cccccccc} 0 & 0 & 0 & 0 & 0 & 0 & 0 & 0 \\ \frac{s1}{2} & 0 & 0 & 0 & 0 & 0 & 0 & 0 \\ 0 & -s1 & 0 & 0 & 0 & 0 & 0 & 0 \\ 0 & 0 & 0 & 0 & 0 & 0 & 0 & 0 \\ \frac{s2}{2} & 0 & 0 & 0 & 0 & 0 & 0 & 0 \\ 0 & 0 & -s2 & 0 & 0 & 0 & 0 & 0 \\ 0 & 0 & 0 & 0 & 0 & 0 & 0 & 0 \\ \frac{s3}{2} & 0 & 0 & 0 & 0 & 0 & 0 & 0 \\ 0 & 0 & 0 & 0 & -s3 & 0 & 0 & 0 \end{array} \right] \end{array} \right]
\end{aligned}$$

```

> for i from 1 to n0 do for j from 1 to n0 do for k from 1 to n0 do c[i,j,k] := eV(Br[Ev[i],
  Ev[j]])[k] :od:od:od:
for i from 1 to n0 do for j from 1 to n0 do for k from (n0 + 1) to N do c[i,j,k] := 0 :od:od:
od:
for i from 1 to n0 do for j from (n0 + 1) to N do for k from 1 to n0 do c[i,j,k] := 0 :od:od:
od:
for i from 1 to n0 do for j from (n0 + 1) to N do for k from (n0 + 1) to N do c[i,j,k] :=
  oV(Br[Ev[i], Ov[j - n0]])[k - n0] :od:od:od:
for i from (n0 + 1) to N do for j from 1 to n0 do for k from 1 to n0 do c[i,j,k] := 0 :od:od:
od:
for i from (n0 + 1) to N do for j from 1 to n0 do for k from (n0 + 1) to N do c[i,j,k] :=
  oV(Br[Ov[i - n0], Ev[j]])[k - n0] :od:od:od:
for i from (n0 + 1) to N do for j from (n0 + 1) to N do for k from 1 to n0 do c[i,j,k] :=
  eV(sBr[Ov[i - n0], Ov[j - n0]])[k] :od:od:od:
for i from (n0 + 1) to N do for j from (n0 + 1) to N do for k from (n0 + 1) to N do c[i,j,

```

$k] := 0 : \text{od} : \text{od} : \text{od} :$

$$\begin{aligned} &> \text{JacEEE} := (i, j, k) \rightarrow \text{simplify}(\text{add}(\text{Br}[\text{Ev}[l], \text{Ev}[k]] \cdot eV(\text{Br}[\text{Ev}[i], \text{Ev}[j]])([l] + \text{Br}[\text{Ev}[l], \\ &\quad \text{Ev}[i]] \cdot eV(\text{Br}[\text{Ev}[j], \text{Ev}[k]])([l] + \text{Br}[\text{Ev}[l], \text{Ev}[j]] \cdot eV(\text{Br}[\text{Ev}[k], \text{Ev}[i]])([l], l = 1 \dots 9)) : \\ &\quad \{ \text{seq}(\text{seq}(\text{seq}(\text{JacEEE}(i, j, k), k = j + 1 \dots 9), j = i + 1 \dots 9), i = 1 \dots 9) \} \\ &\quad \{0\} \end{aligned} \quad (1.5)$$

$$\begin{aligned} &> \text{JacEEO} := (i, j, k) \rightarrow \text{simplify}(\text{add}(\text{Br}[\text{Ev}[l], \text{Ov}[k]] \cdot eV(\text{Br}[\text{Ev}[i], \text{Ev}[j]])([l], l = 1 \dots 9) \\ &\quad + \text{add}(\text{Br}[\text{Ov}[l], \text{Ev}[i]] \cdot oV(\text{Br}[\text{Ev}[j], \text{Ov}[k]])([l] + \text{Br}[\text{Ov}[l], \text{Ev}[j]] \cdot oV(\text{Br}[\text{Ov}[k], \\ &\quad \text{Ev}[i]])([l], l = 1 \dots 8)) : \\ &\quad \{ \text{seq}(\text{seq}(\text{seq}(\text{JacEEO}(i, j, k), k = 1 \dots 8), j = i + 1 \dots 9), i = 1 \dots 9) \} \\ &\quad \{0\} \end{aligned} \quad (1.6)$$

$$\begin{aligned} &> \text{JacEOO} := (i, j, k) \rightarrow \text{simplify}(\text{add}(\text{Br}[\text{Ov}[l], \text{Ov}[k]] \cdot oV(\text{Br}[\text{Ev}[i], \text{Ov}[j]])([l] - \text{Br}[\text{Ov}[l], \\ &\quad \text{Ov}[j]] \cdot oV(\text{Br}[\text{Ov}[k], \text{Ev}[i]])([l], l = 1 \dots 8) + \text{add}(\text{Br}[\text{Ev}[l], \text{Ev}[i]] \cdot eV(\text{Br}[\text{Ov}[j], \\ &\quad \text{Ov}[k]])([l], l = 1 \dots 9)) : \\ &\quad \{ \text{seq}(\text{seq}(\text{seq}(\text{JacEOO}(i, j, k), k = i \dots 8), j = 1 \dots 8), i = 1 \dots 9) \} \\ &\quad \{0\} \end{aligned} \quad (1.7)$$

$$\begin{aligned} &> \text{JacOOO} := (i, j, k) \rightarrow \text{simplify}(\text{add}(\text{Br}[\text{Ev}[l], \text{Ov}[k]] \cdot eV(\text{Br}[\text{Ov}[i], \text{Ov}[j]])([l] + \text{Br}[\text{Ev}[l], \\ &\quad \text{Ov}[i]] \cdot eV(\text{Br}[\text{Ov}[j], \text{Ov}[k]])([l] + \text{Br}[\text{Ev}[l], \text{Ov}[j]] \cdot eV(\text{Br}[\text{Ov}[k], \text{Ov}[i]])([l], l = 1 \dots 9) \\ &\quad ) : \\ &\quad \text{simplify}(\text{eval}(\{ \text{seq}(\text{seq}(\text{seq}(\text{JacOOO}(i, j, k), k = i \dots 8), j = i \dots 8), i = 1 \dots 8) \}, \{ s3 = -s1 - s2 \})) \\ &\quad \{0\} \end{aligned} \quad (1.8)$$

$$> s1 := -1 - \alpha : s2 := 1 : s3 := \alpha :$$

$$\begin{aligned} &> \text{KFe} := (A, B) \rightarrow \text{add}(\text{add}(eV(\text{Br}[A, \text{Ev}[j]])([i] \cdot eV(\text{Br}[B, \text{Ev}[i]])([j], j = 1 \dots n0), i = 1 \dots n0) \\ &\quad - \text{add}(\text{add}(oV(\text{Br}[A, \text{Ov}[j]])([i] \cdot oV(\text{Br}[B, \text{Ov}[i]])([j], j = 1 \dots n1), i = 1 \dots n1) : \\ &\quad \text{KFo} := (A, B) \rightarrow \text{add}(\text{add}(eV(sBr[A, \text{Ov}[j]])([i] \cdot oV(\text{Br}[B, \text{Ev}[i]])([j], j = 1 \dots n1), i = 1 \dots n0) \\ &\quad - \text{add}(\text{add}(oV(\text{Br}[A, \text{Ev}[j]])([i] \cdot eV(sBr[B, \text{Ov}[i]])([j], j = 1 \dots n0), i = 1 \dots n1) : \end{aligned}$$

$$> \text{me} := (i, j) \rightarrow \text{KFe}(\text{Ev}[i], \text{Ev}[j]) : \text{mo} := (i, j) \rightarrow \text{KFo}(\text{Ov}[i], \text{Ov}[j]) : \text{Matrix}(\text{me}, n0), \\ \text{Matrix}(\text{mo}, n1)$$

$$\left[ \begin{array}{cccccccccc} 0 & 0 & 0 & 0 & 0 & 0 & 0 & 0 & 0 & 0 \\ 0 & 0 & 0 & 0 & 0 & 0 & 0 & 0 & 0 & 0 \\ 0 & 0 & 0 & 0 & 0 & 0 & 0 & 0 & 0 & 0 \\ 0 & 0 & 0 & 0 & 0 & 0 & 0 & 0 & 0 & 0 \\ 0 & 0 & 0 & 0 & 0 & 0 & 0 & 0 & 0 & 0 \\ 0 & 0 & 0 & 0 & 0 & 0 & 0 & 0 & 0 & 0 \\ 0 & 0 & 0 & 0 & 0 & 0 & 0 & 0 & 0 & 0 \\ 0 & 0 & 0 & 0 & 0 & 0 & 0 & 0 & 0 & 0 \\ 0 & 0 & 0 & 0 & 0 & 0 & 0 & 0 & 0 & 0 \\ 0 & 0 & 0 & 0 & 0 & 0 & 0 & 0 & 0 & 0 \end{array} \right], \left[ \begin{array}{cccccccccc} 0 & 0 & 0 & 0 & 0 & 0 & 0 & 0 & 0 & 0 \\ 0 & 0 & 0 & 0 & 0 & 0 & 0 & 0 & 0 & 0 \\ 0 & 0 & 0 & 0 & 0 & 0 & 0 & 0 & 0 & 0 \\ 0 & 0 & 0 & 0 & 0 & 0 & 0 & 0 & 0 & 0 \\ 0 & 0 & 0 & 0 & 0 & 0 & 0 & 0 & 0 & 0 \\ 0 & 0 & 0 & 0 & 0 & 0 & 0 & 0 & 0 & 0 \\ 0 & 0 & 0 & 0 & 0 & 0 & 0 & 0 & 0 & 0 \\ 0 & 0 & 0 & 0 & 0 & 0 & 0 & 0 & 0 & 0 \\ 0 & 0 & 0 & 0 & 0 & 0 & 0 & 0 & 0 & 0 \\ 0 & 0 & 0 & 0 & 0 & 0 & 0 & 0 & 0 & 0 \end{array} \right] \quad (1.9)$$

$$\begin{aligned} &> \text{KFe} := (A, B) \rightarrow \text{add} \left( \text{add} \left( \frac{1}{4s1} eV(\text{Br}[A, \text{Ev}[j]])([i] \cdot eV(\text{Br}[B, \text{Ev}[i]])([j], j = 1 \dots 3) \right), i = 1 \right. \\ &\quad \left. \dots 3 \right) + \text{add} \left( \text{add} \left( \frac{1}{4s2} eV(\text{Br}[A, \text{Ev}[j]])([i] \cdot eV(\text{Br}[B, \text{Ev}[i]])([j], j = 4 \dots 6) \right), i = 4 \dots 6 \right) \end{aligned}$$

$$\begin{aligned}
& + \text{add} \left( \text{add} \left( \frac{1}{4s^3} eV(Br[A, Ev[j]])[i] \cdot eV(Br[B, Ev[i]])(j), j = 7 \dots 9 \right), i = 7 \dots 9 \right) : \\
& me := (i, j) \rightarrow \text{simplify}(KFe(Ev[i], Ev[j])) : \text{Matrix}(me, n0)
\end{aligned}$$

$$\begin{bmatrix}
0 & 0 & \frac{1}{-1-\alpha} & 0 & 0 & 0 & 0 & 0 & 0 \\
0 & -\frac{2}{1+\alpha} & 0 & 0 & 0 & 0 & 0 & 0 & 0 \\
\frac{1}{-1-\alpha} & 0 & 0 & 0 & 0 & 0 & 0 & 0 & 0 \\
0 & 0 & 0 & 0 & 0 & 1 & 0 & 0 & 0 \\
0 & 0 & 0 & 0 & 2 & 0 & 0 & 0 & 0 \\
0 & 0 & 0 & 1 & 0 & 0 & 0 & 0 & 0 \\
0 & 0 & 0 & 0 & 0 & 0 & 0 & 0 & \frac{1}{\alpha} \\
0 & 0 & 0 & 0 & 0 & 0 & 0 & \frac{2}{\alpha} & 0 \\
0 & 0 & 0 & 0 & 0 & 0 & \frac{1}{\alpha} & 0 & 0
\end{bmatrix} \quad (1.10)$$

> for  $il$  from 0 to 1 do for  $j1$  from 0 to 1 do for  $k1$  from 0 to 1 do for  $i2$  from 0 to 1 do for  $j2$  from 0 to 1 do for  $k2$  from 0 to 1 do  $KBr[W[i1, j1, k1], W[i2, j2, k2]] := -\epsilon[i1, i2] \cdot \epsilon[j1, j2] \cdot \epsilon[k1, k2] : \text{od} : \text{od} : \text{od} : \text{od} : \text{od} : \text{od} : KFo := (A, B) \rightarrow \text{add}(\text{add}(KBr[Ov[i], Ov[j]] \cdot oV(A)[i] \cdot oV(B)[j], j = 1 \dots n1), i = 1 \dots n1) : mo := (i, j) \rightarrow KFo(Ov[i], Ov[j]) : \text{Matrix}(mo, n1)$

$$\begin{bmatrix}
0 & 0 & 0 & 0 & 0 & 0 & 0 & -1 \\
0 & 0 & 0 & 0 & 0 & 0 & 1 & 0 \\
0 & 0 & 0 & 0 & 0 & 1 & 0 & 0 \\
0 & 0 & 0 & 0 & -1 & 0 & 0 & 0 \\
0 & 0 & 0 & 1 & 0 & 0 & 0 & 0 \\
0 & 0 & -1 & 0 & 0 & 0 & 0 & 0 \\
0 & -1 & 0 & 0 & 0 & 0 & 0 & 0 \\
1 & 0 & 0 & 0 & 0 & 0 & 0 & 0
\end{bmatrix} \quad (1.11)$$

>  $KFSee := (i, j, k) \rightarrow \text{add}(KFe(Ev[i], Ev[k]) \cdot eV(Br[Ev[i], Ev[j]])(l) - KFe(Ev[i], Ev[l]) \cdot eV(Br[Ev[j], Ev[k]])(l), l = 1 \dots n0) : \{seq(seq(seq(KFSee(i, j, k), k = 1 \dots n0), j = 1 \dots n0), i = 1 \dots n0)\}$

$\{0\}$  (1.12)

>  $KFSeo := (i, j, k) \rightarrow \text{simplify}(\text{add}(KFo(Ov[i], Ov[k]) \cdot oV(Br[Ev[i], Ov[j]])(l), l = 1 \dots n1) - \text{add}(KFe(Ev[i], Ev[l]) \cdot eV(Br[Ov[j], Ov[k]])(l), l = 1 \dots n0)) : \{seq(seq(seq(KFSeo(i, j, k), k = 1 \dots n1), j = 1 \dots n1), i = 1 \dots n0)\}$

$$\{0\} \quad (1.13)$$

$$\begin{aligned} &> KFSoeo := (i, j, k) \rightarrow \text{add}(KFo(Ov[l], Ov[k]) \cdot oV(Br[Ov[i], Ev[j]])(l) - KFo(Ov[i], Ov[l]) \\ &\quad \cdot oV(Br[Ev[j], Ov[k]])(l, l = 1 \dots nl) : \{seq(seq(seq(KFSee(i, j, k), k = 1 \dots nl), j = 1 \\ &\quad \dots n0), i = 1 \dots nl)\} \end{aligned}$$

$$\{0\} \quad (1.14)$$

$$\begin{aligned} &> KFSooe := (i, j, k) \rightarrow \text{simplify}(\text{add}(KFe(Ev[l], Ev[k]) \cdot eV(Br[Ov[i], Ov[j]])(l, l = 1 \dots n0) \\ &\quad - \text{add}(KFo(Ov[i], Ov[l]) \cdot oV(Br[Ov[j], Ev[k]])(l, l = 1 \dots nl)) : \\ &\quad \{seq(seq(seq(KFSooe(i, j, k), k = 1 \dots n0), j = 1 \dots nl), i = 1 \dots nl)\} \end{aligned}$$

$$\{0\} \quad (1.15)$$

$$> Ov$$

$$[W_{0,0,0}, W_{1,0,0}, W_{0,1,0}, W_{1,1,0}, W_{0,0,1}, W_{1,0,1}, W_{0,1,1}, W_{1,1,1}] \quad (1.16)$$

$$> \text{unassign}('k1', 'k2') :$$

$$\begin{aligned} &> RsE := \left[ k1 \cdot X_1, -H_1, \frac{1}{k1} \cdot Y_1, k2 \cdot X_2, -H_2, \frac{1}{k2} \cdot Y_2, -\frac{k3^2}{k1 \cdot k2} \cdot X_3, -H_3, -\frac{k1 \cdot k2}{k3^2} \cdot Y_3 \right] : RsO := \\ &\quad \left[ k3 \cdot W_{1,1,1}, \frac{k3}{k1} \cdot W_{0,1,1}, \frac{k3}{k2} \cdot W_{1,0,1}, \frac{k3}{k1 \cdot k2} \cdot W_{0,0,1}, -\frac{k1 \cdot k2}{k3} \cdot W_{1,1,0}, -\frac{k2}{k3} \cdot W_{0,1,0}, -\frac{k1}{k3} \right. \\ &\quad \left. \cdot W_{1,0,0}, -\frac{1}{k3} \cdot W_{0,0,0} \right] : \end{aligned}$$

$$Te := X \rightarrow \text{simplify}(\text{add}(RsE[i] \cdot eV(X)(i, i = 1 \dots n0)) : To := X \rightarrow \text{simplify}(\text{add}(RsO[i] \cdot oV(X)(i, i = 1 \dots nl)) :$$

$$\begin{aligned} &> chkEE := (i, j) \rightarrow \text{simplify}(\text{add}(\text{add}(Br[Ev[k], Ev[l]] \cdot eV(Te(Ev[i]))(k) \cdot eV(Te(Ev[j]))(l, k \\ &\quad = 1 \dots n0), l = 1 \dots n0) - Te(Br[Ev[i], Ev[j]])) : \{seq(seq(chkEE(i, j), j = i + 1 \dots n0), i = 1 \\ &\quad \dots n0)\} \end{aligned}$$

$$\{0\} \quad (1.17)$$

$$\begin{aligned} &> chkEO := (i, j) \rightarrow \text{simplify}(\text{add}(\text{add}(Br[Ev[k], Ov[l]] \cdot eV(Te(Ev[i]))(k) \cdot oV(To(Ov[j]))(l, k \\ &\quad = 1 \dots n0), l = 1 \dots nl) - To(Br[Ev[i], Ov[j]])) : \{seq(seq(chkEO(i, j), j = 1 \dots nl), i = 1 \\ &\quad \dots n0)\} \end{aligned}$$

$$\{0\} \quad (1.18)$$

$$\begin{aligned} &> chkOO := (i, j) \rightarrow \text{simplify}(\text{add}(\text{add}(Br[Ov[k], Ov[l]] \cdot oV(To(Ov[i]))(k) \\ &\quad \cdot oV(To(Ov[j]))(l, k = 1 \dots nl), l = 1 \dots nl) - Te(Br[Ov[i], Ov[j]])) : \\ &\quad \{seq(seq(chkOO(i, j), j = 1 \dots nl), i = 1 \dots nl)\} \end{aligned}$$

$$\{0\} \quad (1.19)$$

$$\begin{aligned} &> BFe := (A, B) \rightarrow \text{add}(KFe(Ev[i], B) \cdot eV(Te(A))(i, i = 1 \dots n0) : BFo := (A, B) \\ &\quad \rightarrow \text{add}(KFo(Ov[j], B) \cdot oV(To(A))(j, j = 1 \dots nl) : \end{aligned}$$

$$> me := (i, j) \rightarrow \text{simplify}(BFe(Ev[i], Ev[j])) : Me := \text{Matrix}(me, n0)$$

$$Me := \quad (1.20)$$



$$\begin{bmatrix} -\frac{k1}{1+\alpha} & 0 & 0 & 0 & 0 & 0 & 0 & 0 & 0 \\ 0 & \frac{2}{1+\alpha} & 0 & 0 & 0 & 0 & 0 & 0 & 0 \\ 0 & 0 & -\frac{1}{(1+\alpha)k1} & 0 & 0 & 0 & 0 & 0 & 0 \\ 0 & 0 & 0 & k2 & 0 & 0 & 0 & 0 & 0 \\ 0 & 0 & 0 & 0 & -2 & 0 & 0 & 0 & 0 \\ 0 & 0 & 0 & 0 & 0 & \frac{1}{k2} & 0 & 0 & 0 \\ 0 & 0 & 0 & 0 & 0 & 0 & -\frac{k3^2}{\alpha k1 k2} & 0 & 0 \\ 0 & 0 & 0 & 0 & 0 & 0 & 0 & -\frac{2}{\alpha} & 0 \\ 0 & 0 & 0 & 0 & 0 & 0 & 0 & 0 & -\frac{k1 k2}{\alpha k3^2} \end{bmatrix}$$

>  $mo := (i,j) \rightarrow \text{simplify}(B\text{Fo}(Ov[i], Ov[j])) : Mo := \text{Matrix}(mo, n1)$

$$Mo := \begin{bmatrix} k3 & 0 & 0 & 0 & 0 & 0 & 0 & 0 \\ 0 & -\frac{k3}{k1} & 0 & 0 & 0 & 0 & 0 & 0 \\ 0 & 0 & -\frac{k3}{k2} & 0 & 0 & 0 & 0 & 0 \\ 0 & 0 & 0 & \frac{k3}{k1 k2} & 0 & 0 & 0 & 0 \\ 0 & 0 & 0 & 0 & \frac{k1 k2}{k3} & 0 & 0 & 0 \\ 0 & 0 & 0 & 0 & 0 & -\frac{k2}{k3} & 0 & 0 \\ 0 & 0 & 0 & 0 & 0 & 0 & -\frac{k1}{k3} & 0 \\ 0 & 0 & 0 & 0 & 0 & 0 & 0 & \frac{1}{k3} \end{bmatrix}$$

(1.21)

>  $RsE := [-X_1, -H_1, -Y_1, -X_2, -H_2, -Y_2, -X_3, -H_3, -Y_3] : RsO := [W_{1,1,1}, -W_{0,1,1}, -W_{1,0,1}, W_{0,0,1}, -W_{1,1,0}, W_{0,1,0}, W_{1,0,0}, -W_{0,0,0}] :$

$Te := X \rightarrow \text{simplify}(\text{add}(RsE[i] \cdot eV(X)[i], i = 1..n0)) : To := X \rightarrow \text{simplify}(\text{add}(RsO[i] \cdot oV(X)[i], i = 1..n1)) :$

>  $BFe := (A, B) \rightarrow add(KFe(Ev[i], B) \cdot eV(To(A))[i], i = 1 \dots n0) : BFo := (A, B)$   
 $\rightarrow add(KFo(Ov[j], B) \cdot oV(To(A))[j], j = 1 \dots n1) :$   
>  $me := (i, j) \rightarrow simplify(BFe(Ev[i], Ev[j])) : Me := simplify(Matrix(me, n0))$

$$Me := \begin{bmatrix} \frac{1}{1+\alpha} & 0 & 0 & 0 & 0 & 0 & 0 & 0 & 0 \\ 0 & \frac{2}{1+\alpha} & 0 & 0 & 0 & 0 & 0 & 0 & 0 \\ 0 & 0 & \frac{1}{1+\alpha} & 0 & 0 & 0 & 0 & 0 & 0 \\ 0 & 0 & 0 & -1 & 0 & 0 & 0 & 0 & 0 \\ 0 & 0 & 0 & 0 & -2 & 0 & 0 & 0 & 0 \\ 0 & 0 & 0 & 0 & 0 & -1 & 0 & 0 & 0 \\ 0 & 0 & 0 & 0 & 0 & 0 & -\frac{1}{\alpha} & 0 & 0 \\ 0 & 0 & 0 & 0 & 0 & 0 & 0 & -\frac{2}{\alpha} & 0 \\ 0 & 0 & 0 & 0 & 0 & 0 & 0 & 0 & -\frac{1}{\alpha} \end{bmatrix} \quad (1.22)$$

>  $mo := (i, j) \rightarrow simplify(BFo(Ov[i], Ov[j])) : Mo := Matrix(mo, n1)$

$$Mo := \begin{bmatrix} 1 & 0 & 0 & 0 & 0 & 0 & 0 & 0 \\ 0 & 1 & 0 & 0 & 0 & 0 & 0 & 0 \\ 0 & 0 & 1 & 0 & 0 & 0 & 0 & 0 \\ 0 & 0 & 0 & 1 & 0 & 0 & 0 & 0 \\ 0 & 0 & 0 & 0 & 1 & 0 & 0 & 0 \\ 0 & 0 & 0 & 0 & 0 & 1 & 0 & 0 \\ 0 & 0 & 0 & 0 & 0 & 0 & 1 & 0 \\ 0 & 0 & 0 & 0 & 0 & 0 & 0 & 1 \end{bmatrix} \quad (1.23)$$

>  $sgn1 := i \rightarrow \frac{sign(i) - sign(-i)}{2} :$

>  $sgn2 := (i, j) \rightarrow 1 - \frac{\left(sign\left(n0 + \frac{1}{2} - i\right) - 1\right) \cdot \left(sign\left(n0 + \frac{1}{2} - j\right) - 1\right)}{2} :$

>  $sg1 := i \rightarrow sign\left(n0 + \frac{1}{2} - i\right) : sg2 := (i, j) \rightarrow sign\left(n0 + \frac{1}{2} - i\right) \cdot sign\left(n0 + \frac{1}{2} - j\right) :$   
 $sg3 := (i, j, k) \rightarrow sign\left(n0 + \frac{1}{2} - i\right) \cdot sign\left(n0 + \frac{1}{2} - j\right) \cdot sign\left(n0 + \frac{1}{2} - k\right) :$

```

> Par0 := proc(S) local p, q, r; r := 0 : p := 0 : q := 0 : for i to nops(S) do for j to nops(C0)
do if diff(S[i], Cc0[j]) ≠ 0 then r := sg1(C0[j][2]) : fi: od: if r = 1 then p := p + 1
else q := q + 1 : fi: od: [ p, q]; end proc:
Par1 := proc(S) local p, q, r; r := 0 : p := 0 : q := 0 : for i to nops(S) do for j to nops(C1)
do if diff(S[i], Cc1[j]) ≠ 0 then r := sg2(C1[j][2], C1[j][3]) : fi: od: if r = 1 then p :=
p + 1 else q := q + 1 : fi: od: [ p, q]; end proc:
Par2 := proc(S) local p, q, r; r := 0 : p := 0 : q := 0 : for i to nops(S) do for j to nops(C2)
do if diff(S[i], Cc2[j]) ≠ 0 then r := sg3(C2[j][2], C2[j][3], C2[j][4]) : fi: od: if r = 1
then p := p + 1 else q := q + 1 : fi: od: [ p, q]; end proc:
# m1 := {1, 10, 12, 14, 16} : m2 := {1, 4, 10, 14} : m3 := {4, 12, 16} : m4 := {4, 7, 12, 14} :
m5 := {4, 7, 16} : m6 := {10, 11, 12, 14} :
# (List of all parabolics : the first five are for DDI namely m1, m2, m12, m23, m123,
and the last one is the Borel for DDIV.)

```

## Complex $C^*(m, g)$ for $m=m1=g[-]$ corresponding to $p[1]$ of DD-I

```

> m1 := {1, 10, 12, 14, 16} : m10 := {1} : m11 := {10, 12, 14, 16} :
d[1] := -2 : d[2] := 0 : d[3] := 2 : d[4] := 0 : d[5] := 0 : d[6] := 0 : d[7] := 0 : d[8] :=
0 : d[9] := 0 : d[10] := -1 : d[11] := 1 : d[12] := -1 : d[13] := 1 : d[14] := -1 :
d[15] := 1 : d[16] := -1 : d[17] := 1 :
> Cc0 := [seq(e[i], i = 1..N)] : Cc1 := [seq(seq(e[i, j], j in m1), i = 1..N)] : Cc2 :=
[op({seq(seq(seq(e[i, j, k], k in m1), j in m1), i = 1..N)} \ {seq(seq(e[i, j, j], j = 1..n0), i
= 1..N), seq(seq(seq(e[i, j, k], k = 1..j-1), j = 1..N), i = 1..N)})] :
> C0 := [seq([e[i], i], i = 1..N)] : C1 := [seq(seq([e[i, j], i, j], j in m1), i = 1..N)] : C2 :=
[op({seq(seq(seq([e[i, j, k], i, j, k], k in m1), j in m1), i = 1..N)} \ {seq(seq([e[i, j, j], i, j,
j], j = 1..n0), i = 1..N), seq(seq(seq([e[i, j, k], i, j, k], k = 1..j-1), j = 1..N), i = 1..N)})] :
> for i to N do de[i] := add(add(c[i, j, k] e[k, j], j in m1), k = 1..N) : od:
for k in m1 do dθ[k] := eval( add( add( - 1/2 c[i, j, k] θ[i, j], j in m1 ), i in m1 ),
{seq(seq(θ[j, i] = -θ[i, j], j = i+1..N), i = 1..n0), seq(θ[j, j] = 0, j = 1..n0),
seq(seq(θ[j, i] = θ[i, j], j = i+1..N), i = n0+1..N)}) : od:
> cC0 := add(c[i] e[i], i = 1..N) : dC0 := collect(expand(add(c[i] de[i], i = 1..N)), Cc1) :
> sl0 := solve({coeffs(dC0, Cc1)}, {seq(c[i], i = 1..N)}) : eval(cC0, sl0)
c1 e1 (1.1.1)
> Par0([e1]), [d[1]]
[1, 0], [-2] (1.1.2)
> bl0 := factor(Basis([coeffs(dC0, Cc1)], plex(α, seq(c[i], i = 1..N)))) : slb0 :=
solve({op(bl0), α ≠ -1})
bl0 := [c17, c15, c13, c11, c9, c8, c7, c6, c5, c4, c3, c2, c16 (1 + α), c14 (1 + α), c12 (1 + α),
c10 (1 + α)]
slb0 := {α = α, c2 = 0, c3 = 0, c4 = 0, c5 = 0, c6 = 0, c7 = 0, c8 = 0, c9 = 0, c10 = 0, c11 = 0, c12
= 0, c13 = 0, c14 = 0, c15 = 0, c16 = 0, c17 = 0} (1.1.3)

```

$$\begin{aligned} &> \text{eval}(cC0, slb0) \\ &\qquad\qquad\qquad c_1 e_1 \end{aligned} \tag{1.1.4}$$

$$\begin{aligned} &> Cf0 := \{ \} : \text{for } i \text{ to } nops(sl0) \text{ do if } lhs(sl0[i]) = rhs(sl0[i]) \text{ then } Cf0 := \{ op(Cf0), \\ &\quad lhs(sl0[i]) \} : \text{fi:od:} \\ &b0 := 0 : z0 := nops(Cf0) : d0 := nops(C0) : \\ &dim(B0) = b0, dim(Z0) = z0, dim(H0) = z0 - b0 \\ &\qquad\qquad\qquad dim(B0) = 0, dim(Z0) = 1, dim(H0) = 1 \end{aligned} \tag{1.1.5}$$

$$\begin{aligned} &> \text{for } i \text{ to } N \text{ do for } j \text{ in } m1 \text{ do } de[i, j] := \text{eval} \left( \text{add}(\text{add}(c[i, l, k] e[k, l, j], l \text{ in } m1), k = 1 .. N) \right. \\ &\quad \left. + \frac{1}{2} \text{add}(\text{add}(c[k, l, j] e[i, k, l], l \text{ in } m1), k \text{ in } m10) + \frac{1}{2} \text{add}(\text{add}(c[k, l, j] e[i, k, l], l \right. \\ &\quad \left. \text{in } m10), k \text{ in } m11) - \frac{1}{2} \text{add}(\text{add}(c[k, l, j] e[i, k, l], l \text{ in } m11), k \text{ in } m11), sbs1) \right) : \text{od:od:} \\ &> seq(\text{simplify}(\text{add}(\text{diff}(de[j], Cc1[i]) \cdot d \parallel (Cc1[i]), i = 1 .. nops(Cc1))), j = 1 .. nops(Cc0)) \\ &\qquad\qquad\qquad 0, 0, 0, 0, 0, 0, 0, 0, 0, 0, 0, 0, 0, 0, 0, 0, 0 \end{aligned} \tag{1.1.6}$$

$$\begin{aligned} &> cC1 := \text{add}(cc[op(C1[i][2..3])] C1[i, 1], i = 1 .. nops(C1)) : dC1 := \text{expand}(\text{add} \\ &\quad (cc[op(C1[i][2..3])] \cdot d \parallel (C1[i, 1]), i = 1 .. nops(C1))) : \\ &b11 := \text{Basis}([coeffs(dC1, Cc2)], \text{plex}(\alpha, seq(cc[op(C1[i][2..3])], i = 1 .. nops(C1)))) : \\ &s11a := \text{solve}(\{op(b11), \alpha \neq 0, \alpha \neq -1\}) : \\ &s11 := \text{solve}(\{op(b11), \alpha \neq 0, \alpha \neq -1\}, \{\alpha, seq(cc[op(C1[i][2..3])], i = 1 .. nops(C1))\}) : nops(\{s11a\}), nops(\{s11\}); \\ &Cf1 := \{ \} : \text{for } i \text{ to } nops(s11) \text{ do if } lhs(s11[i]) = rhs(s11[i]) \text{ then } Cf1 := \{ op(Cf1), \\ &\quad lhs(s11[i]) \} : \text{fi:od: } Cf1 \\ &\qquad\qquad\qquad 1, 1 \end{aligned}$$

$$\begin{aligned} &\{ \alpha, cc_{1, 10}, cc_{1, 12}, cc_{1, 14}, cc_{1, 16}, cc_{8, 10}, cc_{8, 12}, cc_{8, 14}, cc_{8, 16}, cc_{10, 1}, cc_{12, 1}, cc_{12, 12}, cc_{12, 16}, cc_{14, 1}, \\ &\quad cc_{14, 14}, cc_{14, 16}, cc_{16, 1}, cc_{16, 12}, cc_{16, 14}, cc_{16, 16}, cc_{17, 16} \} \end{aligned} \tag{1.1.7}$$

$$\begin{aligned} &> Cf1 := Cf1 \setminus \{ \alpha \} : \\ &> \text{Basis}([coeffs(\text{expand}(\text{subs}(s11a, cC1) - dC0), Cc1)], \text{plex}(\alpha, seq(cc[op(C1[i][2..3])], i = 1 \\ &\quad .. nops(C1)), seq(c[i], i = 1 .. N))) : \text{solve}(\%, \{ seq(c[i], i = 1 .. N) \}) \\ &[-c_3 + cc_{17, 16} cc_{16, 16} + c_2 - c_5 - c_8, cc_{16, 14} - c_6, cc_{16, 12} - c_9, cc_{16, 1} + c_{17}, cc_{14, 16} - c_4, cc_{14, 14} \\ &\quad + c_2 + c_5 - c_8, cc_{14, 1} + c_{15}, cc_{12, 16} - c_7, cc_{12, 12} + c_2 - c_5 + c_8, cc_{12, 1} + c_{13}, cc_{10, 1} + c_{11}, \\ &\quad cc_{8, 14} c_{11} + c_{13} cc_{8, 16}, cc_{8, 12} c_{13} + c_{15} cc_{8, 14}, cc_{8, 12} c_{11} - c_{15} cc_{8, 16}, cc_{8, 10} c_{15} + c_{17} cc_{8, 12}, \\ &\quad cc_{8, 10} c_{13} - c_{17} cc_{8, 14}, cc_{8, 10} c_{11} + c_{17} cc_{8, 16}, c_{10} c_{17} + 2 cc_{8, 10} c_{10} + cc_{1, 16} c_{17}, c_{10} c_{15} \\ &\quad - 2 cc_{8, 12} c_{10} + cc_{1, 16} c_{15}, c_{10} c_{13} + 2 cc_{8, 14} c_{10} + cc_{1, 16} c_{13}, c_{10} c_{11} - 2 cc_{8, 16} c_{10} \\ &\quad + cc_{1, 16} c_{11}, -c_{12} c_{17} - 2 cc_{8, 10} c_{12} + cc_{1, 14} c_{17}, -c_{12} c_{15} + 2 cc_{8, 12} c_{12} + cc_{1, 14} c_{15}, \\ &\quad -c_{12} c_{13} - 2 cc_{8, 14} c_{12} + cc_{1, 14} c_{13}, -c_{11} c_{12} + cc_{1, 14} c_{11} + 2 c_{12} cc_{8, 16}, cc_{1, 14} c_{10} \\ &\quad + c_{12} cc_{1, 16}, -c_{14} c_{17} - 2 cc_{8, 10} c_{14} + cc_{1, 12} c_{17}, -c_{14} c_{15} + 2 cc_{8, 12} c_{14} + cc_{1, 12} c_{15}, \\ &\quad -c_{13} c_{14} + cc_{1, 12} c_{13} - 2 c_{14} cc_{8, 14}, cc_{1, 12} c_{12} - c_{14} cc_{1, 14}, -c_{11} c_{14} + cc_{1, 12} c_{11} \end{aligned} \tag{1.1.8}$$



```

> mlt2 := { } :for j in m1 do for k in m1 do if k > j or (k=j and j in m11) then mlt2 :=
  {op(mlt2), [j, k]} :fi:od:od:
mlt3 := { } :for j in m1 do for k in m1 do for l in m1 do if (k > j and l > k) or (k=j and j
  in m11 and l ≥ k) or (l=k and k in m11 and j < k) then mlt3 := {op(mlt3), [j, k, l]} :
  fi:od:od:od:
> Cc2 := { } :for i to N do for j in m1 do for k in m1 do if [j, k] in mlt2 then Cc2 :=
  {op(Cc2), e[i, j, k]} :fi:od:od:od: Cc2 := [op(Cc2)] :
Cc3 := { } :for i to N do for j in m1 do for k in m1 do for l in m1 do if [j, k, l] in mlt3
  then Cc3 := {op(Cc3), e[i, j, k, l]} :fi:od:od:od:od: Cc3 := [op(Cc3)] :
> cC2 := add(cc[op(C2[i][2..4])] C2[i, 1], i = 1..nops(C2)) : dC2 := expand(add
  (cc[op(C2[i][2..4])]·d|| (C2[i, 1]), i = 1..nops(C2))) :
sl2 := solve({coeffs(dC2, Cc3)}, {seq(cc[op(C2[i][2..4])], i = 1..nops(C2))}) : Cf2 := { } :
  for i to nops(sl2) do if lhs(sl2[i]) = rhs(sl2[i]) then Cf2 := {op(Cf2), lhs(sl2[i])} :fi:
  od:
eliminate({coeffs(expand(subs(sl2, cC2) - dC1), Cc2)}, Cf2) : %[2], nops(%[1]),
  nops(Cf2)

```

$\emptyset, 74, 74$  (1.1.12)

```

> tmp := eliminate({coeffs(expand(subs(sl2, cC2) - dC1), Cc2)}, {seq(cc[op(C1[i][2..3])], i
  = 1..nops(C1))}) :
tmss := solve(tmp[2]) : ltm := [ ] : for i to nops(tmss) do if lhs(tmss[i]) ≠ rhs(tmss[i])
  then ltm := [op(ltm), lhs(tmss[i])] :fi:od: ltm : Coh2 := {seq(diff(cC2, ltm[i]), i = 1
  ..nops(ltm))} :
deg2 := [ ] :for i to nops(Coh2) do for j to nops(Cc2) do if diff(Cc2[j], Coh2[i]) ≠ 0
  then deg2 := [op(deg2), d[C2[j][2]] - d[C2[j][3]] - d[C2[j][4]]] :fi:od:od: deg2:
b2 := d1 - z1 : z2 := nops(Cf2) : d2 := nops(C2) : dim(B2) = b2, dim(Z2) = z2, dim(H2)
  = z2 - b2
Coh2 := {e8, 10, 10, e8, 10, 12, e8, 10, 14, e8, 10, 16, e8, 12, 12, e8, 12, 16, e8, 14, 14, e8, 14, 16, e8, 16, 16}
  [2, 2, 2, 2, 2, 2, 2, 2, 2]
dim(B2) = 65, dim(Z2) = 74, dim(H2) = 9

```

(1.1.13)

```

> Par2([e8, 10, 10, e8, 10, 12, e8, 10, 14, e8, 10, 16, e8, 12, 12, e8, 12, 16, e8, 14, 14, e8, 14, 16, e8, 16, 16])
  [9, 0]

```

(1.1.14)

H2 is supported in homogeneity 2 (contact projective Weyl tensor: 9 components)

## Complex C\*(m,g) for m=m2=g[-] corresponding to p[2] of DD-I

```

> m1 := {1, 4, 10, 14} : m10 := {1, 4} : m11 := {10, 14} :
d[1] := -1 : d[2] := 0 : d[3] := 1 : d[4] := -1 : d[5] := 0 : d[6] := 1 : d[7] := 0 :
d[8] := 0 : d[9] := 0 : d[10] := -1 : d[11] := 0 : d[12] := 0 : d[13] := 1 : d[14] :=
  -1 : d[15] := 0 : d[16] := 0 : d[17] := 1 :
> Cc0 := [seq(e[i], i = 1..N)] : Cc1 := [seq(seq(e[i, j], j in m1), i = 1..N)] : Cc2 :=
  [op({seq(seq(seq(e[i, j, k], k in m1), j in m1), i = 1..N)} \ {seq(seq(e[i, j, j], j = 1..n0), i
  = 1..N), seq(seq(seq(e[i, j, k], k = 1..j-1), j = 1..N), i = 1..N)})] :
> C0 := [seq([e[i], i], i = 1..N)] : C1 := [seq(seq([e[i, j], i, j], j in m1), i = 1..N)] : C2 :=
  [op({seq(seq(seq([e[i, j, k], i, j, k], k in m1), j in m1), i = 1..N)} \ {seq(seq([e[i, j, j], i, j,
  j], j = 1..n0), i = 1..N), seq(seq(seq([e[i, j, k], i, j, k], k = 1..j-1), j = 1..N), i = 1..N)})]

```

```

]:
> for i to N do de[i] := add(add(c[i,j,k] e[k,j], j in m1), k = 1 ..N) :od:
for k in m1 do dθ[k] := eval( add( add( - 1/2 c[i,j,k] θ[i,j], j in m1 ), i in m1 ),
    {seq(seq(θ[j,i] = -θ[i,j], j = i + 1 ..N), i = 1 ..n0), seq(θ[j,j] = 0, j = 1 ..n0),
    seq(seq(θ[j,i] = θ[i,j], j = i + 1 ..N), i = n0 + 1 ..N) } ) :od:
> cC0 := add(c[i] e[i], i = 1 ..N) : dC0 := collect(expand(add(c[i] de[i], i = 1 ..N)), Cc1) :
> sl0 := solve( {coeffs(dC0, Cc1)}, {seq(c[i], i = 1 ..N)} ) : eval(cC0, sl0)
    c1 e1 + c4 e4 + c10 e10 + c14 e14 (1.2.1)

```

```

> Par0( [e1, e4, e10, e14] ), [d[1], d[4], d[10], d[14]]
    [2, 2], [-1, -1, -1, -1] (1.2.2)

```

```

> bl0 := factor( Basis( [coeffs(dC0, Cc1)], plex(α, seq(c[i], i = 1 ..N)) ) ); slb0 :=
    solve( {op(bl0), α ≠ -1} )
    bl0 := [c17, c16, c15, c13, c12, c11, c9, c8, c7, c6, c5, c3, c2]
slb0 := {α = α, c2 = 0, c3 = 0, c5 = 0, c6 = 0, c7 = 0, c8 = 0, c9 = 0, c11 = 0, c12 = 0, c13 = 0, c15
    = 0, c16 = 0, c17 = 0} (1.2.3)

```

```

> eval(cC0, slb0)
    c1 e1 + c4 e4 + c10 e10 + c14 e14 (1.2.4)

```

```

> Cf0 := { } :for i to nops(sl0) do if lhs(sl0[i]) = rhs(sl0[i]) then Cf0 := {op(Cf0),
    lhs(sl0[i])} :fi:od:
b0 := 0 : z0 := nops(Cf0) : d0 := nops(C0) :
dim(B0) = b0, dim(Z0) = z0, dim(H0) = z0 - b0
    dim(B0) = 0, dim(Z0) = 4, dim(H0) = 4 (1.2.5)

```

```

> for i to N do for j in m1 do de[i,j] := eval( add( add( c[i,l,k] e[k,l,j], l in m1 ), k = 1 ..N)
    + 1/2 add( add( c[k,l,j] e[i,k,l], l in m1 ), k in m10 ) + 1/2 add( add( c[k,l,j] e[i,k,l], l
    in m10 ), k in m11 ) - 1/2 add( add( c[k,l,j] e[i,k,l], l in m11 ), k in m11 ), sbs1 ) :od:od:
> seq(simplify( add( diff( de[j], Cc1[i]) · d || ( Cc1[i] ), i = 1 ..nops(Cc1) ), j = 1 ..nops(Cc0) )
    0, 0, 0, 0, 0, 0, 0, 0, 0, 0, 0, 0, 0, 0, 0, 0 (1.2.6)

```

```

> cC1 := add(cc[op(CI[i][2..3])] CI[i,1], i = 1 ..nops(CI)) : dC1 := expand( add
    (cc[op(CI[i][2..3])] · d || (CI[i,1]), i = 1 ..nops(CI)) ) :
b11 := Basis( [coeffs(dC1, Cc2)], plex(α, seq(cc[op(CI[i][2..3])], i = 1 ..nops(CI)) ) ) :
s11a := solve( {op(b11), α ≠ 0, α ≠ -1} ) :
s11 := solve( {op(b11), α ≠ 0, α ≠ -1}, {α, seq(cc[op(CI[i][2..3])], i = 1 ..nops(CI))
    } ) : nops( {s11a} ), nops( {s11} );
Cf1 := { } :for i to nops(s11) do if lhs(s11[i]) = rhs(s11[i]) then Cf1 := {op(Cf1),
    lhs(s11[i])} :fi:od: Cf1
    1, 1

```

(1.2.7)

$$\{\alpha, cc_{1,1}, cc_{1,4}, cc_{1,10}, cc_{1,14}, cc_{4,1}, cc_{4,4}, cc_{4,10}, cc_{4,14}, cc_{5,10}, cc_{5,14}, cc_{10,1}, cc_{10,4}, cc_{10,10}, cc_{10,14}, cc_{14,1}, cc_{14,4}, cc_{14,10}, cc_{14,14}, cc_{15,14}, cc_{16,14}\} \quad (1.2.7)$$

>  $Cfl := Cfl \setminus \{\alpha\} :$

>  $Basis([coeffs(expand(subs(slla, cCl) - dC0), CcI)], plex(\alpha, seq(cc[op(CI[i][2..3]]), i = 1 .. nops(CI))), seq(c[i], i = 1 .. N))]; solve(%, \{seq(c[i], i = 1 .. N)\})$

$$[cc_{16,14} - c_6, cc_{15,14} - c_3, cc_{14,14} + c_2 + c_5 - c_8, cc_{14,10} - c_9, c_{16} + cc_{14,4}, cc_{14,1} + c_{15}, cc_{10,14} - c_7, c_2 + c_5 + c_8 + cc_{10,10}, c_{12} + cc_{10,4}, cc_{10,1} + c_{11}, 2cc_{5,14} + c_{13}, 2cc_{5,10} - c_{17}, cc_{4,14} + c_{11}, cc_{4,10} - c_{15}, 2c_5 + cc_{4,4}, cc_{4,1}, cc_{1,10}, c_{12} + c_{16}, cc_{1,14}, cc_{1,4}, cc_{1,1} + 2c_2, c_{16}\alpha + c_{16} + cc_{1,10}, c_{12}\alpha + c_{12} - cc_{1,14}] \quad (1.2.8)$$

>  $tmp := eliminate(\{coeffs(expand(subs(sll, cCl) - dC0), CcI)\}, \{seq(c[i], i = 1 .. N)\}) :$   
 $tmss := solve(tmp[2]) : ltm := [] : \text{for } i \text{ to } nops(tmss) \text{ do if } lhs(tmss[i]) \neq rhs(tmss[i])$   
 $\text{then } ltm := [op(ltm), lhs(tmss[i])] : \text{fi:od: } ltm : CohI := \{seq(diff(cCl, ltm[i]), i = 1 .. nops(ltm))\};$   
 $degI := [] : \text{for } i \text{ to } nops(CohI) \text{ do for } j \text{ to } nops(CcI) \text{ do if } diff(CcI[j], CohI[i]) \neq 0$   
 $\text{then } degI := [op(degI), d[CI[j][2]] - d[CI[j][3]]] : \text{fi:od:od: } degI;$   
 $bI := d0 - z0 : zI := nops(Cfl) : dI := nops(CI) : dim(BI) = bI, dim(ZI) = zI, dim(HI)$   
 $= zI - bI$

$$CohI := \{e_{1,1}, e_{1,4}, e_{1,10}, e_{1,14}, e_{4,1}, e_{4,10}, e_{4,14}\}$$

$$[0, 0, 0, 0, 0, 0, 0]$$

$$dim(BI) = 13, dim(ZI) = 20, dim(HI) = 7 \quad (1.2.9)$$

>  $tmp[2]$

$$\{cc_{1,4}, cc_{4,1}, cc_{4,10} + cc_{14,1}, -cc_{10,1} + cc_{4,14}, -2cc_{14,14} + 2cc_{1,1} + 2cc_{4,4} - 2cc_{10,10}, cc_{14,4}\alpha - cc_{1,10} + cc_{14,4}, cc_{10,4}\alpha + cc_{1,14} + cc_{10,4}\} \quad (1.2.10)$$

>  $ParI([e_{1,1}, e_{1,4}, e_{1,10}, e_{1,14}, e_{4,1}, e_{4,10}, e_{4,14}])$   
 $[3, 4]$

$$(1.2.11)$$

H1 is supported in homogeneity 0 (structure reduction)

> **for**  $i$  **to**  $N$  **do** **for**  $j$  **in**  $mI$  **do** **for**  $k$  **in**  $mI$  **do** **if**  $k > j$  **or**  $(k = j \text{ and } j \text{ in } mI1)$  **then**  $de[i, j, k] :=$   
 $eval\left( add(add(c[i, q, p] e[p, q, j, k], q \text{ in } mI), p = 1 .. N) + \frac{1}{2} add(add(c[p, q, j] e[i, p,$   
 $q, k], q \text{ in } mI), p \text{ in } mI0) + \frac{1}{2} add(add(c[p, q, j] e[i, p, q, k], q \text{ in } mI0), p \text{ in } mI1)$   
 $- \frac{1}{2} add(add(c[p, q, j] e[i, p, q, k], q \text{ in } mI1), p \text{ in } mI1) - \frac{1}{2} add(add(c[p, q, k] e[i,$   
 $j, p, q], q \text{ in } mI), p \text{ in } mI0) - \frac{1}{2} add(add(c[p, q, k] e[i, j, p, q], q \text{ in } mI0), p \text{ in } mI1)$   
 $+ \frac{1}{2} add(add(c[p, q, k] e[i, j, p, q], q \text{ in } mI1), p \text{ in } mI1), sbs2 \right) : \text{fi:od:od:od:}$

>  $seq(seq(simplify(add(diff(de[j, k], Cc2[i]) \cdot d[(Cc2[i]), i = 1 .. nops(Cc2)])), j = 1 .. N), k = 1 .. N)$

$$(1.2.12)$$





$$\begin{aligned} & \text{Par2}([e_{8,1,4}, e_{8,1,10}, e_{8,1,14}, e_{8,4,10}, e_{8,4,14}, e_{8,10,10}, e_{8,14,14}, e_{9,14,14}]) \\ & \quad [4, 4] \end{aligned} \quad (1.2.16)$$

H2 is supported in homogeneity 2, dim=(4|4)

>

## Complex $C^*(m,g)$ for $m=m_3=g[-]$ corresponding to p[12] of DD-I

$$\begin{aligned} & \text{m1} := \{1, 4, 10, 12, 14, 16\} : \text{m10} := \{1, 4\} : \text{m11} := \{10, 12, 14, 16\} : \\ & d[1] := -3 : d[2] := 0 : d[3] := 3 : d[4] := -1 : d[5] := 0 : d[6] := 1 : d[7] := 0 : \\ & d[8] := 0 : d[9] := 0 : d[10] := -2 : d[11] := 1 : d[12] := -1 : d[13] := 2 : d[14] := \\ & -2 : d[15] := 1 : d[16] := -1 : d[17] := 2 : \\ & \text{Cc0} := [\text{seq}(e[i], i = 1..N)] : \text{Cc1} := [\text{seq}(\text{seq}(e[i,j], j \text{ in } m1), i = 1..N)] : \text{Cc2} := \\ & [\text{op}(\{\text{seq}(\text{seq}(\text{seq}(e[i,j,k], k \text{ in } m1), j \text{ in } m1), i = 1..N)\} \setminus \{\text{seq}(\text{seq}(e[i,j,j], j = 1..n0), i \\ & = 1..N), \text{seq}(\text{seq}(\text{seq}(e[i,j,k], k = 1..j-1), j = 1..N), i = 1..N)\})] : \\ & \text{C0} := [\text{seq}([e[i], i], i = 1..N)] : \text{C1} := [\text{seq}(\text{seq}([e[i,j], i,j], j \text{ in } m1), i = 1..N)] : \text{C2} := \\ & [\text{op}(\{\text{seq}(\text{seq}(\text{seq}([e[i,j,k], i,j,k], k \text{ in } m1), j \text{ in } m1), i = 1..N)\} \setminus \{\text{seq}(\text{seq}([e[i,j,j], i,j, \\ & j], j = 1..n0), i = 1..N), \text{seq}(\text{seq}(\text{seq}([e[i,j,k], i,j,k], k = 1..j-1), j = 1..N), i = 1..N)\})] : \\ & \text{for } i \text{ to } N \text{ do } de[i] := \text{add}(\text{add}(c[i,j,k] e[k,j], j \text{ in } m1), k = 1..N) : \text{od} : \\ & \text{for } k \text{ in } m1 \text{ do } d\theta[k] := \text{eval}\left(\text{add}\left(\text{add}\left(-\frac{1}{2} c[i,j,k] \theta[i,j], j \text{ in } m1\right), i \text{ in } m1\right), \right. \\ & \quad \left. \{\text{seq}(\text{seq}(\theta[j,i] = -\theta[i,j], j = i+1..N), i = 1..n0), \text{seq}(\theta[j,j] = 0, j = 1..n0), \right. \\ & \quad \left. \text{seq}(\text{seq}(\theta[j,i] = \theta[i,j], j = i+1..N), i = n0+1..N)\} \right) : \text{od} : \\ & \text{cC0} := \text{add}(c[i] e[i], i = 1..N) : \text{dC0} := \text{collect}(\text{expand}(\text{add}(c[i] de[i], i = 1..N)), \text{Cc1}) : \\ & \text{sl0} := \text{solve}(\{\text{coeffs}(\text{dC0}, \text{Cc1})\}, \{\text{seq}(c[i], i = 1..N)\}) : \text{eval}(\text{cC0}, \text{sl0}) \end{aligned} \quad (1.3.1)$$

$$\begin{aligned} & \text{Par0}([e_1]), [d[1]] \\ & \quad [1, 0], [-3] \end{aligned} \quad (1.3.2)$$

$$\begin{aligned} & \text{bl0} := \text{factor}(\text{Basis}([\text{coeffs}(\text{dC0}, \text{Cc1})], \text{plex}(\alpha, \text{seq}(c[i], i = 1..N)))) : \text{slb0} := \\ & \text{solve}(\{\text{op}(\text{bl0}), \alpha \neq -1\}) \\ & \text{bl0} := [c_{17}, c_{16}, c_{15}, c_{13}, c_{12}, c_{11}, c_9, c_8, c_7, c_6, c_5, c_4, c_3, c_2, c_{14} (1 + \alpha), c_{10} (1 + \alpha)] \\ & \text{slb0} := \{\alpha = \alpha, c_2 = 0, c_3 = 0, c_4 = 0, c_5 = 0, c_6 = 0, c_7 = 0, c_8 = 0, c_9 = 0, c_{10} = 0, c_{11} = 0, c_{12} \\ & = 0, c_{13} = 0, c_{14} = 0, c_{15} = 0, c_{16} = 0, c_{17} = 0\} \end{aligned} \quad (1.3.3)$$

$$\begin{aligned} & \text{eval}(\text{cC0}, \text{slb0}) \\ & \quad c_1 e_1 \end{aligned} \quad (1.3.4)$$

$$\begin{aligned} & \text{Cf0} := \{\} : \text{for } i \text{ to } \text{nops}(\text{sl0}) \text{ do if } \text{lhs}(\text{sl0}[i]) = \text{rhs}(\text{sl0}[i]) \text{ then } \text{Cf0} := \{\text{op}(\text{Cf0}), \\ & \quad \text{lhs}(\text{sl0}[i])\} : \text{fi} : \text{od} : \\ & b0 := 0 : z0 := \text{nops}(\text{Cf0}) : d0 := \text{nops}(\text{C0}) : \\ & \text{dim}(B0) = b0, \text{dim}(Z0) = z0, \text{dim}(H0) = z0 - b0 \\ & \quad \text{dim}(B0) = 0, \text{dim}(Z0) = 1, \text{dim}(H0) = 1 \end{aligned} \quad (1.3.5)$$



H1 is supported in homogeneity -2 (even cont outer derivation 4->1) and +1 (higher order reduction)

[illegible]

```

> Cc2 := { } :for i to N do for j in m1 do for k in m1 do if [j, k] in m1t2 then Cc2 :=
  {op(Cc2), e[i, j, k]} :fi:od:od:od: Cc2 := [op(Cc2)] :
Cc3 := { } :for i to N do for j in m1 do for k in m1 do for l in m1 do if [j, k, l] in m1t3
  then Cc3 := {op(Cc3), e[i, j, k, l]} :fi:od:od:od:od: Cc3 := [op(Cc3)] :

```

$$\emptyset, 88, 88 \quad (1.3.12)$$

```

> tmp := eliminate( { coeffs( expand( subs( sl2, cC2 ) - dC1 ), Cc2 ) }, { seq( cc[ op( C1[ i ][ 2 .. 3 ] ) ], i
    = 1 .. nops( C1 ) ) } ) :
tmss := solve( tmp[ 2 ] ) : ltm := [ ] : for i to nops( tmss ) do if lhs( tmss[ i ] )  $\neq$  rhs( tmss[ i ] )

```

```

then  $ltm := [op(ltm), lhs(tmss[i])] : \mathbf{fi} : \mathbf{od} : ltm : Coh2 := \{seq(diff(cC2, ltm[i]), i = 1$ 
 $\dots nops(ltm))\};$ 
 $deg2 := [ ] : \mathbf{for} i \mathbf{to} nops(Coh2) \mathbf{do} \mathbf{for} j \mathbf{to} nops(Cc2) \mathbf{do} \mathbf{if} diff(Cc2[j], Coh2[i]) \neq 0$ 
 $\mathbf{then} deg2 := [op(deg2), d[C2[j][2]] - d[C2[j][3]] - d[C2[j][4]]] : \mathbf{fi} : \mathbf{od} : \mathbf{od} : deg2;$ 
 $b2 := d1 - z1 : z2 := nops(Cf2) : d2 := nops(C2) : dim(B2) = b2, dim(Z2) = z2, dim(H2)$ 
 $= z2 - b2$ 
 $Coh2 := \{e_{8,4,10}, e_{8,4,14}, e_{8,12,12}, e_{8,12,16}, e_{8,16,16}\}$ 
 $[3, 3, 2, 2, 2]$ 
 $dim(B2) = 83, dim(Z2) = 88, dim(H2) = 5$ 

```

(1.3.13)

```

>  $Par2([e_{8,4,10}, e_{8,4,14}]), Par2([e_{8,12,12}, e_{8,12,16}, e_{8,16,16}])$ 
 $[0, 2], [3, 0]$ 

```

(1.3.14)

H2 is supported in homogeneity 2 (dim=0|2) and 3 (dim=3|0)

## Complex $C^*(m, g)$ for $m=m_4=g[-]$ corresponding to p[23] of DD-I

```

>  $m1 := \{1, 4, 7, 10, 12, 14\} : m10 := \{1, 4, 7\} : m11 := \{10, 12, 14\} :$ 
 $d[1] := -2 : d[2] := 0 : d[3] := 2 : d[4] := -1 : d[5] := 0 : d[6] := 1 : d[7] := -1 :$ 
 $d[8] := 0 : d[9] := 1 : d[10] := -2 : d[11] := 0 : d[12] := -1 : d[13] := 1 : d[14] :=$ 
 $-1 : d[15] := 1 : d[16] := 0 : d[17] := 2 :$ 
>  $Cc0 := [seq(e[i], i = 1..N)] : Cc1 := [seq(seq(e[i,j], j \mathbf{in} m1), i = 1..N)] : Cc2 :=$ 
 $[op(\{seq(seq(seq(e[i,j,k], k \mathbf{in} m1), j \mathbf{in} m1), i = 1..N)\} \setminus \{seq(seq(e[i,j,j], j = 1..n0), i$ 
 $= 1..N), seq(seq(seq(e[i,j,k], k = 1..j-1), j = 1..N), i = 1..N)\})] :$ 
>  $C0 := [seq([e[i], i], i = 1..N)] : C1 := [seq(seq([e[i,j], i,j], j \mathbf{in} m1), i = 1..N)] : C2 :=$ 
 $[op(\{seq(seq(seq([e[i,j,k], i,j,k], k \mathbf{in} m1), j \mathbf{in} m1), i = 1..N)\} \setminus \{seq(seq([e[i,j,j], i,j,$ 
 $j], j = 1..n0), i = 1..N), seq(seq(seq([e[i,j,k], i,j,k], k = 1..j-1), j = 1..N), i = 1..N)\})$ 
 $] :$ 
> for  $i \mathbf{to} N \mathbf{do} de[i] := add(add(c[i,j,k] e[k,j], j \mathbf{in} m1), k = 1..N) : \mathbf{od} :$ 
for  $k \mathbf{in} m1 \mathbf{do} d\theta[k] := eval\left(add\left(add\left(-\frac{1}{2} c[i,j,k] \theta[i,j], j \mathbf{in} m1\right), i \mathbf{in} m1\right),\right.$ 
 $\left.\{seq(seq(\theta[j,i] = -\theta[i,j], j = i+1..N), i = 1..n0), seq(\theta[j,j] = 0, j = 1..n0),\right.$ 
 $\left.seq(seq(\theta[j,i] = \theta[i,j], j = i+1..N), i = n0+1..N)\}\right) : \mathbf{od} :$ 
>  $cC0 := add(c[i] e[i], i = 1..N) : dC0 := collect(expand(add(c[i] de[i], i = 1..N)), Cc1) :$ 
>  $sl0 := solve(\{coeffs(dC0, Cc1)\}, \{seq(c[i], i = 1..N)\}) : eval(cC0, sl0)$ 
 $c_1 e_1 + c_{10} e_{10}$ 

```

(1.4.1)

```

>  $Par0([e_1, e_{10}], [d[1], d[10]])$ 
 $[1, 1], [-2, -2]$ 

```

(1.4.2)

```

>  $bl0 := factor(Basis([coeffs(dC0, Cc1)], plex(\alpha, seq(c[i], i = 1..N)))) : slb0 :=$ 
 $solve(\{op(bl0), \alpha \neq -1\})$ 
 $bl0 := [c_{17}, c_{16}, c_{15}, c_{14}, c_{13}, c_{12}, c_{11}, c_9, c_8, c_7, c_6, c_5, c_4, c_3, c_2]$ 
 $slb0 := \{\alpha = \alpha, c_2 = 0, c_3 = 0, c_4 = 0, c_5 = 0, c_6 = 0, c_7 = 0, c_8 = 0, c_9 = 0, c_{11} = 0, c_{12} = 0, c_{13}$ 
 $= 0, c_{14} = 0, c_{15} = 0, c_{16} = 0, c_{17} = 0\}$ 

```

(1.4.3)

$$\begin{aligned} &> \text{eval}(cC0, slb0) \\ &\qquad\qquad\qquad c_1 e_1 + c_{10} e_{10} \end{aligned} \tag{1.4.4}$$

$$\begin{aligned} &> Cf0 := \{ \} : \text{for } i \text{ to } nops(sl0) \text{ do if } lhs(sl0[i]) = rhs(sl0[i]) \text{ then } Cf0 := \{ op(Cf0), \\ &\quad lhs(sl0[i]) \} : \text{fi:od:} \\ &\quad b0 := 0 : z0 := nops(Cf0) : d0 := nops(C0) : \\ &\quad dim(B0) = b0, dim(Z0) = z0, dim(H0) = z0 - b0 \\ &\qquad\qquad\qquad dim(B0) = 0, dim(Z0) = 2, dim(H0) = 2 \end{aligned} \tag{1.4.5}$$

$$\begin{aligned} &> \text{for } i \text{ to } N \text{ do for } j \text{ in } m1 \text{ do } de[i, j] := \text{eval} \left( \text{add}(\text{add}(c[i, l, k] e[k, l, j], l \text{ in } m1), k = 1 .. N) \right. \\ &\quad \left. + \frac{1}{2} \text{add}(\text{add}(c[k, l, j] e[i, k, l], l \text{ in } m1), k \text{ in } m10) + \frac{1}{2} \text{add}(\text{add}(c[k, l, j] e[i, k, l], l \right. \\ &\quad \left. \text{in } m10), k \text{ in } m11) - \frac{1}{2} \text{add}(\text{add}(c[k, l, j] e[i, k, l], l \text{ in } m11), k \text{ in } m11), sbs1) \right) : \text{od:od:} \\ &> seq(\text{simplify}(\text{add}(\text{diff}(de[j], Cc1[i]) \cdot d \parallel (Cc1[i]), i = 1 .. nops(Cc1))), j = 1 .. nops(Cc0)) \\ &\qquad\qquad\qquad 0, 0, 0, 0, 0, 0, 0, 0, 0, 0, 0, 0, 0, 0, 0, 0, 0 \end{aligned} \tag{1.4.6}$$

$$\begin{aligned} &> cC1 := \text{add}(cc[op(C1[i][2..3])] C1[i, 1], i = 1 .. nops(C1)) : dC1 := \text{expand}(\text{add} \\ &\quad (cc[op(C1[i][2..3])] \cdot d \parallel (C1[i, 1]), i = 1 .. nops(C1))) : \\ &\quad bl1 := \text{Basis}([coeffs(dC1, Cc2)], \text{plex}(\alpha, seq(cc[op(C1[i][2..3])], i = 1 .. nops(C1)))) : \\ &\quad sll1 := \text{solve}(\{op(bl1), \alpha \neq 0, \alpha \neq -1\}) : \\ &\quad sll := \text{solve}(\{op(bl1), \alpha \neq 0, \alpha \neq -1\}, \{\alpha, seq(cc[op(C1[i][2..3])], i = 1 .. nops(C1))\} \\ &\quad \}) : nops(\{sll1\}), nops(\{sll\}); \\ &\quad Cfl := \{ \} : \text{for } i \text{ to } nops(sll) \text{ do if } lhs(sll[i]) = rhs(sll[i]) \text{ then } Cfl := \{ op(Cfl), \\ &\quad lhs(sll[i]) \} : \text{fi:od: } Cfl \\ &\qquad\qquad\qquad 1, 1 \end{aligned} \tag{1.4.7}$$

$$\begin{aligned} &\{ \alpha, cc_{1,4}, cc_{1,7}, cc_{1,12}, cc_{1,14}, cc_{5,10}, cc_{5,12}, cc_{5,14}, cc_{7,12}, cc_{10,1}, cc_{10,4}, cc_{10,7}, cc_{10,10}, cc_{10,12}, \\ &\quad cc_{10,14}, cc_{12,12}, cc_{14,4}, cc_{14,14}, cc_{15,14}, cc_{16,12}, cc_{16,14} \} \end{aligned} \tag{1.4.7}$$

$$\begin{aligned} &> Cfl := Cfl \setminus \{ \alpha \} : \\ &> \text{Basis}([coeffs(\text{expand}(\text{subs}(sll1, cC1) - dC0), Cc1)], \text{plex}(\alpha, seq(cc[op(C1[i][2..3])], i = 1 \\ &\quad .. nops(C1)), seq(c[i], i = 1 .. N))) : solve(%, \{seq(c[i], i = 1 .. N)\}) \\ &\quad [cc_{16,14} - c_6, cc_{16,12} - c_9, cc_{15,14} - c_3, cc_{14,14} + c_2 + c_5 - c_8, c_{16} + cc_{14,4}, cc_{12,12} + c_2 - c_5 \\ &\quad + c_8, cc_{10,14} - c_7, -c_4 + cc_{10,12}, c_2 + c_5 + c_8 + cc_{10,10}, c_{14} + cc_{10,7}, c_{12} + cc_{10,4}, cc_{10,1} \\ &\quad + c_{11}, 2 cc_{5,14} + c_{13}, -c_{15} + 2 cc_{5,12}, 2 cc_{5,10} - c_{17}, -c_{11} c_{12} + cc_{1,14} c_{11} + cc_{7,12} c_{12}, \\ &\quad cc_{1,12} c_{12} - c_{14} cc_{1,14}, -c_{11} c_{14} + cc_{1,12} c_{11} + cc_{7,12} c_{14}, cc_{1,7}, cc_{1,4}, c_{14} \alpha + c_{14} - cc_{1,12}, \\ &\quad c_{12} \alpha + c_{12} - cc_{1,14}, c_{11} \alpha + cc_{7,12}] \end{aligned} \tag{1.4.8}$$

$$\begin{aligned} &> tmp := \text{eliminate}(\{coeffs(\text{expand}(\text{subs}(sll, cC1) - dC0), Cc1)\}, \{seq(c[i], i = 1 .. N)\}) : \\ &\quad tmss := \text{solve}(tmp[2]) : ltm := [ ] : \text{for } i \text{ to } nops(tmss) \text{ do if } lhs(tmss[i]) \neq rhs(tmss[i]) \\ &\quad \text{then } ltm := [op(ltm), lhs(tmss[i])] : \text{fi:od: } ltm : Coh1 := \{seq(\text{diff}(cC1, ltm[i]), i = 1 \\ &\quad .. nops(ltm))\}; \\ &\quad deg1 := [ ] : \text{for } i \text{ to } nops(Coh1) \text{ do for } j \text{ to } nops(Cc1) \text{ do if } \text{diff}(Cc1[j], Coh1[i]) \neq 0 \\ &\quad \text{then } deg1 := [op(deg1), d[CI[j][2]] - d[CI[j][3]]] : \text{fi:od:od: } deg1; \end{aligned}$$



$$\text{eliminate}(\{\text{coeffs}(\text{expand}(\text{subs}(sl2, cC2) - dC1), Cc2)\}, Cf2) : \%[2], \text{nops}(\%[1]),$$

$$\text{nops}(Cf2)$$

$$\emptyset, 88, 88 \quad (1.4.12)$$

$$\begin{aligned} &> \text{tmp} := \text{eliminate}(\{\text{coeffs}(\text{expand}(\text{subs}(sl2, cC2) - dC1), Cc2)\}, \{\text{seq}(cc[\text{op}(CI[i][2..3])], i \\ &= 1 \dots \text{nops}(CI))\}) : \\ &\text{tmss} := \text{solve}(\text{tmp}[2]) : \text{ltm} := [] : \text{for } i \text{ to } \text{nops}(\text{tmss}) \text{ do if } \text{lhs}(\text{tmss}[i]) \neq \text{rhs}(\text{tmss}[i]) \\ &\text{ then } \text{ltm} := [\text{op}(\text{ltm}), \text{lhs}(\text{tmss}[i])] : \text{fi} : \text{od} : \text{ltm} : \text{Coh2} := \{\text{seq}(\text{diff}(cC2, \text{ltm}[i]), i = 1 \\ &\dots \text{nops}(\text{ltm}))\}; \\ &\text{deg2} := [] : \text{for } i \text{ to } \text{nops}(\text{Coh2}) \text{ do for } j \text{ to } \text{nops}(Cc2) \text{ do if } \text{diff}(Cc2[j], \text{Coh2}[i]) \neq 0 \\ &\text{ then } \text{deg2} := [\text{op}(\text{deg2}), d[C2[j][2]] - d[C2[j][3]] - d[C2[j][4]]] : \text{fi} : \text{od} : \text{od} : \text{deg2}; \\ &b2 := d1 - z1 : z2 := \text{nops}(Cf2) : d2 := \text{nops}(C2) : \text{dim}(B2) = b2, \text{dim}(Z2) = z2, \text{dim}(H2) \\ &= z2 - b2 \\ &\text{Coh2} := \{e_{1,4,7}, e_{1,4,12}, e_{8,4,14}, e_{8,7,12}, e_{8,14,14}, e_{11,7,12}\} \\ &[0, 0, 2, 2, 2, 2] \\ &\text{dim}(B2) = 82, \text{dim}(Z2) = 88, \text{dim}(H2) = 6 \end{aligned} \quad (1.4.13)$$

$$\begin{aligned} &> \text{Par2}([e_{1,4,7}, e_{1,4,12}]), \text{Par2}([e_{8,4,14}, e_{8,7,12}, e_{8,14,14}, e_{11,7,12}]) \\ &[1, 1], [2, 2] \end{aligned} \quad (1.4.14)$$

H2 is supported in homogeneity 0 (dim=1|1) and 2 (dim=2|2)

## Complex $C^*(m, g)$ for $m=m5=g[-]$ corresponding to p[123] of DD-I

$$\begin{aligned} &> m1 := \{1, 4, 7, 10, 12, 14, 16\} : m10 := \{1, 4, 7\} : m11 := \{10, 12, 14, 16\} : \\ &d[1] := -4 : d[2] := 0 : d[3] := 4 : d[4] := -1 : d[5] := 0 : d[6] := 1 : d[7] := -1 : \\ &d[8] := 0 : d[9] := 1 : d[10] := -3 : d[11] := 1 : d[12] := -2 : d[13] := 2 : d[14] := \\ &-2 : d[15] := 2 : d[16] := -1 : d[17] := 3 : \\ &> Cc0 := [\text{seq}(e[i], i = 1 \dots N)] : Cc1 := [\text{seq}(\text{seq}(e[i, j], j \text{ in } m1), i = 1 \dots N)] : Cc2 := \\ &[\text{op}(\{\text{seq}(\text{seq}(\text{seq}(e[i, j, k], k \text{ in } m1), j \text{ in } m1), i = 1 \dots N)\} \setminus \{\text{seq}(\text{seq}(e[i, j, j], j = 1 \dots n0), i \\ &= 1 \dots N), \text{seq}(\text{seq}(\text{seq}(e[i, j, k], k = 1 \dots j - 1), j = 1 \dots N), i = 1 \dots N)\})] : \\ &> C0 := [\text{seq}([e[i], i], i = 1 \dots N)] : C1 := [\text{seq}(\text{seq}([e[i, j], i, j], j \text{ in } m1), i = 1 \dots N)] : C2 := \\ &[\text{op}(\{\text{seq}(\text{seq}(\text{seq}([e[i, j, k], i, j, k], k \text{ in } m1), j \text{ in } m1), i = 1 \dots N)\} \setminus \{\text{seq}(\text{seq}([e[i, j, j], i, j, j], j = 1 \dots n0), i = 1 \dots N), \\ &\text{seq}(\text{seq}(\text{seq}([e[i, j, k], i, j, k], k = 1 \dots j - 1), j = 1 \dots N), i = 1 \dots N)\})] : \\ &> \text{for } i \text{ to } N \text{ do } de[i] := \text{add}(\text{add}(c[i, j, k] e[k, j], j \text{ in } m1), k = 1 \dots N) : \text{od} : \\ &\text{for } k \text{ in } m1 \text{ do } d\theta[k] := \text{eval}\left(\text{add}\left(\text{add}\left(-\frac{1}{2} c[i, j, k] \theta[i, j], j \text{ in } m1\right), i \text{ in } m1\right), \right. \\ &\quad \left. \{\text{seq}(\text{seq}(\theta[j, i] = -\theta[i, j], j = i + 1 \dots N), i = 1 \dots n0), \text{seq}(\theta[j, j] = 0, j = 1 \dots n0), \right. \\ &\quad \left. \text{seq}(\text{seq}(\theta[j, i] = \theta[i, j], j = i + 1 \dots N), i = n0 + 1 \dots N)\} \right) : \text{od} : \\ &> cC0 := \text{add}(c[i] e[i], i = 1 \dots N) : dC0 := \text{collect}(\text{expand}(\text{add}(c[i] de[i], i = 1 \dots N)), Cc1) : \\ &> sl0 := \text{solve}(\{\text{coeffs}(dC0, Cc1)\}, \{\text{seq}(c[i], i = 1 \dots N)\}) : \text{eval}(cC0, sl0) \\ &c_1 e_1 \end{aligned} \quad (1.5.1)$$

$$\begin{aligned} &> \text{Par0}([e_1]), [d[1]] \\ &[1, 0], [-4] \end{aligned} \quad (1.5.2)$$



$$\begin{aligned}
& \triangleright \text{bl0} := \text{factor}(\text{Basis}([\text{coeffs}(\text{dC0}, \text{Cc1})], \text{plex}(\alpha, \text{seq}(c[i], i = 1 \dots N)))); \text{slb0} := \\
& \quad \text{solve}(\{\text{op}(\text{bl0}), \alpha \neq -1\}) \\
& \quad \text{bl0} := [c_{17}, c_{16}, c_{15}, c_{14}, c_{13}, c_{12}, c_{11}, c_9, c_8, c_7, c_6, c_5, c_4, c_3, c_2, c_{10} (1 + \alpha)] \\
& \text{slb0} := \{\alpha = \alpha, c_2 = 0, c_3 = 0, c_4 = 0, c_5 = 0, c_6 = 0, c_7 = 0, c_8 = 0, c_9 = 0, c_{10} = 0, c_{11} = 0, c_{12} \\
& \quad = 0, c_{13} = 0, c_{14} = 0, c_{15} = 0, c_{16} = 0, c_{17} = 0\} \quad (1.5.3)
\end{aligned}$$

$$\begin{aligned}
& \triangleright \text{eval}(\text{cC0}, \text{slb0}) \\
& \quad c_1 e_1 \quad (1.5.4)
\end{aligned}$$

$$\begin{aligned}
& \triangleright \text{Cf0} := \{\} : \text{for } i \text{ to } \text{nops}(\text{sl0}) \text{ do if } \text{lhs}(\text{sl0}[i]) = \text{rhs}(\text{sl0}[i]) \text{ then } \text{Cf0} := \{\text{op}(\text{Cf0}), \\
& \quad \text{lhs}(\text{sl0}[i])\} : \text{fi:od:} \\
& \text{b0} := 0 : \text{z0} := \text{nops}(\text{Cf0}) : \text{d0} := \text{nops}(\text{C0}) : \\
& \text{dim}(\text{B0}) = \text{b0}, \text{dim}(\text{Z0}) = \text{z0}, \text{dim}(\text{H0}) = \text{z0} - \text{b0} \\
& \quad \text{dim}(\text{B0}) = 0, \text{dim}(\text{Z0}) = 1, \text{dim}(\text{H0}) = 1 \quad (1.5.5)
\end{aligned}$$

$$\begin{aligned}
& \triangleright \text{for } i \text{ to } N \text{ do for } j \text{ in } m1 \text{ do } \text{de}[i, j] := \text{eval}\left(\text{add}(\text{add}(c[i, l, k] e[k, l, j], l \text{ in } m1), k = 1 \dots N) \right. \\
& \quad \left. + \frac{1}{2} \text{add}(\text{add}(c[k, l, j] e[i, k, l], l \text{ in } m1), k \text{ in } m10) + \frac{1}{2} \text{add}(\text{add}(c[k, l, j] e[i, k, l], l \right. \\
& \quad \left. \text{in } m10), k \text{ in } m11) - \frac{1}{2} \text{add}(\text{add}(c[k, l, j] e[i, k, l], l \text{ in } m11), k \text{ in } m11), \text{sbs1}\right) : \text{od:od:} \\
& \triangleright \text{seq}(\text{simplify}(\text{add}(\text{diff}(\text{de}[j], \text{Cc1}[i]) \cdot d \parallel (\text{Cc1}[i]), i = 1 \dots \text{nops}(\text{Cc1})), j = 1 \dots \text{nops}(\text{Cc0})) \\
& \quad 0, 0, 0, 0, 0, 0, 0, 0, 0, 0, 0, 0, 0, 0, 0, 0, 0 \quad (1.5.6)
\end{aligned}$$

$$\begin{aligned}
& \triangleright \text{cC1} := \text{add}(\text{cc}[\text{op}(\text{C1}[i][2 \dots 3])] \text{C1}[i, 1], i = 1 \dots \text{nops}(\text{C1})) : \text{dC1} := \text{expand}(\text{add} \\
& \quad (\text{cc}[\text{op}(\text{C1}[i][2 \dots 3])] \cdot d \parallel (\text{C1}[i, 1]), i = 1 \dots \text{nops}(\text{C1}))) : \\
& \text{b11} := \text{Basis}([\text{coeffs}(\text{dC1}, \text{Cc2})], \text{plex}(\alpha, \text{seq}(\text{cc}[\text{op}(\text{C1}[i][2 \dots 3])], i = 1 \dots \text{nops}(\text{C1})))) : \\
& \text{s11a} := \text{solve}(\{\text{op}(\text{b11}), \alpha \neq 0, \alpha \neq -1\}) : \\
& \text{s11} := \text{solve}(\{\text{op}(\text{b11}), \alpha \neq 0, \alpha \neq -1\}, \{\alpha, \text{seq}(\text{cc}[\text{op}(\text{C1}[i][2 \dots 3])], i = 1 \dots \text{nops}(\text{C1}))\} \\
& \quad \}) : \text{nops}(\{\text{s11a}\}), \text{nops}(\{\text{s11}\}); \\
& \text{Cf1} := \{\} : \text{for } i \text{ to } \text{nops}(\text{s11}) \text{ do if } \text{lhs}(\text{s11}[i]) = \text{rhs}(\text{s11}[i]) \text{ then } \text{Cf1} := \{\text{op}(\text{Cf1}), \\
& \quad \text{lhs}(\text{s11}[i])\} : \text{fi:od: Cf1} \\
& \quad 1, 1 \\
& \{\alpha, \text{cc}_{1,4}, \text{cc}_{1,7}, \text{cc}_{1,16}, \text{cc}_{5,10}, \text{cc}_{5,12}, \text{cc}_{5,14}, \text{cc}_{8,16}, \text{cc}_{10,1}, \text{cc}_{10,4}, \text{cc}_{10,7}, \text{cc}_{10,12}, \text{cc}_{12,12}, \text{cc}_{12,16}, \\
& \quad \text{cc}_{14,4}, \text{cc}_{14,14}, \text{cc}_{16,12}, \text{cc}_{16,14}, \text{cc}_{16,16}, \text{cc}_{17,16}\} \quad (1.5.7)
\end{aligned}$$

$$\begin{aligned}
& \triangleright \text{Cf1} := \text{Cf1} \setminus \{\alpha\} : \\
& \triangleright \text{Basis}([\text{coeffs}(\text{expand}(\text{subs}(\text{s11a}, \text{cC1}) - \text{dC0}), \text{Cc1})], \text{plex}(\alpha, \text{seq}(\text{cc}[\text{op}(\text{C1}[i][2 \dots 3])], i = 1 \\
& \quad \dots \text{nops}(\text{C1})), \text{seq}(c[i], i = 1 \dots N))]; \text{solve}(\%, \{\text{seq}(c[i], i = 1 \dots N)\}) \\
& [-c_3 + \text{cc}_{17,16}, \text{cc}_{16,16} + c_2 - c_5 - c_8, \text{cc}_{16,14} - c_6, \text{cc}_{16,12} - c_9, \text{cc}_{14,14} + c_2 + c_5 - c_8, c_{16} \\
& \quad + \text{cc}_{14,4}, \text{cc}_{12,12} + c_2 - c_5 + c_8, \text{cc}_{10,14} - c_7, -c_4 + \text{cc}_{10,12}, c_{14} + \text{cc}_{10,7}, c_{12} + \text{cc}_{10,4}, \text{cc}_{10,1} \\
& \quad + c_{11}, 2 \text{cc}_{5,14} + c_{13}, -c_{15} + 2 \text{cc}_{5,12}, 2 \text{cc}_{5,10} - c_{17}, c_{10} c_{11} - 2 \text{cc}_{8,16} c_{10} + \text{cc}_{1,16} c_{11}, \\
& \quad \text{cc}_{1,7}, \text{cc}_{1,4}, c_{11} \alpha + 2 \text{cc}_{8,16} c_{10} \alpha + c_{10} + \text{cc}_{1,16}] \quad (1.5.8)
\end{aligned}$$



```

then Cc3 := {op(Cc3), e[i, j, k, l]} : fi : od : od : od : Cc3 := [op(Cc3)] :
> cC2 := add(cc[op(C2[i][2..4])] C2[i, 1], i = 1..nops(C2)) : dC2 := expand(add
(cc[op(C2[i][2..4])]·d[(C2[i, 1]), i = 1..nops(C2))]) :
sl2 := solve({coeffs(dC2, Cc3)}, {seq(cc[op(C2[i][2..4])], i = 1..nops(C2))}) : Cf2 := {} :
for i to nops(sl2) do if lhs(sl2[i]) = rhs(sl2[i]) then Cf2 := {op(Cf2), lhs(sl2[i])} : fi :
od :
eliminate({coeffs(expand(subs(sl2, cC2) - dC1), Cc2)}, Cf2) : %[2], nops(%[1]),
nops(Cf2)

```

(1.5.12)

```

> tmp := eliminate({coeffs(expand(subs(sl2, cC2) - dC1), Cc2)}, {seq(cc[op(C1[i][2..3])], i
= 1..nops(C1))}) :
tmss := solve(tmp[2]) : ltm := [] : for i to nops(tmss) do if lhs(tmss[i]) ≠ rhs(tmss[i])
then ltm := [op(ltm), lhs(tmss[i])] : fi : od : ltm : Coh2 := {seq(diff(cC2, ltm[i]), i = 1
..nops(ltm))} :
deg2 := [] : for i to nops(Coh2) do for j to nops(Cc2) do if diff(Cc2[j], Coh2[i]) ≠ 0
then deg2 := [op(deg2), d[C2[j][2]] - d[C2[j][3]] - d[C2[j][4]]] : fi : od : od : deg2 :
b2 := d1 - z1 : z2 := nops(Cf2) : d2 := nops(C2) : dim(B2) = b2, dim(Z2) = z2, dim(H2)
= z2 - b2

```

Coh2 := {e<sub>1,4,7</sub>, e<sub>8,4,14</sub>, e<sub>8,7,12</sub>, e<sub>8,16,16</sub>}

[-2, 3, 3, 2]

dim(B2) = 100, dim(Z2) = 104, dim(H2) = 4 (1.5.13)

```

> Par2([e1,4,7]), Par2([e8,16,16]), Par2([e8,4,14, e8,7,12])
[1, 0], [1, 0], [0, 2] (1.5.14)

```

H2 is supported in homogeneity -2 (dim=1|0) and 2 (dim=1|0) and 3 (dim=0|2)

## Complex C\*(m,g) for m=m6=g[-] corresponding to p[123] of DD-II

```

> m1 := {1, 4, 7, 10, 11, 12, 14} : m10 := {1, 4, 7} : m11 := {10, 11, 12, 14} :
d[1] := -2 : d[2] := 0 : d[3] := 2 : d[4] := -2 : d[5] := 0 : d[6] := 2 : d[7] := -2 :
d[8] := 0 : d[9] := 2 : d[10] := -3 : d[11] := -1 : d[12] := -1 : d[13] := 1 :
d[14] := -1 : d[15] := 1 : d[16] := 1 : d[17] := 3 :
> Cc0 := [seq(e[i], i = 1..N)] : Cc1 := [seq(seq(e[i, j], j in m1), i = 1..N)] : Cc2 :=
[op({seq(seq(seq(e[i, j, k], k in m1), j in m1), i = 1..N)}\{seq(seq(e[i, j, j], j = 1..n0), i
= 1..N), seq(seq(seq(e[i, j, k], k = 1..j-1), j = 1..N), i = 1..N)})] :
> C0 := [seq([e[i], i], i = 1..N)] : C1 := [seq(seq([e[i, j], i, j], j in m1), i = 1..N)] : C2 :=
[op({seq(seq(seq([e[i, j, k], i, j, k], k in m1), j in m1), i = 1..N)}\{seq(seq([e[i, j, j], i, j,
j], j = 1..n0), i = 1..N), seq(seq(seq([e[i, j, k], i, j, k], k = 1..j-1), j = 1..N), i = 1..N)})] :
> for i to N do de[i] := add(add(c[i, j, k] e[k, j], j in m1), k = 1..N) : od :
for k in m1 do dθ[k] := eval( add( add( - 1/2 c[i, j, k] θ[i, j], j in m1 ), i in m1 ),
{seq(seq(θ[j, i] = -θ[i, j], j = i + 1..N), i = 1..n0), seq(θ[j, j] = 0, j = 1..n0),
seq(seq(θ[j, i] = θ[i, j], j = i + 1..N), i = n0 + 1..N)}) : od :

```

$$\begin{aligned}
&> cC0 := add(c[i] e[i], i = 1 .. N) : dC0 := collect(expand(add(c[i] de[i], i = 1 .. N)), Cc1) : \\
&> sl0 := solve(\{coeffs(dC0, Cc1)\}, \{seq(c[i], i = 1 .. N)\}) : eval(cC0, sl0) \\
&\qquad\qquad\qquad c_{10} e_{10} \qquad\qquad\qquad (1.6.1)
\end{aligned}$$

$$\begin{aligned}
&> Par0([e_{10}], [d[10]]) \\
&\qquad\qquad\qquad [0, 1], [-3] \qquad\qquad\qquad (1.6.2)
\end{aligned}$$

$$\begin{aligned}
&> bl0 := factor(Basis([coeffs(dC0, Cc1)], plex(\alpha, seq(c[i], i = 1 .. N)))) : slb0 := \\
&\quad solve(\{op(bl0), \alpha \neq -1\}) \\
&\quad\quad bl0 := [c_{17}, c_{16}, c_{15}, c_{14}, c_{13}, c_{12}, c_{11}, c_9, c_8, c_7, c_6, c_5, c_4, c_3, c_2, c_1] \\
slb0 := \{\alpha = \alpha, c_1 = 0, c_2 = 0, c_3 = 0, c_4 = 0, c_5 = 0, c_6 = 0, c_7 = 0, c_8 = 0, c_9 = 0, c_{11} = 0, c_{12} \\
= 0, c_{13} = 0, c_{14} = 0, c_{15} = 0, c_{16} = 0, c_{17} = 0\} \qquad\qquad\qquad (1.6.3)
\end{aligned}$$

$$\begin{aligned}
&> eval(cC0, slb0) \\
&\qquad\qquad\qquad c_{10} e_{10} \qquad\qquad\qquad (1.6.4)
\end{aligned}$$

$$\begin{aligned}
&> Cf0 := \{\} : \text{for } i \text{ to } nops(sl0) \text{ do if } lhs(sl0[i]) = rhs(sl0[i]) \text{ then } Cf0 := \{op(Cf0), \\
&\quad lhs(sl0[i])\} : \text{fi:od:} \\
b0 := 0 : z0 := nops(Cf0) : d0 := nops(C0) : \\
dim(B0) = b0, dim(Z0) = z0, dim(H0) = z0 - b0 \\
\qquad\qquad\qquad dim(B0) = 0, dim(Z0) = 1, dim(H0) = 1 \qquad\qquad\qquad (1.6.5)
\end{aligned}$$

$$\begin{aligned}
&> \text{for } i \text{ to } N \text{ do for } j \text{ in } m1 \text{ do } de[i, j] := eval\left( add(add(c[i, l, k] e[k, l, j], l \text{ in } m1), k = 1 .. N) \right. \\
&\quad \left. + \frac{1}{2} add(add(c[k, l, j] e[i, k, l], l \text{ in } m1), k \text{ in } m10) + \frac{1}{2} add(add(c[k, l, j] e[i, k, l], l \right. \\
&\quad \left. \text{in } m10), k \text{ in } m11) - \frac{1}{2} add(add(c[k, l, j] e[i, k, l], l \text{ in } m11), k \text{ in } m11), sbs1 \right) : \text{od:od:} \\
&> seq(simplify(add(diff(de[j], Cc1[i]) \cdot d || (Cc1[i]), i = 1 .. nops(Cc1))), j = 1 .. nops(Cc0)) \\
&\qquad\qquad\qquad 0, 0, 0, 0, 0, 0, 0, 0, 0, 0, 0, 0, 0, 0, 0, 0, 0 \qquad\qquad\qquad (1.6.6)
\end{aligned}$$

$$\begin{aligned}
&> cC1 := add(cc[op(CI[i][2..3])] CI[i, 1], i = 1 .. nops(CI)) : dC1 := expand(add \\
&\quad (cc[op(CI[i][2..3])] \cdot d || (CI[i, 1]), i = 1 .. nops(CI))) : \\
b11 := Basis([coeffs(dC1, Cc2)], plex(\alpha, seq(cc[op(CI[i][2..3])], i = 1 .. nops(CI)))) : \\
s11a := solve(\{op(b11), \alpha \neq 0, \alpha \neq -1\}) : \\
s11 := solve(\{op(b11), \alpha \neq 0, \alpha \neq -1\}, \{\alpha, seq(cc[op(CI[i][2..3])], i = 1 .. nops(CI))\} \\
\quad \}) : nops(\{s11a\}), nops(\{s11\}); \\
Cf1 := \{\} : \text{for } i \text{ to } nops(s11) \text{ do if } lhs(s11[i]) = rhs(s11[i]) \text{ then } Cf1 := \{op(Cf1), \\
lhs(s11[i])\} : \text{fi:od: } Cf1 \\
\qquad\qquad\qquad 1, 1
\end{aligned}$$

$$\begin{aligned}
&\{\alpha, cc_{1, 14}, cc_{4, 11}, cc_{5, 10}, cc_{5, 11}, cc_{5, 12}, cc_{5, 14}, cc_{7, 12}, cc_{10, 1}, cc_{10, 4}, cc_{10, 7}, cc_{10, 11}, cc_{10, 12}, cc_{10, 14}, \\
&\quad cc_{11, 11}, cc_{12, 12}, cc_{14, 14}, cc_{15, 14}, cc_{16, 12}, cc_{16, 14}\} \qquad\qquad\qquad (1.6.7)
\end{aligned}$$

$$\begin{aligned}
&> Cf1 := Cf1 \setminus \{\alpha\} : \\
&> Basis([coeffs(expand(subs(s11a, cC1) - dC0), Cc1)], plex(\alpha, seq(cc[op(CI[i][2..3])], i = 1 \\
&\quad .. nops(CI)), seq(c[i], i = 1 .. N))) : solve(%, \{seq(c[i], i = 1 .. N)\}) \\
&\qquad\qquad\qquad (1.6.8)
\end{aligned}$$

$$\begin{aligned} & \left[ cc_{16,14} - c_6, cc_{16,12} - c_9, cc_{15,14} - c_3, cc_{14,14} + c_2 + c_5 - c_8, cc_{12,12} + c_2 - c_5 + c_8, -c_2 + c_5 \right. \\ & \quad + c_8 + cc_{11,11}, cc_{10,14} - c_7, -c_4 + cc_{10,12}, -c_1 + cc_{10,11}, c_{14} + cc_{10,7}, c_{12} + cc_{10,4}, cc_{10,1} \\ & \quad + c_{11}, 2cc_{5,14} + c_{13}, -c_{15} + 2cc_{5,12}, 2cc_{5,11} + c_{16}, 2cc_{5,10} - c_{17}, c_{14} + cc_{4,11}, -c_{11}c_{12} \\ & \quad \left. + cc_{1,14}c_{11} + cc_{7,12}c_{12}, c_{12}\alpha + c_{12} - cc_{1,14}, c_{11}\alpha + cc_{7,12} \right] \quad (1.6.8) \end{aligned}$$

$$Parl([e_{1,14}, e_{4,11}, e_{7,12}]) \quad [0, 3] \quad (1.6.10)$$

[illegible]

```

    {op(mlt2), [j, k]} :fi:od:od:
    mlt3 := { } :for j in m1 do for k in m1 do for l in m1 do if (k > j and l > k) or (k=j and j
    in m11 and l ≥ k) or (l=k and k in m11 and j < k) then mlt3 := {op(mlt3), [j, k, l]} :
    fi:od:od:od:

```

```

> Cc2 := { } :for i to N do for j in m1 do for k in m1 do if [j, k] in mlt2 then Cc2 :=
    {op(Cc2), e[i, j, k]} :fi:od:od:od: Cc2 := [op(Cc2)] :
    Cc3 := { } :for i to N do for j in m1 do for k in m1 do for l in m1 do if [j, k, l] in mlt3
    then Cc3 := {op(Cc3), e[i, j, k, l]} :fi:od:od:od:od: Cc3 := [op(Cc3)] :
> cC2 := add(cc[op(C2[i][2..4])] C2[i, 1], i = 1..nops(C2)) : dC2 := expand(add
    (cc[op(C2[i][2..4])]·d|| (C2[i, 1]), i = 1..nops(C2))) :
    sl2 := solve({coeffs(dC2, Cc3)}, {seq(cc[op(C2[i][2..4])], i = 1..nops(C2))}) : Cf2 := { } :
    for i to nops(sl2) do if lhs(sl2[i]) = rhs(sl2[i]) then Cf2 := {op(Cf2), lhs(sl2[i])} :fi:
    od:
    eliminate({coeffs(expand(subs(sl2, cC2) - dC1), Cc2)}, Cf2) : %[2], nops(%[1]),
    nops(Cf2)

```

∅, 104, 104

(1.6.12)

```

> tmp := eliminate({coeffs(expand(subs(sl2, cC2) - dC1), Cc2)}, {seq(cc[op(C1[i][2..3])], i
    = 1..nops(C1))}) :
    tmss := solve(tmp[2]) : ltm := [ ] : for i to nops(tmss) do if lhs(tmss[i]) ≠ rhs(tmss[i])
    then ltm := [op(ltm), lhs(tmss[i])] :fi:od: ltm : Coh2 := {seq(diff(cC2, ltm[i]), i = 1
    ..nops(ltm))} :
    deg2 := [ ] : for i to nops(Coh2) do for j to nops(Cc2) do if diff(Cc2[j], Coh2[i]) ≠ 0
    then deg2 := [op(deg2), d[C2[j][2]] - d[C2[j][3]] - d[C2[j][4]]] :fi:od:od: deg2:
    b2 := d1 - z1 : z2 := nops(Cf2) : d2 := nops(C2) : dim(B2) = b2, dim(Z2) = z2, dim(H2)
    = z2 - b2

```

$Coh2 := \{e_{7, 11, 12}, e_{8, 14, 14}, e_{11, 7, 12}, e_{12, 7, 11}\}$

[0, 2, 2, 2]

$dim(B2) = 100, dim(Z2) = 104, dim(H2) = 4$

(1.6.13)

```

> Par2([e7, 11, 12]), Par2([e8, 14, 14, e11, 7, 12, e12, 7, 11])
    [1, 0], [3, 0]

```

(1.6.14)

H2 is supported in homogeneity 0 (dim=1|0) and 2 (dim=3|0)

>

>
