# Supplementary material for: Geometric realizations of the Lie superalgebra D(2,1;a)
Source: arXiv:2507.03418 ancillary file (2025-07-04)
Supplement: Supplementary file 3 [file JB_for_p12i.pdf]

In this worksheet we work with G/P\_1^I realization of LSA D(2,1;a)

> *interface*(warnlevel = 0) : with(Physics) :

> Setup(anticommutativeprefix = {seq(y||i, i = 1..4)}, anticommutativecolor = maroon)  
[anticommutativecolor = maroon, anticommutativeprefix = {y1, y2, y3, y4}] (1)

> var := x, y1, y2, y3, y4 : GrassmannParity(y2 y3), GrassmannParity(y2 y3 y4)  
0, 1 (2)

> diff(y2 y3, y2), diff(y3 y2, y2)  
y3, -y3 (3)

The Jacobi-Lagrange bracket, version 1:  $\sigma = dx + y1 dy1 + y2 dy2 + y3 dy3 + y4 dy4$

> X := (f, g) → simplify  $\left( f \text{diff}(g, x) + \frac{(-1)^{\text{GrassmannParity}(f)}}{2} \text{add}((\text{diff}(f, y||i) + (y||i) \text{diff}(f, x)) \cdot (\text{diff}(g, y||i) + (y||i) \text{diff}(g, x)), i = 1..4) \right) :$

JB := (f, g) → simplify  $\left( f \text{diff}(g, x) - (-1)^{\text{GrassmannParity}(f) \cdot \text{GrassmannParity}(g)} g \text{diff}(f, x) + \frac{(-1)^{\text{GrassmannParity}(f)}}{2} \text{add}((\text{diff}(f, y||i) + (y||i) \text{diff}(f, x)) \cdot (\text{diff}(g, y||i) + (y||i) \text{diff}(g, x)), i = 1..4) \right) :$

XJB := (f, g, h) → simplify  $(X(f, X(g, h)) - (-1)^{\text{GrassmannParity}(f) \cdot \text{GrassmannParity}(g)} X(g, X(f, h)) - X(JB(f, g), h)) :$

> {seq(seq(seq(XJB(var[i], var[j], var[k])), k = 1..5), j = 1..5), i = 1..5)}  
{0} (4)

# x=x, y[i] = ξ[i]

> g :=  $\left[ 1, y1, y2, y3, y4, x, y1 y2, y1 y3, y1 y4, y2 y3, y2 y4, y3 y4, x y1 + a y2 y3 y4, x y2 - a y1 y3 y4, x y3 + a y1 y2 y4, x y4 - a y1 y2 y3, \frac{x^2}{2} - a y1 y2 y3 y4 \right] :$

#` [1], [y1, y2, y3, y4], [x, y1 y2, y1 y3, y1 y4, y2 y3, y2 y4, y3 y4], [x y1 + a y2 y3 y4, x y2 - a y1 y3 y4, x y3 + a y1 y2 y4, x y4 - a y1 y2 y3],  $\left[ \frac{x^2}{2} - a y1 y2 y3 y4 \right]$

> seq(JB(g[1], g[i]), i = 2..5), seq(JB(g[1], g[i]), i = 6..12), seq(seq(JB(g[i], g[j]), j = i + 2..5), i = 2..5)  
0, 0, 0, 0, 1, 0, 0, 0, 0, 0, 0, 0, 0, 0 (5)

> seq(seq(JB(g[i], g[j]), i = 2..5), j = 6..12)  
 $\frac{y1}{2}, \frac{y2}{2}, \frac{y3}{2}, \frac{y4}{2}, -\frac{y2}{2}, \frac{y1}{2}, 0, 0, -\frac{y3}{2}, 0, \frac{y1}{2}, 0, -\frac{y4}{2}, 0, 0, \frac{y1}{2}, 0, -\frac{y3}{2}, \frac{y2}{2}, 0, 0,$   
 $-\frac{y4}{2}, 0, \frac{y2}{2}, 0, 0, -\frac{y4}{2}, \frac{y3}{2}$  (6)

> seq(seq(JB(g[i], g[j]), j = i + 1..12), i = 7..12) (7)

$$\frac{y_2 y_3}{2}, \frac{y_2 y_4}{2}, -\frac{y_1 y_3}{2}, -\frac{y_1 y_4}{2}, 0, \frac{y_3 y_4}{2}, \frac{y_1 y_2}{2}, 0, -\frac{y_1 y_4}{2}, 0, \frac{y_1 y_2}{2}, \frac{y_1 y_3}{2}, \frac{y_3 y_4}{2},$$

$$-\frac{y_2 y_4}{2}, \frac{y_2 y_3}{2}$$

> seq(seq(JB(g[i], g[j]), i=j..16), j=13..16)

$$a y_1 y_2 y_3 y_4 - \frac{x^2}{2}, 0, 0, 0, a y_1 y_2 y_3 y_4 - \frac{x^2}{2}, 0, 0, a y_1 y_2 y_3 y_4 - \frac{x^2}{2}, 0, a y_1 y_2 y_3 y_4 - \frac{x^2}{2} \quad (8)$$

>

The Jacobi-Lagrange bracket, version 2:  $\sigma = dx + y_3 \cdot dy_1 + y_4 \cdot dy_2 = dx - dy_1 \cdot y_3 - dy_2 \cdot y_4$

> X := (f, g) → simplify(f diff(g, x) + (-1)<sup>GrassmannParity(f)</sup> add(diff(f, y|| (i+2)) · (diff(g, y|| i) + (y|| (i+2)) diff(g, x)), i=1..2) + (-1)<sup>GrassmannParity(f)</sup> add((diff(f, y|| i) + (y|| (i+2)) diff(f, x)) · diff(g, y|| (i+2)), i=1..2)):

JB := (f, g) → simplify(f diff(g, x) - (-1)<sup>GrassmannParity(f) · GrassmannParity(g)</sup> g diff(f, x) + (-1)<sup>GrassmannParity(f)</sup> add(diff(f, y|| (i+2)) · (diff(g, y|| i) + (y|| (i+2)) diff(g, x)), i=1..2) + (-1)<sup>GrassmannParity(f)</sup> add((diff(f, y|| i) + (y|| (i+2)) diff(f, x)) · diff(g, y|| (i+2)), i=1..2)):

XJB := (f, g, h) → simplify(X(f, X(g, h)) - (-1)<sup>GrassmannParity(f) · GrassmannParity(g)</sup> X(g, X(f, h)) - X(JB(f, g), h)):

> {seq(seq(seq(XJB(var[i], var[j], var[k])), k=1..5), j=1..5), i=1..5)}  
{0}

(9)

# y[1] = 0[1], y[2] = 0[2], y[3] = v[1], y[4] = v[2]

> g := [1, y1, y2, y3, y4, y1 y2, x, y1 y3, y1 y4, y2 y3, y2 y4, y3 y4, x y1 + a y1 y2 y4, x y2 - a y1 y2 y3, x y3 + (a+1) y2 y3 y4, x y4 - (a+1) y1 y3 y4, x<sup>2</sup> - (y1 y3 + y2 y4) x - (a+1) y1 y2 y3 y4]:

# [1, [y1, y2], [y3, y4, y1 y2], [x, y1 y3, y1 y4, y2 y3, y2 y4], [y3 y4, x y1 + a y1 y2 y4, x y2 - a y1 y2 y3], [x y3 + (a+1) y2 y3 y4, x y4 - (a+1) y1 y3 y4], [x<sup>2</sup> - (y1 y3 + y2 y4) x - (a+1) y1 y2 y3 y4]

> seq(JB(g[1], g[i]), i=2..6), seq(JB(g[1], g[i]), i=7..11)  
0, 0, 0, 0, 0, 1, 0, 0, 0, 0

(10)

> seq(seq(JB(g[i], g[j]), j=4..6), i=4..6), seq(seq(JB(g[i], g[j]), j=2..3), i=4..6)  
0, 0, -y2, 0, 0, y1, y2, -y1, 0, -1, 0, 0, -1, 0, 0

(11)

> seq(seq(JB(g[i], g[j]), i=7..11), j=7..11)

0, 0, 0, 0, 0, 0, 0, y1 y4, -y2 y3, 0, 0, -y1 y4, 0, -y2 y4 + y1 y3, y1 y4, 0, y2 y3, -y1 y3 + y2 y4, 0, -y2 y3, 0, 0, -y1 y4, y2 y3, 0

(12)

> seq(seq(JB(g[i], g[j]), j=12..14), i=12..14)

0, (-a-1) y1 y3 y4 + x y4, (-a-1) y2 y3 y4 - x y3, y1 y3 y4 - x y4 + a y1 y3 y4, 0, 0, y2 y3 y4 + a y2 y3 y4 + x y3, 0, 0

(13)

> seq(seq(JB(g[i], g[j]), j=15..16), i=12..14)

0, 0, (a+1) y1 y2 y3 y4 - x (x - y1 y3 - y2 y4), 0, 0, (a+1) y1 y2 y3 y4 - x (x - y1 y3 - y2 y4)

(14)

$$\begin{aligned} &> \text{seq}(\text{seq}(\text{JB}(g[i], g[j]), j = 15 \dots 16), i = 15 \dots 16) \\ &\quad \quad \quad 0, 0, 0, 0 \end{aligned} \quad (15)$$

$$\begin{aligned} &> \text{diff}(y1 \ y2, y2, y1) \\ &\quad \quad \quad -1 \end{aligned} \quad (16)$$

$$\begin{aligned} &> \text{diff}(y1 \ y2 \ y3 \ y4, y4, y3, y2, y1) \\ &\quad \quad \quad 1 \end{aligned} \quad (17)$$

$$\begin{aligned} &> pp := \{y1 \ y3, x \ y1 + b \ y1 \ y2 \ y4, x \ y2 - b \ y1 \ y2 \ y3, x \ y3 + (b + 1) \ y2 \ y3 \ y4, x \ y4 - (b \\ &\quad + 1) \ y1 \ y3 \ y4, x^2 - (y1 \ y3 + y2 \ y4) \ x - (b + 1) \ y1 \ y2 \ y3 \ y4\} : \\ &> DO := f \rightarrow \text{simplify}(\{(1 + b) \ \text{diff}(f, x, x) + 2 \ \text{diff}(f, y4, y3, y2, y1), \text{diff}(f, x, y1, y2), \text{diff}(f, x, \\ &\quad y1, y3) - \text{diff}(f, x, y2, y4), \text{diff}(f, x, y1, y4), \text{diff}(f, x, y2, y3), \text{diff}(f, x, y3, y4), b \ y3 \ \text{diff}(f, \\ &\quad x, y1) + y3 \ \text{diff}(f, y4, y2, y1), b \ y4 \ \text{diff}(f, x, y2) - y4 \ \text{diff}(f, y3, y2, y1), (b + 1) \ \text{diff}(f, x, \\ &\quad y3) + \text{diff}(f, y4, y3, y2), (b + 1) \ \text{diff}(f, x, y4) - \text{diff}(f, y4, y3, y1)\}) : \\ &> \text{map}(DO, pp) \\ &\quad \quad \quad \{\{0\}\} \end{aligned} \quad (18)$$

define odd part of m=g[-]:

$$\begin{aligned} &> v1 := -y1; v2 := y2; v3 := y4; v4 := y3; \\ &\quad \quad \quad v1 := -y1 \\ &\quad \quad \quad v2 := y2 \\ &\quad \quad \quad v3 := y4 \\ &\quad \quad \quad v4 := y3 \end{aligned} \quad (19)$$

define two obvious sl2's

$$\begin{aligned} &> Y1 := 1; X1 := -(x^2 - (y1 \ y3 + y2 \ y4) \ x - (a + 1) \ y1 \ y2 \ y3 \ y4); H1 := \text{JB}(X1, Y1); \\ &\quad Y2 := y1 \ y2; X2 := -y3 \ y4; H2 := \text{JB}(X2, Y2); \\ &\quad \quad \quad Y1 := 1 \\ &\quad \quad \quad X1 := -x^2 + x \ (y1 \ y3 + y2 \ y4) + (a + 1) \ y1 \ y2 \ y3 \ y4 \\ &\quad \quad \quad H1 := 2 \ x - y1 \ y3 - y2 \ y4 \\ &\quad \quad \quad Y2 := y1 \ y2 \\ &\quad \quad \quad X2 := -y3 \ y4 \\ &\quad \quad \quad H2 := y1 \ y3 + y2 \ y4 \end{aligned} \quad (20)$$

$$\begin{aligned} &> \text{simplify}([ \text{JB}(H1, X1) - 2 \ X1, \text{JB}(H1, Y1) + 2 \ Y1, \text{JB}(X1, Y1) - H1 ], \text{simplify}([ \text{JB}(H2, X2) \\ &\quad - 2 \ X2, \text{JB}(H2, Y2) + 2 \ Y2, \text{JB}(X2, Y2) - H2 ])) \\ &\quad \quad \quad [0, 0, 0], [0, 0, 0] \end{aligned} \quad (21)$$

the basis of g0

$$\begin{aligned} &> g1 := x; g2 := y1 \ y3; g3 := y1 \ y4; g4 := y2 \ y3; g5 := y2 \ y4; \\ &\quad \quad \quad g1 := x \\ &\quad \quad \quad g2 := y1 \ y3 \\ &\quad \quad \quad g3 := y1 \ y4 \\ &\quad \quad \quad g4 := y2 \ y3 \\ &\quad \quad \quad g5 := y2 \ y4 \end{aligned} \quad (22)$$

$$\begin{aligned}
&> \text{gen} := b \, g1 + c \, g2 + d \, g3 + e \, g4 + f \, g5; \text{solve}(\{JB(X1, \text{gen}) = 0, JB(X2, \text{gen}) = 0, JB(Y1, \\
&\quad \text{gen}) = 0, JB(Y2, \text{gen}) = 0\}, \{b, c, d, e, f\}); \\
&\quad \text{gen} := b \, x + c \, y1 \, y3 + d \, y1 \, y4 + e \, y2 \, y3 + f \, y2 \, y4 \\
&\quad \{b = 0, c = -f, d = d, e = e, f = f\}
\end{aligned} \tag{23}$$

$$\begin{aligned}
&> H3 := g2 - g5; X3 := g4; Y3 := g3; \\
&\quad H3 := -y2 \, y4 + y1 \, y3 \\
&\quad X3 := y2 \, y3 \\
&\quad Y3 := y1 \, y4
\end{aligned} \tag{24}$$

$$\begin{aligned}
&> JB(H3, X3) - 2 \, X3, JB(H3, Y3) + 2 \, Y3, JB(X3, Y3) - H3 \\
&\quad 0, 0, 0
\end{aligned} \tag{25}$$

$$\begin{aligned}
&> \#` \text{[y3 y4, x y1 + a y1 y2 y4, x y2 - a y1 y2 y3], [x y3 + (a + 1) y2 y3 y4, x y4 - (a} \\
&\quad + 1) y1 y3 y4]}
\end{aligned}$$

bases of odd parts of g[1] and g[2]

$$\begin{aligned}
&> w1 := x \, y4 - (a + 1) \, y1 \, y3 \, y4; w2 := x \, y3 + (a + 1) \, y2 \, y3 \, y4; w3 := -(x \, y1 + a \, y1 \, y2 \, y4); \\
&\quad w4 := (x \, y2 - a \, y1 \, y2 \, y3); \\
&\quad w1 := x \, y4 - (a + 1) \, y1 \, y3 \, y4 \\
&\quad w2 := x \, y3 + (a + 1) \, y2 \, y3 \, y4 \\
&\quad w3 := -x \, y1 - a \, y1 \, y2 \, y4 \\
&\quad w4 := x \, y2 - a \, y1 \, y2 \, y3
\end{aligned} \tag{26}$$

g[-2]: v2 is the highest weight vector, v1 is the lowest:

$$\begin{aligned}
&\quad -y1 \, y3 + y2 \, y4
\end{aligned} \tag{27}$$

$$\begin{aligned}
&> JB(X3, v2), JB(H3, v2) - v2, JB(Y3, v2) - v1, JB(X3, v1) - v2, JB(H3, v1) + v1, JB(Y3, v1); \\
&\quad 0, 0, 0, 0, 0, 0
\end{aligned} \tag{28}$$

g[-1]: v4 is the highest, v3 is the lowest:

$$\begin{aligned}
&> JB(X3, v4), JB(H3, v4) - v4, JB(Y3, v4) - v3, JB(X3, v3) - v4, JB(H3, v3) + v3, JB(Y3, v3); \\
&\quad 0, 0, 0, 0, 0, 0
\end{aligned} \tag{29}$$

g[1]: w4 is the highest, w3 is the lowest

$$\begin{aligned}
&> \text{simplify}([JB(X3, w4), JB(H3, w4) - w4, JB(Y3, w4) - w3]), \text{simplify}([JB(X3, w3) - w4, \\
&\quad JB(H3, w3) + w3, JB(Y3, w3)]); \\
&\quad [0, 0, 0], [0, 0, 0]
\end{aligned} \tag{30}$$

g[2]: w2 is the highest, w1 is the lowest:

$$\begin{aligned}
&> \text{simplify}([JB(X3, w2), JB(H3, w2) - w2, JB(Y3, w2) - w1]), \text{simplify}([JB(X3, w1) - w2, \\
&\quad JB(H3, w1) + w1, JB(Y3, w1)]); \\
&\quad [0, 0, 0], [0, 0, 0]
\end{aligned} \tag{31}$$

recheck the action of X1,Y1,X2,Y2

$$\begin{aligned}
&> \text{simplify}([JB(X1, v1) - w3, JB(X1, v2) - w4, JB(X1, v3) - w1, JB(X1, v4) - w2]); \\
&\quad \text{simplify}([JB(H1, v1) + v1, JB(H1, v2) + v2, JB(H1, v3) + v3, JB(H1, v4) + v4, JB(H1, w1) \\
&\quad - w1, JB(H1, w2) - w2, JB(H1, w3) - w3, JB(H1, w4) - w4]); \\
&\quad \text{simplify}([JB(Y1, w3) - v1, JB(Y1, w4) - v2, JB(Y1, w1) - v3, JB(Y1, w2) - v4]); \\
&\quad [0, 0, 0, 0] \\
&\quad [0, 0, 0, 0, 0, 0, 0, 0]
\end{aligned} \tag{32}$$

$$[0, 0, 0, 0] \quad (32)$$

> *simplify*( $[JB(X2, v1) - v3, JB(X2, v2) - v4, JB(X2, w3) - w1, JB(X2, w4) - w2]$ );  
*simplify*( $[JB(H2, v1) + v1, JB(H2, v2) + v2, JB(H2, v3) - v3, JB(H2, v4) - v4, JB(H2, w1) - w1, JB(H2, w2) - w2, JB(H2, w3) + w3, JB(H2, w4) + w4]$ );  
*simplify*( $[JB(Y2, v3) - v1, JB(Y2, v4) - v2, JB(Y2, w1) - w3, JB(Y2, w2) - w4]$ );

$$[0, 0, 0, 0]$$

$$[0, 0, 0, 0, 0, 0, 0, 0]$$

$$[0, 0, 0, 0] \quad (33)$$

g[-1]xg[-2]: [highest,lowest]= -s1 Y1  
g[-1]xg[-2]: [lowest,highest]= +s1 Y1  
g[-1]xg[+1]: [lowest,lowest]= +s3 Y3  
g[-1]xg[+1]: [highest,highest]= -s3 X3  
g[-1]xg[+2]: [lowest,highest]= +s2 X2  
g[-1]xg[+2]: [highest,lowest]= -s2 X2

>  $s1 := -1; s2 := 1 + a; s3 := -a;$

$$s1 := -1$$

$$s2 := a + 1$$

$$s3 := -a$$

$$(34)$$

> *simplify*( $[JB(v1, v4) + s1 Y1, JB(v2, v3) - s1 Y1, JB(v1, v3), JB(v2, w4)]$ );

$$[0, 0, 0, 0]$$

$$(35)$$

> *simplify* $\left(\left[JB(v3, w3) - s3 Y3, JB(v4, w4) + s3 X3, JB(v3, w4) - \frac{s1}{2} H1 + \frac{s2}{2} H2 - \frac{s3}{2} H3, JB(v4, w3) + \frac{s1}{2} H1 - \frac{s2}{2} H2 - \frac{s3}{2} H3\right]\right);$   
 $JB(v3, w2) - s2 X2, JB(v4, w1) + s2 X2, JB(v3, w1), JB(v4, w2);$

$$[0, 0, 0, 0]$$

$$0, 0, 0, 0$$

$$(36)$$

> *simplify* $\left(\frac{s3}{s1}\right)$

$$a$$

$$(37)$$

>
