# Supplementary material for: Geometric realizations of the Lie superalgebra D(2,1;a)
Source: arXiv:2507.03418 ancillary file (2025-07-04)
Supplement: Supplementary file 4 [file JB_for_p1i.pdf]

In this worksheet we work with G/P<sub>1</sub><sup>I</sup> realization of LSA D(2,1;a)

$$\begin{aligned} &> \text{interface}(\text{warnlevel} = 0) : \text{with}(\text{Physics}) : \text{with}(\text{LinearAlgebra}) : \\ &> \text{Setup}(\text{anticommutativeprefix} = \{\text{seq}(y \parallel i, i = 1 \dots 4)\}, \text{anticommutativecolor} = \text{maroon}) \\ &\quad [\text{anticommutativecolor} = \text{maroon}, \text{anticommutativeprefix} = \{y1, y2, y3, y4\}] \end{aligned} \quad (1)$$

$$\begin{aligned} &> \text{GrassmannParity}(y2 \, y3), \text{GrassmannParity}(y2 \, y3 \, y4) \\ &\quad 0, 1 \end{aligned} \quad (2)$$

$$\begin{aligned} &> \text{diff}(y2 \, y3, y2), \text{diff}(y3 \, y2, y2) \\ &\quad y3, -y3 \end{aligned} \quad (3)$$

The Jacobi-Lagrange bracket

$$\begin{aligned} &> JB := (f, g) \rightarrow \text{simplify} \left( f \, \text{diff}(g, x) - (-1)^{\text{GrassmannParity}(f) \cdot \text{GrassmannParity}(g)} g \, \text{diff}(f, x) \right. \\ &\quad \left. + \frac{(-1)^{\text{GrassmannParity}(f)}}{2} \text{add}((\text{diff}(f, y \parallel i) + (y \parallel i) \, \text{diff}(f, x)) \cdot (\text{diff}(g, y \parallel i) + (y \parallel i) \, \text{diff}(g, x)), i = 1 \dots 4) \right) : \\ &> JB(1, x), JB(1, y1), JB(1, y1 \, y2) \\ &\quad 1, 0, 0 \end{aligned} \quad (4)$$

$$\begin{aligned} &> JB(y1, y1), JB(y1, y2) \\ &\quad -\frac{1}{2}, 0 \end{aligned} \quad (5)$$

$$\begin{aligned} &> JB(x, y1), JB(y1 \, y2, y1), JB(y1 \, y2, y2), JB(y1 \, y2, y3) \\ &\quad -\frac{y1}{2}, \frac{y2}{2}, -\frac{y1}{2}, 0 \end{aligned} \quad (6)$$

$$\begin{aligned} &> JB(y1 \, y2, y1 \, y2), JB(y1 \, y2, y1 \, y3), JB(y1 \, y2, y3 \, y4), JB(x, y1 \, y2) \\ &\quad 0, \frac{y2 \, y3}{2}, 0, 0 \end{aligned} \quad (7)$$

$$\begin{aligned} &> JB(2 \, x, x \, y1 + a \, y2 \, y3 \, y4), JB(2 \, x, x \, y2 - a \, y1 \, y3 \, y4); JB(2 \, y1 \, y2, x \, y1 + a \, y2 \, y3 \, y4), \\ &\quad JB(2 \, y1 \, y3, x \, y1 + a \, y2 \, y3 \, y4), JB(2 \, y2 \, y3, x \, y1 + a \, y2 \, y3 \, y4) \\ &\quad x \, y1 + a \, y2 \, y3 \, y4, x \, y2 - a \, y1 \, y3 \, y4 \\ &\quad x \, y2 - a \, y1 \, y3 \, y4, x \, y3 + a \, y1 \, y2 \, y4, 0 \end{aligned} \quad (8)$$

$$\begin{aligned} &> JB(x \, y1 + a \, y2 \, y3 \, y4, x \, y1 + a \, y2 \, y3 \, y4), JB(x \, y1 + a \, y2 \, y3 \, y4, x \, y2 - a \, y1 \, y3 \, y4) \\ &\quad a \, y1 \, y2 \, y3 \, y4 - \frac{x^2}{2}, 0 \end{aligned} \quad (9)$$

$$\begin{aligned} &> \\ &> SL2a := [y1 \, y2 + y3 \, y4, y1 \, y3 - y2 \, y4, y1 \, y4 + y2 \, y3] : SL2b := [y1 \, y2 - y3 \, y4, y1 \, y3 \\ &\quad + y2 \, y4, y1 \, y4 - y2 \, y3] : SL2c := [-2 \, x, 1, x^2 - 2 \, a \, y1 \, y2 \, y3 \, y4] : \text{map}(JB, SL2a, SL2b), \\ &\quad \text{map}(JB, SL2a, SL2c), \text{map}(JB, SL2b, SL2c) \\ &\quad [[0, 0, 0], [0, 0, 0], [0, 0, 0]], [[0, 0, 0], [0, 0, 0], [0, 0, 0]], [[0, 0, 0], [0, 0, 0], [0, 0, 0]] \end{aligned} \quad (10)$$

$$\begin{aligned} &> JB(SL2a[1], SL2a[2]) - SL2a[3], JB(SL2a[1], SL2a[3]) + SL2a[2] \\ &\quad 0, 0 \end{aligned} \quad (11)$$

$$\begin{aligned} &> SL2a := [2 \, I \, (y1 \, y2 + y3 \, y4), (y1 \, y3 - y2 \, y4) + I \, (y1 \, y4 + y2 \, y3), (y1 \, y3 - y2 \, y4) - I \, (y1 \, y4 \end{aligned}$$

$$+ y_2 y_3)] : SL2b := [2 I (y_1 y_2 - y_3 y_4), (y_1 y_3 + y_2 y_4) - I (y_1 y_4 - y_2 y_3), (y_1 y_3 + y_2 y_4) + I (y_1 y_4 - y_2 y_3)] :$$

$$\begin{aligned} &> \text{simplify}(JB(SL2a[1], SL2a[2]) - 2 SL2a[2]), \text{simplify}(JB(SL2a[1], SL2a[3]) \\ &\quad + 2 SL2a[3]), \text{simplify}(JB(SL2a[3], SL2a[2]) - SL2a[1]), \\ &\text{simplify}(JB(SL2b[1], SL2b[2]) - 2 SL2b[2]), \text{simplify}(JB(SL2b[1], SL2b[3]) \\ &\quad + 2 SL2b[3]), \text{simplify}(JB(SL2b[3], SL2b[2]) - SL2b[1]), \\ &\text{simplify}(JB(SL2c[1], SL2c[2]) - 2 SL2c[2]), \text{simplify}(JB(SL2c[1], SL2c[3]) + 2 SL2c[3]), \\ &\text{simplify}(JB(SL2c[3], SL2c[2]) - SL2c[1]) \\ &\quad 0, 0, 0, 0, 0, 0, 0, 0, 0 \end{aligned} \quad (12)$$

$$\begin{aligned} &> C2C2a := [y_1, y_2, y_3, y_4] : C2C2b := [x y_1 + a y_2 y_3 y_4, x y_2 - a y_1 y_3 y_4, x y_3 + a y_1 y_2 y_4, \\ &\quad x y_4 - a y_1 y_2 y_3] : \\ &> \text{solve}(\{ \text{Coefficients}(\text{map}(JB, SL2a[3], \text{add}(z[i] C2C2a[i], i = 1 \dots \text{nops}(C2C2a))))), \{y_1, y_2, y_3, \\ &\quad y_4\} \} \text{ union } \{ \text{Coefficients}(\text{map}(JB, SL2b[3], \text{add}(z[i] C2C2a[i], i = 1 \dots \text{nops}(C2C2a))))), \\ &\quad \{y_1, y_2, y_3, y_4\} \} \} ); \\ &\text{solve}(\{ \text{Coefficients}(\text{map}(JB, SL2a[3], \text{add}(z[i] C2C2b[i], i = 1 \dots \text{nops}(C2C2b))))), \{y_1, y_2, y_3, \\ &\quad y_4\} \} \text{ union } \{ \text{Coefficients}(\text{map}(JB, SL2b[3], \text{add}(z[i] C2C2b[i], i = 1 \dots \text{nops}(C2C2b))))), \\ &\quad \{y_1, y_2, y_3, y_4\} \} \} ); \\ &\text{solve}(\{ \text{Coefficients}(\text{map}(JB, SL2a[2], \text{add}(z[i] C2C2a[i], i = 1 \dots \text{nops}(C2C2a))))), \{y_1, y_2, y_3, \\ &\quad y_4\} \} \text{ union } \{ \text{Coefficients}(\text{map}(JB, SL2b[2], \text{add}(z[i] C2C2a[i], i = 1 \dots \text{nops}(C2C2a))))), \\ &\quad \{y_1, y_2, y_3, y_4\} \} \} ); \\ &\text{solve}(\{ \text{Coefficients}(\text{map}(JB, SL2a[2], \text{add}(z[i] C2C2b[i], i = 1 \dots \text{nops}(C2C2b))))), \{y_1, y_2, y_3, \\ &\quad y_4\} \} \text{ union } \{ \text{Coefficients}(\text{map}(JB, SL2b[2], \text{add}(z[i] C2C2b[i], i = 1 \dots \text{nops}(C2C2b))))), \\ &\quad \{y_1, y_2, y_3, y_4\} \} \} ); \\ &\quad \{z_1 = I z_2, z_2 = z_2, z_3 = 0, z_4 = 0\} \\ &\quad \{z_1 = z_1, z_2 = -I z_1, z_3 = 0, z_4 = 0\} \\ &\quad \{z_1 = -I z_2, z_2 = z_2, z_3 = 0, z_4 = 0\} \\ &\quad \{z_1 = z_1, z_2 = I z_1, z_3 = 0, z_4 = 0\} \end{aligned} \quad (13)$$

$$\begin{aligned} &> LWm1 := I y_1 + y_2; LWp1 := (x y_1 + a y_2 y_3 y_4) - I (x y_2 - a y_1 y_3 y_4); \\ &\quad HWm1 := -I y_1 + y_2; HWp1 := I \cdot (x y_1 + a y_2 y_3 y_4) - (x y_2 - a y_1 y_3 y_4); \\ &\quad LWm1 := y_2 + I y_1 \\ &\quad LWp1 := x y_1 + a y_2 y_3 y_4 - I (x y_2 - a y_1 y_3 y_4) \\ &\quad HWm1 := y_2 - I y_1 \\ &\quad HWp1 := I (x y_1 + a y_2 y_3 y_4) - x y_2 + a y_1 y_3 y_4 \end{aligned} \quad (14)$$

2 sl2 in g0

$$\begin{aligned} &> ha := 2 I (y_1 y_2 + y_3 y_4); \\ &\quad xa := -(y_1 y_3 - y_2 y_4 + I (y_1 y_4 + y_2 y_3)); \\ &\quad ya := (y_1 y_3 - y_2 y_4 - I (y_1 y_4 + y_2 y_3)); \\ &\quad ha := 2 I (y_1 y_2 + y_3 y_4) \\ &\quad xa := -y_1 y_3 + y_2 y_4 - I (y_1 y_4 + y_2 y_3) \\ &\quad ya := y_1 y_3 - y_2 y_4 - I (y_1 y_4 + y_2 y_3) \end{aligned} \quad (15)$$

$$\begin{aligned} &> \text{simplify}([JB(xa, ya) - ha, JB(ha, xa) - 2 xa, JB(ha, ya) + 2 ya]) \\ &\quad [0, 0, 0] \end{aligned} \quad (16)$$

$$\begin{aligned}
&> hb := 2 I (y1 y2 - y3 y4); \\
&xb := (y1 y3 + y2 y4 - I (y1 y4 - y2 y3)); \\
&yb := -(y1 y3 + y2 y4 + I (y1 y4 - y2 y3)); \\
&\quad hb := 2 I (y1 y2 - y3 y4) \\
&\quad xb := y1 y3 + y2 y4 - I (y1 y4 - y2 y3) \\
&\quad yb := -y1 y3 - y2 y4 - I (y1 y4 - y2 y3)
\end{aligned} \tag{17}$$

$$\begin{aligned}
&> simplify([JB(xb, yb) - hb, JB(hb, xb) - 2 xb, JB(hb, yb) + 2 yb]); \\
&\quad [0, 0, 0]
\end{aligned} \tag{18}$$

g1

$$\begin{aligned}
&> f4 := -HWp1; f3 := JB(ya, f4); f2 := JB(yb, f4); f1 := JB(ya, f2); f5 := \frac{1}{s1} JB(f1, f4); \\
&\quad f4 := -I (x y1 + a y2 y3 y4) + x y2 - a y1 y3 y4 \\
&\quad f3 := a y1 y2 y3 - I a y1 y2 y4 - (y4 + I y3) x \\
&\quad f2 := a y1 y2 y3 + I a y1 y2 y4 + x (-y4 + I y3) \\
&\quad f1 := a y1 y3 y4 - I a y2 y3 y4 - x (y2 + I y1) \\
&\quad f5 := \frac{x^2 - 2 a y1 y2 y3 y4}{s1}
\end{aligned} \tag{19}$$

check relations

$$\begin{aligned}
&> simplify([JB(f1, f4) - s1 f5, JB(f2, f3) + s1 f5, JB(f2, f4), JB(f3, f4), JB(f1, f2), JB(f1, f1), \\
&\quad JB(f1, f2)]) \\
&\quad [0, 0, 0, 0, 0, 0, 0]
\end{aligned} \tag{20}$$

$$\begin{aligned}
&> hc := 2 x; yc := -2; xc := \frac{x^2}{2} - a y1 y2 y3 y4 \\
&\quad hc := 2 x \\
&\quad yc := -2 \\
&\quad xc := -a y1 y2 y3 y4 + \frac{x^2}{2}
\end{aligned} \tag{21}$$

$$\begin{aligned}
&> simplify([JB(xc, yc) - hc, JB(hc, xc) - 2 xc, JB(hc, yc) + 2 yc]) \\
&\quad [0, 0, 0]
\end{aligned} \tag{22}$$

$$\begin{aligned}
&> e1 := -HWm1; e3 := JB(yb, e1); e2 := JB(ya, e1); e4 := JB(yb, e2); e5 := -\frac{1}{s1}; \\
&\quad e1 := -y2 + I y1 \\
&\quad e3 := y4 - I y3 \\
&\quad e2 := y4 + I y3 \\
&\quad e4 := y2 + I y1 \\
&\quad e5 := -\frac{1}{s1}
\end{aligned} \tag{23}$$

these match the equations for the negative part m

$$\begin{aligned}
&> [JB(e2, e2), JB(e3, e3), JB(e4, e4), JB(e1, e2), JB(e1, e3), JB(e1, e4) + s1 e5, JB(e2, e3) \\
&\quad - s1 e5, JB(e2, e4), JB(e3, e4), JB(e1, e2), JB(e1, e1), JB(e1, e2)]
\end{aligned} \tag{24}$$

$$[0, 0, 0, 0, 0, 0, 0, 0, 0, 0, 0, 0, 0] \quad (24)$$

$$\begin{aligned} & \text{> } s1 := 1; s2 := -\frac{1+a}{2}; s3 := -\frac{1-a}{2}; \\ & \text{simplify}(s3/s2) \end{aligned}$$

$$\begin{aligned} s1 &:= 1 \\ s2 &:= -\frac{1}{2} - \frac{a}{2} \\ s3 &:= -\frac{1}{2} + \frac{a}{2} \\ & \frac{1-a}{1+a} \end{aligned} \quad (25)$$

$$\begin{aligned} & \text{> } \text{simplify}\left(JB(e1, f1) + \frac{1}{2} hc - \left(-\frac{1+a}{4} ha - \frac{1-a}{4} hb\right)\right), \\ & \text{simplify}\left(JB(e1, f1) - \left(\frac{s2}{2} ha + \frac{s3}{2} hb - \frac{s1}{2} hc\right)\right), \\ & \text{simplify}\left(JB(e2, f2) - \left(\frac{s2}{2} ha - \frac{s3}{2} hb + \frac{s1}{2} hc\right)\right), \\ & \text{simplify}\left(JB(e3, f3) - \left(-\frac{s2}{2} ha + \frac{s3}{2} hb + \frac{s1}{2} hc\right)\right), \\ & \text{simplify}\left(JB(e4, f4) - \left(-\frac{s2}{2} ha - \frac{s3}{2} hb - \frac{s1}{2} hc\right)\right) \\ & \quad 0, 0, 0, 0, 0 \end{aligned} \quad (26)$$

$$\begin{aligned} & \text{> } \text{simplify}([JB(e1, f2) + s2 xa, JB(e1, f3) + s3 xb, JB(e1, f4), JB(e2, f3), JB(e2, f4) - s3 xb, \\ & \quad JB(e3, f4) - s2 xa]) \\ & \quad [0, 0, 0, 0, 0, 0] \end{aligned} \quad (27)$$
