# Supplementary material for: Geometric realizations of the Lie superalgebra D(2,1;a)
Source: arXiv:2507.03418 ancillary file (2025-07-04)
Supplement: Supplementary file 5 [file JB_for_p1ip12i.pdf]

> *interface*(warnlevel = 0) : *with*(Physics) : *with*(LinearAlgebra) :  
 > *Setup*(anticommutativeprefix = {seq( $\xi \parallel i, i = 1..4$ ), seq( $\theta \parallel i, i = 1..2$ ), seq( $v \parallel i, i = 1..2$ )},  
 anticommutativecolor = maroon)  
 [anticommutativecolor = maroon, anticommutativeprefix = {v1, v2,  $\theta 1$ ,  $\theta 2$ ,  $\xi 1$ ,  $\xi 2$ ,  $\xi 3$ ,  $\xi 4$ }] (1)

> *sbs* :=  $\left\{ x = y - \frac{1}{2} (\theta 1 v1 + \theta 2 v2), \xi 1 = \frac{1}{2} (\theta 1 + v1), \xi 2 = \frac{1}{2 I} (\theta 1 - v1), \xi 3 = \frac{1}{2} (\theta 2 + v2), \xi 4 = \frac{1}{2 I} (\theta 2 - v2) \right\}$ :

> *tmp* := *simplify*(*eval*([ $\xi 1 \xi 2, \xi 1 \xi 3, \xi 1 \xi 4, \xi 2 \xi 3, \xi 2 \xi 4, \xi 3 \xi 4$ ], *sbs*))  
*tmp* :=  $\left[ -\frac{1}{2} v1 \theta 1, \frac{\theta 1 \theta 2}{4} - \frac{v2 \theta 1}{4} + \frac{v1 \theta 2}{4} + \frac{v1 v2}{4}, -\frac{1}{2} \left( \frac{\theta 1}{2} + \frac{v1}{2} \right) (\theta 2 - v2), \right.$   
 $\left. -\frac{1}{2} (\theta 1 - v1) \left( \frac{\theta 2}{2} + \frac{v2}{2} \right), -\frac{(\theta 1 - v1) (\theta 2 - v2)}{4}, -\frac{1}{2} v2 \theta 2 \right]$  (2)

> *simplify*({2 *I tmp*[1], *tmp*[2] + *I tmp*[3] + *I tmp*[4] - *tmp*[5], *tmp*[2] + *I tmp*[3] - *I tmp*[4] + *tmp*[5],  
 -*tmp*[2] + *I tmp*[3] - *I tmp*[4] - *tmp*[5], *tmp*[2] - *I tmp*[3] - *I tmp*[4] - *tmp*[5], 2 *I tmp*[6]})  
 {v1 v2, v1  $\theta 1$ , v1  $\theta 2$ , v2  $\theta 1$ , v2  $\theta 2$ ,  $\theta 1 \theta 2$ } (3)

> *simplify*(*expand*(*eval*( $x \xi 1 + \varepsilon \xi 2 \xi 3 \xi 4$ , *sbs*))), *simplify*(*expand*(*eval*( $x \xi 2 - \varepsilon \xi 1 \xi 3 \xi 4$ ,  
*sbs*)))  
 $\frac{(\varepsilon - 1) v2 \theta 1 \theta 2}{4} + \frac{(\varepsilon + 1) v1 v2 \theta 2}{4} + \frac{y (\theta 1 + v1)}{2}, \frac{1}{4} (2 y v1 - 2 y \theta 1 + \varepsilon v1 v2 \theta 2$   
 $- \varepsilon v2 \theta 1 \theta 2 + v1 v2 \theta 2 + v2 \theta 1 \theta 2)$  (4)

> *simplify*(*expand*(*eval*( $I (x \xi 4 - \varepsilon \xi 1 \xi 2 \xi 3)$ , *sbs*)))  
 $\frac{(1 - \varepsilon) v1 \theta 1 \theta 2}{4} + \frac{(\varepsilon + 1) v1 v2 \theta 1}{4} - \frac{y (v2 - \theta 2)}{2}$  (5)

> *simplify*(*expand*(*eval*( $x \xi 1 + \varepsilon \xi 2 \xi 3 \xi 4 + I (x \xi 2 - \varepsilon \xi 1 \xi 3 \xi 4)$ , *sbs*))),  
*simplify*(*expand*(*eval*( $x \xi 1 + \varepsilon \xi 2 \xi 3 \xi 4 - I (x \xi 2 - \varepsilon \xi 1 \xi 3 \xi 4)$ , *sbs*))),  
*simplify*(*expand*(*eval*( $x \xi 3 + \varepsilon \xi 1 \xi 2 \xi 4 + I (x \xi 4 - \varepsilon \xi 1 \xi 2 \xi 3)$ , *sbs*))),  
*simplify*(*expand*(*eval*( $x \xi 3 + \varepsilon \xi 1 \xi 2 \xi 4 - I (x \xi 4 - \varepsilon \xi 1 \xi 2 \xi 3)$ , *sbs*)))  
 $\frac{(\varepsilon - 1) v2 \theta 1 \theta 2}{2} + y \theta 1, \frac{(\varepsilon + 1) v1 v2 \theta 2}{2} + y v1$   
 $\frac{(1 - \varepsilon) v1 \theta 1 \theta 2}{2} + y \theta 2, \frac{(-1 - \varepsilon) v1 v2 \theta 1}{2} + y v2$  (6)

> *JB* := (*f*, *g*) → *simplify*(*f diff*(*g*, *y*) - (-1)<sup>GrassmannParity(*f*) · GrassmannParity(*g*)</sup> *g diff*(*f*, *y*) + (-1)<sup>GrassmannParity(*f*)</sup> *add*((*diff*(*f*,  $\theta \parallel i$ ) + ( $v \parallel i$ ) *diff*(*f*, *y*)) · (*diff*(*g*,  $v \parallel i$ )) + (*diff*(*f*,  $v \parallel i$ )) · (*diff*(*g*,  $\theta \parallel i$ ) + ( $v \parallel i$ ) *diff*(*g*, *y*)), *i* = 1..2)) :  
 > *JB*(3 *y* -  $\theta 1 v1$  -  $\theta 2 v2$ , 1), *JB*(3 *y* -  $\theta 1 v1$  -  $\theta 2 v2$ ,  $\theta 1$ ), *JB*(3 *y* -  $\theta 1 v1$  -  $\theta 2 v2$ ,  $\theta 2$ );  
*JB*(3 *y* -  $\theta 1 v1$  -  $\theta 2 v2$ ,  $\theta 1 \theta 2$ ), *JB*(3 *y* -  $\theta 1 v1$  -  $\theta 2 v2$ , *v1*), *JB*(3 *y* -  $\theta 1 v1$  -  $\theta 2 v2$ , *v2*)  
 -3, -2  $\theta 1$ , -2  $\theta 2$  (7)

$$-\theta_1 \theta_2, -v_1, -v_2 \quad (7)$$

$$> JB(y, \theta_1 \theta_2), JB(y, v_1 v_2)$$

$$-\theta_1 \theta_2, v_1 v_2 \quad (8)$$

$$> JB(y, \theta_1 v_1), JB(y, \theta_1 v_2), JB(y, \theta_2 v_1), JB(y, \theta_2 v_2), JB(\theta_1 v_1 + \theta_2 v_2, \theta_1 v_1), JB(\theta_1 v_1 + \theta_2 v_2, \theta_1 v_2), JB(\theta_1 v_1 + \theta_2 v_2, \theta_2 v_1), JB(\theta_1 v_1 + \theta_2 v_2, \theta_2 v_2)$$

$$0, 0, 0, 0, 0, 0, 0, 0 \quad (9)$$

$$> JB(2y - \theta_1 v_1 - \theta_2 v_2, \theta_1 \theta_2), JB(2y - \theta_1 v_1 - \theta_2 v_2, \theta_1 v_1), JB(2y - \theta_1 v_1 - \theta_2 v_2, \theta_1 v_2), JB(2y - \theta_1 v_1 - \theta_2 v_2, \theta_2 v_1), JB(2y - \theta_1 v_1 - \theta_2 v_2, \theta_2 v_2), JB(2y - \theta_1 v_1 - \theta_2 v_2, v_1 v_2)$$

$$0, 0, 0, 0, 0, 0 \quad (10)$$

$$> JB(2y - \theta_1 v_1 - \theta_2 v_2, 1), JB(2y - \theta_1 v_1 - \theta_2 v_2, \theta_1), JB(2y - \theta_1 v_1 - \theta_2 v_2, \theta_2), JB(2y - \theta_1 v_1 - \theta_2 v_2, v_1), JB(2y - \theta_1 v_1 - \theta_2 v_2, v_2)$$

$$-2, -\theta_1, -\theta_2, -v_1, -v_2 \quad (11)$$

>
