# Supplementary material for: Geometric realizations of the Lie superalgebra D(2,1;a)
Source: arXiv:2507.03418 ancillary file (2025-07-04)
Supplement: Supplementary file 6 [file StrEq_p123iv.pdf]

```
[> restart;
```

Packages needed:

- DifferentialGeometry
- Tensor
- Tools
- LinearAlgebra

In later versions of LSA package, it will work without needing to load those packages beforehand

```
> with(DifferentialGeometry): with(Tensor): with(Tools): with  
(LinearAlgebra):
```

Read the LSA code file:

```
> read("/home/anna/Escriptori/PHD/maple andreu/LSA_v1.2.7.mpl")
```

If the file is in the same folder as the current Maple worksheet, the name of the file is enough. Otherwise, the full path is needed.

Load the LSA package:

```
> with(LieSuperAlgebras)
```

```
[ `', BasisElement, ChangeOfBasis, ChangeOfScaling, DimensionOfTanakaSuperProlongation, (1)  
LieSuperAlgebra, StructureRelations, TanakaSuperProlongation, array, basis, bracket,  
changeNames, const, decompose, display, extendLieSuperAlgebra, form, get_str_from_borel,  
graded_root_table, grading, jacobi, list_is_symmetric, parity, reduced_g0_dimension,  
root_table, struc, symbol_algebra, tensor, vector ]
```

In order to set up an object of type LieSuperAlgebra, we need

- names for basis elements
- structure relations
- parity
- grading

The names and the parity can be given by a list that contains 2 lists: even basis elements and odd basis elements

```
> SHCbasis:= [ [X1,H1,Y1,X2,H2,Y2,X3,H3,Y3] , [xxx, xxy, xyx, yxx, xyy, yxy ,  
yyx,yyy] ]  
SHCbasis := [ [X1, H1, Y1, X2, H2, Y2, X3, H3, Y3], [xxx, xxy, xyx, yxx, xyy, yxy, yyx, yyy]] (2)
```

The structure relations can be given by a list, similarly to the LieAlgebras package.

```
> SHCstr:=[  
[H1,X1]=2*X1, [H2,X2]=2*X2, [H3,X3]=2*X3, [X1,Y1]=H1, [X2,Y2]=H2, [X3,  
Y3]=H3, [H1,Y1]=-2*Y1, [H2,Y2]=-2*Y2, [H3,Y3]=-2*Y3,  
[X1,yxx]=xxx, [X1,yxy]=xxy, [X1,yyx]=xyx, [X1,yyy]=xyy,  
[X2,xyx]=xxx, [X2,xyy]=xxy, [X2,yyx]=yxx, [X2,yyy]=yxy,  
[X3,xyx]=xxx, [X3,xyy]=xyx, [X3,yxy]=yxx, [X3,yyy]=yyx,  
[Y1,xxx]=yxx, [Y1,xxy]=yxy, [Y1,xyx]=yyx, [Y1,xyy]=yyy,  
[Y2,xxx]=xyx, [Y2,xxy]=xyy, [Y2,yxx]=yyx, [Y2,yxy]=yyy,  
[Y3,xxx]=xxy, [Y3,xyx]=xyy, [Y3,yxx]=yxy, [Y3,yyx]=yyy,  
[H1,xxx]=xxx, [H1,xxy]=xxy, [H1,xyx]=xyx, [H1,yxx]=-yxx, [H1,xyy]=xyy,  
[H1,yxy]=-yxy, [H1,yyx]=-yyx, [H1,yyy]=-yyy,
```

```

[H2,xxx]=xxx,[H2,xy]=xxy,[H2,xyx]=-xyx,[H2,yxx]=yxx,[H2,xyy]=-xyy,
[H2,yxy]=yxy,[H2,yyx]=-yyx,[H2,yyy]=-yyy,
[H3,xxx]=xxx,[H3,xy]=-xxy,[H3,xyx]=xyx,[H3,yxx]=yxx,[H3,xyy]=-xyy,
[H3,yxy]=-yxy,[H3,yyx]=yyx,[H3,yyy]=-yyy,
[xxx,yx]=s3*X3,[xxx,yxy]=s2*X2,[xxx,xy]=s1*X1,[xxx,yyy]=-s1/2*H1-
s2/2*H2-s3/2*H3,
[xxy,xyx]=-s1*X1,[xxy,yxx]=-s2*X2,[xxy,yyy]=-s3*Y3,[xxy,yyx]=s1/2*
H1+s2/2*H2-s3/2*H3,
[xyx,xxy]=-s1*X1,[xyx,yyy]=-s2*Y2,[xyx,yxx]=-s3*X3,[xyx,yxy]=s1/2*
H1-s2/2*H2+s3/2*H3,
[yxx,yyy]=-s1*Y1,[yxx,xxy]=-s2*X2,[yxx,xyx]=-s3*X3,[yxx,xyy]=-s1/2*
H1+s2/2*H2+s3/2*H3,
[xyy,xxx]=s1*X1,[xyy,yyx]=s2*Y2,[xyy,yxy]=s3*Y3,[xyy,yxx]=-s1/2*H1+
s2/2*H2+s3/2*H3,
[yxy,yyx]=s1*Y1,[yxy,xxx]=s2*X2,[yxy,xyy]=s3*Y3,[yxy,xyx]=s1/2*H1-
s2/2*H2+s3/2*H3,
[yyx,yxy]=s1*Y1,[yyy,xyx]=-s2*Y2,[yyx,xxx]=s3*X3,[yyx,xxy]=s1/2*H1+
s2/2*H2-s3/2*H3
]:

```

```

> SHCgrad:= [-2,0,2,0,0,0,0,0,0,0,1,1,1,-1,1,-1,-1,-1]
      SHCgrad := [-2,0,2,0,0,0,0,0,0,0,1,1,1,-1,1,-1,-1,-1] (3)

```

The grading can be given by a list, where the i-th grading in the list corresponds to the i-th element in the basis. consider the grading pl1

The command LieSuperAlgebra defines an object of type LieSuperAlgebra.

```

> SHCm:= LieSuperAlgebra(SHCstr, SHCbasis, SHCgrad);
      SHCm := Lie superalgebra: Alg (4)

```

```

> %SHCm.struc.jacobi
      SHCm • struc • jacobi (5)

```

```

> base_names:=[op(SHCbasis[1]),op(SHCbasis[2])];
      base_names := [X1, H1, Y1, X2, H2, Y2, X3, H3, Y3, xxx, xxy, xyx, yxx, xyy, yxy, yyx, yyy] (6)

```

```

> base_names_2:=[seq(E||i,i=1..17)];
      base_names_2 := [E1, E2, E3, E4, E5, E6, E7, E8, E9, E10, E11, E12, E13, E14, E15, E16, E17] (7)

```

```

> [seq(changeNames(E||j,base_names_2,base_names),j=1..17)];
      [X1, H1, Y1, X2, H2, Y2, X3, H3, Y3, xxx, xxy, xyx, yxx, xyy, yxy, yyx, yyy] (8)

```

```

> changeNames(E10,base_names_2,base_names);
      xxx (9)

```

```

> superbracket:=(x,y)->SHCm.bracket(changeNames(x,base_names,
      base_names_2),changeNames(y,base_names,base_names_2));
superbracket := (x,y) → LieSuperAlgebras:-`(SHCm, LieSuperAlgebras:-
      bracket(LieSuperAlgebras:-changeNames(x,base_names,base_names_2),
      LieSuperAlgebras:-changeNames(y,base_names,base_names_2))) (10)

```

[e1,e2]=s3e6,[e1,e3]=s2e5,[e2,e3]=s1e4,[e1,e4]=-e7,[e2,e5]=-e7 and

$$[e_3, e_6] = -e_7$$

```
> e1:=xyy; e2:=yxy; e3:=yyx;
e4:=Y1; e5:=Y2; e6:=Y3;
e7:=yyy;
```

$e1 := xyy$   
 $e2 := yxy$   
 $e3 := yyx$   
 $e4 := Y1$   
 $e5 := Y2$   
 $e6 := Y3$   
 $e7 := yyy$

(11)

```
> superbracket(e1,e2);
superbracket(e1,e3);
superbracket(e2,e3);
```

$s3 E9$   
 $s2 E6$   
 $s1 E3$

(12)

$$[v_1, v_2] = v_6, [v_1, v_3] = v_5, [v_2, v_3] = v_4, [v_1, v_4] = (s_2 - s_3) v_7, [v_2, v_5] = (s_3 - s_1) v_7 \text{ and } [v_3, v_6] = (s_1 - s_2) v_7$$

```
> v1:=e2-e3;
v2:=e3-e1;
v3:=e2-e1;
```

$v1 := yxy - yyx$   
 $v2 := -xyy + yyx$   
 $v3 := -xyy + yxy$

(13)

```
> v23:=superbracket(v2,v3);
v13:=superbracket(v1,v3);
v12:=superbracket(v1,v2);
```

$v23 := s1 E3 - s2 E6 - s3 E9$   
 $v13 := -s1 E3 + s2 E6 - s3 E9$   
 $v12 := s1 E3 + s2 E6 - s3 E9$

(14)

```
> superbracket(v1,v23);
superbracket(v2,v13);
superbracket(v3,v12);
```

$(-s3 + s2) E17$   
 $-(-s3 + s1) E17$   
 $(-s2 + s1) E17$

(15)
